# Supplementary material for: Are All Losses Created Equal: A Neural Collapse Perspective
Source: arXiv:2210.02192 source file (2022-10-08)
Supplement: Supplementary file 5 [file thm_global-ls.tex]

In this part of appendices, we prove \Cref{thm:global-minima-ls} in \Cref{sec:main} that we restate as follows.

\begin{theorem}[Global Optimality Condition of LS]\label{thm:global-minima-app-ls}
	Assume that the number of classes $K$ is smaller than feature dimension $d$, i.e., $K< d$, and the dataset is balanced for each class, $n=n_1=\cdots=n_K$. Then any global minimizer $(\mW^\star, \mH^\star,\vb^\star)$ of 
	\begin{align}\label{eq:obj-app-ls}
     \min_{\mb W , \mb H,\mb b  } \; f(\mb W,\mb H,\mb b) \;:=\; g(\mW\mH + \vb\vone^\top) \;+\; \frac{\lambda_{\mb W} }{2} \norm{\mb W}{F}^2 + \frac{\lambda_{\mb H} }{2} \norm{\mb H}{F}^2 + \frac{\lambda_{\mb b} }{2} \norm{\mb b}{2}^2
\end{align}
with 
\begin{align}\label{eqn:g-lls-app}
    &g(\mW\mH + \vb\vone^\top) := \frac{1}{N}\sum_{k=1}^K\sum_{i=1}^n \Lls (\mW\vh_{k,i} + \vb,\vy_k, \alpha);\\
    &\Lls (\vz,\vy_k,\alpha) :=\sum_{m=1}^K\paren{\paren{1-\alpha}y_{k,m}+\frac{\alpha}{K}}\log\paren{\sum_{j=1}^K \exp(z_j-z_k)}.
\end{align}
obeys the following 
\begin{align*}
    & \norm{\mb w^\star}{2}\;=\; \norm{\mb w^{\star 1} }{2} \;=\; \norm{\mb w^{\star 2}}{2} \;=\; \cdots \;=\; \norm{\mb w^{\star K} }{2}, \quad \text{and}\quad \mb b^\star = b^\star \mb 1, \\ 
    & \vh_{k,i}^\star \;=\;  \sqrt{ \frac{ \lambda_{\mb W}  }{ \lambda_{\mb H} n } } \vw^{\star k} ,\quad \forall \; k\in[K],\; i\in[n],  \quad \text{and} \quad  \ol{\mb h}_{i}^\star \;:=\; \frac{1}{K} \sum_{j=1}^K \mb h_{j,i}^\star \;=\; \mb 0, \quad \forall \; i \in [n],
\end{align*}
where either $b^\star = 0$ or $\lambdab=0$, and the matrix $\frac{1}{\norm{\mb w^\star}{2}}  \mW^{\star\top} $ is in the form of $K$-simplex ETF structure defined in Definition \ref{def:simplex-ETF} in the sense that 
\begin{align*}
    \frac{1}{\norm{\mb w^\star}{2}^2}  \mW^{\star\top} \mW^{\star}\;=\; \frac{K}{K-1}  \paren{ \mb I_K - \frac{1}{K} \mb 1_K \mb 1_K^\top }.
\end{align*}
\end{theorem}

\subsection{Main Proof}

Similar to the proofs in \cite{lu2020neural,fang2021layer}, we prove the theorem by directly showing that $f(\mW,\mH,\vb)> f(\mW^\star,\mH^\star,\vb^\star)$ for any $(\mW,\mH, \vb)$ not in the form as shown in \Cref{thm:global-minima-app-ls}.

\vspace{0.1in}

\begin{proof}[Proof of \Cref{thm:global-minima-app-ls}] 
First note that the objective function $f$ is \emph{coercive}\footnote{A function $f:\bb R^n \mapsto \bb R$ is coercive if $f(\mb x) \rightarrow +\infty$ as $\norm{\mb x}{2} \rightarrow +\infty $.}  due to the weight decay regularizers and the fact that the label smooth loss $\Lls (\vz,\vy_k,\alpha)$ is always non-negative. %\js{I don't think so: if data is separable, the minimizer diverges as $g\to 0$. $f$ is coercive because the regularizers ($\|\cdot\|_F$) are coercive.} \zz{Correct and add the weight decay regularizers.}. 
This implies that the global minimizer of $f(\mb W,\mb H,\mb b)$ in \eqref{eq:obj-app-ls} is always finite. By Lemma \ref{lem:critical-balance-ls}, we know that any critical point $(\mb W,\mb H,\mb b)$ of $f$ in \eqref{eq:obj-app-ls} satisfies 
\begin{align*}
    \mW^\top\mW = \frac{\lambda_{\mH}}{\lambda_{\mW}}\mH\mH^\top. 
\end{align*}
For the rest of the proof, to simplify the notations, let $\norm{\mW}{F}^2 = \rho$, and thus $\norm{\mH}{F}^2 = \frac{\lambda_{\mH}}{\lambda_{\mW}}\rho$. 

%\paragraph{The global solutions can be attained by the $K$-Simplex ETF.} 
We will first provide a lower bound for the label-smoothing term $g(\mW\mH + \vb\vone^\top)$ for any $\mW$ with energy $\rho$, and then show that the lower bound is attained if and only if the parameters are in the form described in \Cref{thm:global-minima-app-ls}. Now, by Lemma \ref{lem:lower-bound-g-ls}, we know that for any $c_1,c_3 >0$,
\begin{align*}
   g(\mb W \mb H + \mb b \mb 1^\top) \;\geq\; - \frac{\rho c_2}{(1+c_4)(K-1)} \sqrt{ \frac{ \lambda_{\mb W}  }{ \lambda_{\mb H} n } } \;+\; c_5
\end{align*}
with $c_2 = 1-\frac{\alpha(K-1)(1+c_1)}{K}$, $c_3 = \paren{c_1\log c_1 -(c_1+1)\log(c_1 + 1)} + \frac{\alpha(K-1)}{K}\log\paren{K-1}$ and $c_5 = \frac{c_2}{1+c_4} \log\paren{ (1+c_4)(K-1) } + \frac{c_2c_4}{1+c_4} \log\paren{ \frac{1+c_4}{c_4} } -c_3 $. Therefore, we have
\begin{align*}
    f(\mb W,\mb H,\mb b)\;&=\;  g(\mb W \mb H + \mb b \mb 1^\top) \;+\; \frac{\lambda_{\mb W} }{2} \norm{\mb W}{F}^2 + \frac{\lambda_{\mb H} }{2} \norm{\mb H}{F}^2 + \frac{\lambda_{\mb b} }{2} \norm{\mb b}{2}^2 \\
%    \;&\geq\; \underbrace{ - \frac{ \rho }{ (1+c_1)(K-1) } \sqrt{ \frac{ \lambda_{\mb W} }{ \lambda_{\mb H}  n } } + c_2 + \frac{\lambda_{\mb W}}{2} \rho + \frac{\lambda_{\mb H}^2 }{2\lambda_{\mb W}} \rho }_{ \xi\paren{ \rho, \lambda_{\mb W},\lambda_{\mb H} } }  + \frac{\lambda_{\mb b} }{2} \norm{\mb b}{2}^2 \\
 \;&\geq\; \underbrace{ - \frac{ \rho c_2}{ (1+c_4)(K-1) } \sqrt{ \frac{ \lambda_{\mb W} }{ \lambda_{\mb H}  n } } + c_5 + \lambda_{\mb W} \rho  }_{ \xi\paren{ \rho, \lambda_{\mb W},\lambda_{\mb H} } }  + \frac{\lambda_{\mb b} }{2} \norm{\mb b}{2}^2 \\
    \;&\geq\; \xi\paren{ \rho, \lambda_{\mb W},\lambda_{\mb H} },
\end{align*}
where the last inequality becomes an equality whenever either $\lambdab = 0$ or $\vb = \vzero$. %\js{By the way, typically one never regularizers the bias terms (i.e. $\lambda_b=0$). I'm wondering if we should include this term in $f$ at all.}\zz{Good point. I am not sure if the bias term is regularized or not in practice. Tianyu told me the default implementation in Pytorch does include the regularizer for the bias term. But I am also thinking about whether including the bias term in $f$. On one hand, our result covers the case without the regularizer for the bias term. But on the other hand, our result indicate the bias term in the last layer has no much effect, which maybe a little bit surprising. The results in CIFAR10 and MNIST indeed show that there is no difference in terms of both training and testing without the bias term}. 
Furthermore, by Lemma \ref{lem:lower-bound-equality-cond-ls}, we know that the inequality $f(\mb W,\mb H,\mb b)\;\geq\; \xi\paren{ \rho, \lambda_{\mb W},\lambda_{\mb H} }$ becomes an equality \emph{if and only if} $(\mb W,\mb H,\mb b)$ satisfy the following
\begin{itemize}
    \item[(a)] $\norm{\mb w }{2} \;=\; \norm{\mb w^1}{2} \;=\; \norm{\mb w^2}{2} \;=\; \cdots \;=\; \norm{\mb w^K}{2}$;
    \item[(b)] $\mb b = b \mb 1$, where either $b = 0$ or $\lambdab = 0$;
    \item[(c)] $\ol{\mb h}_{i} \;:=\; \frac{1}{K} \sum_{j=1}^K \mb h_{j,i} \;=\; \mb 0, \quad \forall \; i \in [n]$, and $\sqrt{ \frac{ \lambda_{\mb W}  }{ \lambda_{\mb H} n } } \vw^k \;=\; \vh_{k,i},\quad \forall \; k\in[K],\; i\in[n]$;
    \item[(d)] $\mb W \mb W^\top \;=\; \frac{\rho }{K-1} \paren{ \mb I_K - \frac{1 }{K} \mb 1_K \mb 1_K^\top }$;
    \item[(e)] $c_1 \;=\; \frac{\exp(\frac{\rho}{K}\sqrt{\frac{\lambdaW}{\lambdaH n}})}{(K-1)\exp\paren{{\frac{-\rho}{K(K-1)}\sqrt{\frac{\lambdaW}{\lambdaH n}}}}}$
    \item[(f)] $c_4 \;=\; \brac{(K-1)\exp\bracket{-\frac{\rho}{K-1}\sqrt{\frac{\lambdaW}{\lambdaH n}}}}^{-1}$.
\end{itemize}
To finish the proof, we only need to show that $\rho = \norm{\mb W}{F}^2$ must be finite for any fixed $\lambdaW,\lambdaH>0$.
\end{proof}
%$(ii)$ $c_1  \rightarrow \frac{1}{K-1}$ and $c_2 \rightarrow \log K$ when $\rho\rightarrow 0$, and $(iii)$ $c_1  \rightarrow \infty$ and $c_2 \rightarrow 0$ when $\rho\rightarrow +\infty$. Thus, as plotted in \Cref{fig:obj-lower-bound}, $\xi(\rho;\lambdaW,\lambdaH) \rightarrow \log K$ when $\rho\rightarrow 0$ and $\xi(\rho;\lambdaW,\lambdaH) \rightarrow \infty$ when $\rho\rightarrow \infty$, and $\xi(\rho;\lambdaW,\lambdaH)$ achieves its minimum at a finite $\rho$.  One can verify that all the inequalities in \eqref{eq:cross-entropy-lower-bound} and \eqref{eq:all-cross-entropy-lower-bound} (and hence \eqref{eq:obj-lower-boound}) achieve equality when $(\mW,\mH,\vb)$ have the form as in \Cref{thm:global-minima}. 

\subsection{Supporting Lemmas}

We first characterize the following balance property between $\mW$ and $\mH$ for any critical point  $(\mW,\mH,\vb)$ of our loss function:

\begin{lemma}\label{lem:critical-balance-ls} 
Let $\rho = \norm{\mb W }{F}^2$. Any critical point $(\mW,\mH,\vb)$ of \eqref{eq:obj-app-ls} obeys
\begin{align}\label{eq:critical-balance-ls}
    \mW^\top\mW \;=\; \frac{\lambda_{\mH}}{\lambda_{\mW}}\mH\mH^\top\quad \text{and}\quad \rho \;=\; \norm{\mb W}{F}^2 \;=\; \frac{\lambda_{\mH}}{\lambda_{\mW}} \norm{\mb H}{F}^2.
\end{align}

\end{lemma}

\begin{proof}[Proof of Lemma \ref{lem:critical-balance-ls}]
By definition, any critical point $(\mW,\mH,\vb)$ of \eqref{eq:obj-app-ls} satisfies the following:
\begin{align}
    	\nabla_{\mW}f(\mW,\mH,\vb) \;&=\; \nabla_{\mb Z = \mb W\mb H}\; g(\mW\mH + \vb \vone^\top)\mH^\top + \lambdaW \mW \;=\; \vzero,\label{eqn:W-crtical} \\
	\nabla_{\mH}f(\mW,\mH,\vb) \;&=\;  \mW^\top \nabla_{\mb Z = \mb W\mb H}\; g(\mW\mH + \vb\vone^\top) + \lambdaH \mH \;=\; \vzero. \label{eqn:H-crtical}
\end{align}
Left multiply the first equation by $\mb W^\top$ on both sides and then right multiply second equation by $\mH^\top$ on both sides, it gives
\begin{align*}
    \mb W^\top \nabla_{\mb Z = \mb W\mb H}\; g(\mW\mH + \vb\vone^\top)\mH^\top \;&=\; - \lambdaW \mb W^\top \mW , \\
     \mb W^\top \nabla_{\mb Z = \mb W\mb H}\; g(\mW\mH + \vb\vone^\top)\mH^\top  \;&=\; - \lambdaH \mb H^\top \mH.
\end{align*}
Therefore, combining the equations above, we obtain
\begin{align*}
    \lambdaW \mW^\top \mW \;=\; \lambdaH \mH \mH^\top.
\end{align*}
Moreover, we have
\begin{align*}
    \rho\;=\; \norm{\mb W}{F}^2 \;=\; \trace \paren{ \mb W^\top \mb W } \;=\;  \frac{ \lambda_{\mb H} }{ \lambda_{\mb W} } \trace \paren{ \mb H \mb H^\top } \;=\; \frac{ \lambda_{\mb H} }{ \lambda_{\mb W} } \trace \paren{ \mb H^\top\mb H  } \;=\; \frac{ \lambda_{\mb H} }{ \lambda_{\mb W} } \norm{\mb H}{F}^2,
\end{align*}
as desired.
\end{proof}

\begin{lemma}\label{lem:lower-bound-g-ls}
Let $\mb W = \begin{bmatrix} (\mb w^1)^\top \\ \vdots \\ (\mb w^K)^\top 
\end{bmatrix}\in \bb R^{K \times d}$, $\mH = \begin{bmatrix}\vh_{1,1} \cdots \vh_{K,n} \end{bmatrix}\in \bb R^{d \times N}$, $N= nK$, and $\rho = \norm{\mb W}{F}^2$. Given  $g(\mW\mH + \vb\vone^\top)$ defined in \eqref{eqn:g-lls-app}, for any critical point $(\mW,\mH,\vb)$ of \eqref{eq:obj-app-ls} and $c_1, c_4>0$, we have
\begin{align}\label{eqn:lower-bound-g-ls}
   g(\mb W \mb H + \mb b \mb 1^\top) \;\geq\; - \frac{\rho c_2}{(1+c_4)(K-1)} \sqrt{ \frac{ \lambda_{\mb W}  }{ \lambda_{\mb H} n } } \;+\; c_5,
\end{align}
with $c_2 = 1-\frac{\alpha(K-1)(1+c_1)}{K}$, $c_3 = \paren{c_1\log c_1 -(c_1+1)\log(c_1 + 1)} + \frac{\alpha(K-1)}{K}\log\paren{K-1}$ and $c_5 = \frac{c_2}{1+c_4} \log\paren{ (1+c_4)(K-1) } + \frac{c_2c_4}{1+c_4} \log\paren{ \frac{1+c_4}{c_4} } -c_3 $. 
\end{lemma}

\begin{proof}[Proof of Lemma \ref{lem:lower-bound-g-ls}]
By Lemma \ref{lem:lls-lower-bound} with $\mb z_{k,i} = \mW\vh_{k,i} + \vb$, since the scalar $c_1>0$ and $c_4>0$ can be arbitrary, we choose the same $c_1,c_2, c_3, c_4, c_5$ for all $i\in[n]$ and $k \in [K]$, we have the following lower bound for $ g(\mb W \mb H + \mb b \mb 1^\top)$ as 
\begin{align}
    & \frac{(1+c_4)(K-1)}{c_2} \brac{g(\mb W \mb H + \mb b \mb 1^\top) -c_5  }  \nonumber  \\
    \;=\;&\frac{(1+c_4)(K-1)}{c_2}\brac{ \frac{1}{N}\sum_{k=1}^K\sum_{i=1}^n \Lls(\mW\vh_{k,i} + \vb,\vy_k) - c_5  }  \nonumber \\
     \;\geq\;& \frac{1}{ N} \sum_{k=1}^K\sum_{i=1}^n \Bigg[ \sum_{j=1}^K \paren{  \mb h_{k,i}^\top \mb w^j +b_j} - K \paren{  \mb h_{k,i}^\top \mb w^k + b_k } \Bigg]  \label{eqn:g-lower-1-ls} \\
     \;=\;&  \frac{1}{ N} \sum_{i=1}^n\Bigg[  \paren{\sum_{k=1}^K \sum_{j=1}^K \mb h_{k,i}^\top \mb w^j - K \sum_{k=1}^K  \mb h_{k,i}^\top \mb w^k } \;+\; \underbrace{\sum_{k=1}^K \sum_{j=1}^K\paren{  b_j- b_k } }_{=0}\Bigg]  \nonumber \\
     \;=\;& \frac{1}{ N} \sum_{i=1}^n  \paren{\sum_{k=1}^K \sum_{j=1}^K  \mb h_{j,i}^\top  \mb w^k - K \sum_{k=1}^K  \mb h_{k,i}^\top \mb w^k }  \nonumber \\
     \;=\;& \frac{K}{ N} \sum_{i=1}^n \sum_{k=1}^K  \brac{ \bigg( \frac{1}{K} \sum_{j=1}^K (\mb h_{j,i} - \mb h_{k,i}) \bigg)^\top \mb w^k } \;=\; \frac{1}{ n} \sum_{i=1}^n \sum_{k=1}^K  \paren{ \ol{\mb h}_{i} - \mb h_{k,i} }^\top \mb w^k,  \nonumber
\end{align}
where for the last equality we let $\ol{\mb h}_{i} = \frac{1}{K} \sum_{j=1}^K \mb h_{j,i}$. Furthermore, from the AM-GM inequality in Lemma \ref{lem:young-inequality}, we know that for any $\mb u,\mb v \in \bb R^K$ and any $c_6>0$,
\begin{align*}
    \mb u^\top \mb v \;\leq\; \frac{c_6}{2} \norm{\mb u}{2}^2 \;+\; \frac{1}{2c_6} \norm{\mb v}{2}^2,
\end{align*}
where the inequality becomes an equality when $c_3\vu= \vv$. Thus, we further have
\begin{align*}
     &\frac{(1+c_4)(K-1)}{c_2} \brac{g(\mb W \mb H + \mb b \mb 1^\top) -c_5  } \\
     \;\geq\;& - \frac{c_6}{ 2} \sum_{k=1}^K \norm{\mb w^k}{2}^2 \;-\; \frac{1}{2c_6n} \sum_{i=1}^n \sum_{k=1}^K \norm{ \ol{\mb h}_i - \mb h_{k,i} }{2}^2 \\
     \;=\;& - \frac{c_6}{ 2} \sum_{k=1}^K \norm{\mb w^k}{2}^2 \;-\ \frac{1}{2c_6n} \sum_{i=1}^n \brac{ \paren{\sum_{k=1}^K \norm{ \mb h_{k,i} }{2}^2} - K \norm{ \ol{\mb h}_i }{2}^2 } \\
     \;=\;& - \frac{c_6}{ 2} \norm{\mb W}{F}^2 \;-\ \frac{1}{2c_6n}  \paren{ \norm{\mb H}{F}^2 - K  \sum_{i=1}^n \norm{ \ol{\mb h}_i }{2}^2 },  
\end{align*}
where the first inequality becomes an equality if and only if 
\begin{align}\label{eqn:lower-bound-attained-1-ls}
    c_6\vw^k = (\vh_{k,i} - \overline\vh_i),\quad \forall\; k\in[K],\;i\in[n].
\end{align}
Let $\rho = \norm{\mb W}{F}^2$. Now, by using Lemma \ref{lem:critical-balance-ls}, we have $\mb W^\top \mb W = \frac{ \lambda_{\mb H} }{ \lambda_{\mb W} } \mb H \mb H^\top  $, so that $\norm{\mb H}{F}^2 = \trace\paren{ \mb H \mb H^\top } =  \frac{ \lambda_{\mb W} }{ \lambda_{\mb H} } \trace \paren {\mb W^\top \mb W} =  \frac{ \lambda_{\mb W} }{ \lambda_{\mb H} } \rho $. Therefore, we have
\begin{align}\label{eqn:g-lower-2-ls}
   g(\mb W \mb H + \mb b \mb 1^\top) \geq - \frac{\rho c_2}{2(1+c_4)(K-1)} \paren { c_6  + \frac{ \lambda_{\mb W} }{ \lambda_{\mb H} }  \frac{1}{c_6 n }   } + c_5,
\end{align}
as desired. The last inequality achieves its equality if and only if 
\begin{align}\label{eqn:lower-bound-attained-2-ls}
    \overline \vh_i = \vzero,\quad \forall \; i\in[n].
\end{align}

Plugging this into \eqref{eqn:lower-bound-attained-1-ls}, we have
\begin{align*}
    c_6\vw^k \;=\; \vh_{k,i} \Rightarrow c_6^2 \;=\; \frac{ \sum_{i=1}^n\sum_{k=1}^K\norm{\vh_{k,i}}{2}^2 }{ n \sum_{k=1}^K\norm{\vw^k}{2}^2 } = \frac{\norm{\mH}{F}^2}{n\norm{\mW}{F}^2} = \frac{\lambdaW}{n\lambdaH}.
\end{align*}
This together with the lower bound in \eqref{eqn:g-lower-2-ls} gives
\begin{align*}
   g(\mb W \mb H + \mb b \mb 1^\top) \geq - \frac{\rho c_2}{(1+c_4)(K-1)} \sqrt{ \frac{ \lambda_{\mb W}  }{ \lambda_{\mb H} n } }  + c_5,
\end{align*}
as suggested in \eqref{eqn:lower-bound-g-ls}.
\end{proof}

Next, we show that the lower bound in \eqref{eqn:lower-bound-g-ls} is attained if and only if $(\mb W, \mb H,\mb b)$ satisfies the following conditions.  
\begin{lemma}\label{lem:lower-bound-equality-cond-ls}
Under the same assumptions of Lemma \ref{lem:lower-bound-g-ls},
the lower bound in \eqref{eqn:lower-bound-g-ls} is attained for any critical point $(\mb W,\mb H,\mb b)$ of \eqref{eq:obj-app-ls}
if and only if the following hold
\begin{align*}
    & \norm{\mb w^1}{2} \;=\; \norm{\mb w^2}{2} \;=\; \cdots \;=\; \norm{\mb w^K}{2}, \quad \text{and}\quad \mb b = b \mb 1, \\ 
    &\ol{\mb h}_{i} \;:=\; \frac{1}{K} \sum_{j=1}^K \mb h_{j,i} \;=\; \mb 0, \quad \forall \; i \in [n], \quad \text{and} \quad \sqrt{ \frac{ \lambda_{\mb W}  }{ \lambda_{\mb H} n } } \vw^k \;=\; \vh_{k,i},\quad \forall \; k\in[K],\; i\in[n], \\
    &\mb W \mb W^\top \;=\; \frac{\rho }{K-1} \paren{ \mb I_K - \frac{1 }{K} \mb 1_K \mb 1_K^\top }, \;\text{and}\; c_1 \;=\; \frac{\exp(\frac{\rho}{K}\sqrt{\frac{\lambdaW}{\lambdaH n}})}{(K-1)\exp\paren{{\frac{-\rho}{K(K-1)}\sqrt{\frac{\lambdaW}{\lambdaH n}}}}}\\
    &c_4 \;=\; \brac{(K-1)\exp\bracket{-\frac{\rho}{K-1}\sqrt{\frac{\lambdaW}{\lambdaH n}}}}^{-1}.
\end{align*}
\end{lemma}
The proof of Lemma \ref{lem:lower-bound-equality-cond-ls} utilizes the conditions in Lemma \ref{lem:lls-lower-bound}, and the conditions \eqref{eqn:lower-bound-attained-1-ls} and \eqref{eqn:lower-bound-attained-2-ls} during the proof of Lemma \ref{lem:lower-bound-g-ls}. 

\begin{proof}[Proof of Lemma \ref{lem:lower-bound-equality-cond-ls}]
From the proof of Lemma \ref{lem:lower-bound-g-ls}, if we want to attain the lower bound, we know that we need at least \eqref{eqn:lower-bound-attained-1-ls} and \eqref{eqn:lower-bound-attained-2-ls} to hold, which is equivalent to the following:
\begin{align}\label{eqn:lower-bound-attained-3-ls}
    \ol{\vh}_i \;=\;\frac{1}{K} \sum_{j=1}^K \mb h_{j,i} \;=\; \vzero,\quad \forall i\in [n], \quad \text{and}\quad 
    \sqrt{ \frac{ \lambda_{\mb W}  }{ \lambda_{\mb H} n } }  \vw^k \;=\;  \vh_{k,i},\quad \forall \; k\in [K],\;i\in [n],
\end{align}
which further implies that
\begin{align}\label{eqn:w-sum-zero-ls}
    \sum_{k=1}^K \mb w^k \;=\; \mb 0.
\end{align}
Next, under the condition \eqref{eqn:lower-bound-attained-3-ls}, if we want \eqref{eqn:lower-bound-g-ls} to become an equality, we only need \eqref{eqn:g-lower-1-ls} to become an equality, which is true if and only if the condition \eqref{eqn:lls-lower-bound-equality} in Lemma \ref{lem:lls-lower-bound} holds for $\mb z_{k,i} = \mW\vh_{k,i} + \vb$ for all $i\in[n]$ and $k \in [K]$. First, let $[\mb z_{k,i}]_j = \mb h_{k,i}^\top \mb w^j + b_j $, where we have
\begin{align}
    \sum_{j=1}^K [\mb z_{k,i}]_j \;=\;  \mb h_{k,i}^\top \sum_{j=1}^K \mb w^j  + \sum_{j=1}^K b_j \;&=\; \sqrt{ \frac{ \lambda_{\mb H} n }{ \lambda_{\mb W} } }  \mb h_{k,i}^\top  \sum_{j=1}^K \mb h_{j,i}  + \sum_{j=1}^K b_j \nonumber  \\
    \;&=\;  \sqrt{ \frac{ \lambda_{\mb H} n }{ \lambda_{\mb W} } } K  \mb h_{k,i}^\top  \ol{\mb h}_i + \sum_{j=1}^K b_j \;=\; K \ol{b} \label{eqn:g-lower-3-ls}
\end{align}
with $\ol{b} = \frac{1}{K} \sum_{i=1}^K b_i$, and 
\begin{align}
    K[\mb z_{k,i}]_k \;=\; K \mb h_{k,i}^\top  \mb w^k  + Kb_k \;=\; \sqrt{ \frac{ \lambda_{\mb W}  }{ \lambda_{\mb H} n } } \paren{K\norm{\mb w^k}{2}^2} + Kb_k. \label{eqn:g-lower-4-ls}
\end{align}
Based on \eqref{eqn:g-lower-3-ls}, \eqref{eqn:g-lower-4-ls}, and \eqref{eqn:lls-lower-bound-equality} from Lemma \ref{lem:lls-lower-bound}, we have 
\begin{align}
    c_4 \;&=\; \brac{(K-1) \exp \paren{  \frac{ \paren{\sum_{j=1}^K [\mb z_{k,i}]_j} - K [\mb z_{k,i}]_k}{K-1} }  }^{-1}  \nonumber   \\
    \;&=\; \brac{(K-1)\exp\bracket{\frac{K}{K-1} \paren{ \ol{b} -  \sqrt{ \frac{ \lambda_{\mb W}  }{ \lambda_{\mb H} n } } \norm{\mb w^k}{2}^2 - b_k  } }}^{-1}. \label{eqn:c-form-1-ls}
\end{align}
Since the scalar $c_4>0$ is chosen to be the same for all $k \in [K]$, we have
\begin{align}\label{eqn:g-lower-5-ls}
    \sqrt{ \frac{ \lambda_{\mb W}  }{ \lambda_{\mb H} n } } \norm{\mb w^k}{2}^2 + b_k \;=\; \sqrt{ \frac{ \lambda_{\mb W}  }{ \lambda_{\mb H} n } } \norm{\mb w^\ell}{2}^2 + b_\ell, \quad \forall \; \ell \not =k. 
\end{align}
Second, since $[\mb z_{k,i}]_j = [\mb z_{k,i}]_{\ell}$ for all $\forall j,\ell \neq k,\; k\in[K]$, from \eqref{eqn:lower-bound-attained-3-ls} we have
\begin{align}
     &\mb h_{k,i}^\top \mb w^j  + b_j \;=\;  \mb h_{k,i}^\top \mb w^\ell+ b_\ell, \quad \; \forall j,\ell \neq k,\; k\in[K] \nonumber  \\
     \Longleftrightarrow \quad & \sqrt{ \frac{ \lambda_{\mb W}  }{ \lambda_{\mb H} n } } (\mb w^k)^\top \mb w^j + b_j \;=\; \sqrt{ \frac{ \lambda_{\mb W}  }{ \lambda_{\mb H} n } }  (\mb w^k)^\top \mb w^\ell + b_\ell,\quad  \forall j,\ell \neq k,\; k\in[K]. \label{eqn:g-lower-7-ls}
\end{align}
Based on this and \eqref{eqn:w-sum-zero-ls}, we have
\begin{align}
    \sqrt{ \frac{ \lambda_{\mb W}  }{ \lambda_{\mb H} n } }\norm{\mb w^k}{2}^2 + b_k \;&=\; - \sqrt{ \frac{ \lambda_{\mb W}  }{ \lambda_{\mb H} n } } \sum_{j\not = k} (\mb w^j)^\top \mb w^k +   b_k \nonumber  \\ 
    \;&=\; -(K-1)\sqrt{ \frac{ \lambda_{\mb W}  }{ \lambda_{\mb H} n } }\underbrace{ (\mb w^{\ell})^\top \mb w^k}_{ \ell \not= k, \ell \in [K] } +  \paren{ b_k + \sum_{j\not= \ell, k} \paren{b_\ell - b_j } }  \nonumber  \\
    \;&=\; -(K-1) \sqrt{ \frac{ \lambda_{\mb W}  }{ \lambda_{\mb H} n } } (\mb w^{\ell})^\top \mb w^k + \brac{ 2b_k + (K-1) b_\ell - K \ol{b} } \label{eqn:g-lower-6-ls}
\end{align}
for all $\ell \neq k$. Combining \eqref{eqn:g-lower-5-ls} and \eqref{eqn:g-lower-6-ls}, for all $k,\ell \in [K]$ with $k \not = \ell $ we have 
\begin{align*}
     2b_k + (K-1) b_\ell - K \ol{b}  \;=\; 2b_\ell  + (K-1) b_k - K \ol{b}\quad \Longleftrightarrow \quad b_k \;=\; b_\ell, \; \forall \; k\not = \ell.  
\end{align*}
Therefore, we can write $\mb b = b \mb 1_K$ for some $b>0$. Moreover, since $b_k = b_\ell$ for all $k \not = \ell $, \eqref{eqn:g-lower-5-ls} and \eqref{eqn:g-lower-7-ls}, and \eqref{eqn:g-lower-6-ls} further imply that
\begin{align}
    &\norm{\mb w^1}{2}\;=\; \norm{\mb w^2}{2}\;=\; \cdots \;=\; \norm{\mb w^K}{2},\quad \text{and}\quad \norm{\mb w^k}{2}^2 \;=\; \frac{1}{K} \norm{\mb W}{F}^2 \;=\; \frac{\rho}{K}, \label{eqn:g-lower-8-ls} \\
    & (\mb w^j)^\top \mb w^k \;=\; (\mb w^\ell)^\top \mb w^k \;=\; - \frac{1}{K-1} \norm{\mb w^k}{2}^2\;=\; - \frac{\rho}{K(K-1)}, \quad  \forall j,\ell \neq k,\; k\in[K],\label{eqn:g-lower-9-ls}
\end{align}
where \eqref{eqn:g-lower-9-ls} is equivalent to
\begin{align*}
    \mb W \mb W^\top \;=\; \frac{\rho }{K-1} \paren{ \mb I_K - \frac{1 }{K} \mb 1_K \mb 1_K^\top }.
\end{align*}
Finally, plugging the results in \eqref{eqn:g-lower-8-ls} and \eqref{eqn:g-lower-9-ls} into \eqref{eqn:c-form-1-ls}, we have
\begin{align*}
    c_4  \;=\; \brac{(K-1)\exp\paren{  -  \frac{\rho}{K-1} \sqrt{ \frac{ \lambda_{\mb W}  }{ \lambda_{\mb H} n } }  } }^{-1},
\end{align*}
as desired. Similarly, it works for $c_1$:
\begin{align*}
    c_1 \;=\; \frac{\exp(z_k)}{\sum_{i\neq k}^K\exp(z_i)} 
    \;=\; \frac{\exp(\frac{\rho}{K}\sqrt{\frac{\lambdaW}{\lambdaH n}})}{(K-1)\exp\paren{{\frac{-\rho}{K(K-1)}\sqrt{\frac{\lambdaW}{\lambdaH n}}}}}
\end{align*}
as desired.
\end{proof}

\begin{lemma}\label{lem:lls-lower-bound}
Let $\mb y_k\in \bb R^K$ be an one-hot vector with the $k$th entry equalling $1$ for some $k\in [K]$. For any vector $\vz\in\R^{K}$ and $c_1, c_4>0$, the label-smoothing loss $\Lls (\vz,\vy_k, \alpha)$ with $\vy_k$ can be lower bounded by
\begin{align}\label{eqn:lls-lower-bound}
     \Lls (\vz,\vy_k) \;\geq \;  \frac{c_2}{1+c_4}\frac{ \paren{\sum_{i=1}^K z_i} - K z_k }{K-1} + c_5,
\end{align}
where $c_2 = 1-\frac{\alpha(K-1)(1+c_1)}{K}$, $c_3 = \paren{c_1\log c_1 -(c_1+1)\log(c_1 + 1)} + \frac{\alpha(K-1)}{K}\log\paren{K-1}$ and $c_5 = \frac{c_2}{1+c_4} \log\paren{ (1+c_4)(K-1) } + \frac{c_2c_4}{1+c_4} \log\paren{ \frac{1+c_4}{c_4} } -c_3 $. The inequality becomes an equality when
\begin{align}\label{eqn:lls-lower-bound-equality}
    &z_i \;=\; z_j,\quad \forall i,j \not = k, \nonumber\\
    &c_1 \;=\; \frac{\exp(z_k)}{\sum_{i\neq k}^K\exp(z_i)} \nonumber\\
    &c_4 \;=\; \brac{(K-1) \exp \paren{  \frac{ \paren{\sum_{i=1}^K z_i} - K z_k}{K-1} }  }^{-1}.
\end{align}
\end{lemma}

\begin{proof}[Proof of Lemma \ref{lem:lls-lower-bound}]
Notice that for any vector $\vz\in\R^{K}$, the label-smoothing loss with $\vy_k$ can be lower bounded by 
\begin{align*}
    \Lls (\vz,\vy_k) & \;=\; \paren{(1-\alpha)+\frac{\alpha}{K}}\log \paren{\frac{\sum_{j=1}^K \exp(z_j)}{\exp(z_k)}} + \frac{\alpha}{K}\sum_{i\neq k}^K \log \paren{\frac{\sum_{j=1}^K \exp(z_j)}{\exp(z_i)}}\\
    & = \log \paren{\frac{\sum_{j=1}^K \exp(z_j)}{\exp(z_k)}} + \frac{\alpha}{K}\sum_{i\neq k}^K (z_k - z_i)\\
    & = \log \paren{\frac{\sum_{j=1}^K \exp(z_j)}{\exp(z_k)}} + \frac{\alpha}{K} ((K-1)z_k - \sum_{i\neq k} z_i )
\end{align*}

\begin{align}
    &\Lls (\vz,\vy_k) \;=\; \paren{(1-\alpha)+\frac{\alpha}{K}}\log \paren{\frac{\sum_{j=1}^K \exp(z_j)}{\exp(z_k)}} + \frac{\alpha}{K}\sum_{i\neq k}^K \log \paren{\frac{\sum_{j=1}^K \exp(z_j)}{\exp(z_i)}} \nonumber\\
    \;=\;& \paren{(1-\alpha)+\frac{\alpha}{K}}\log \paren{\frac{\sum_{j=1}^K \exp(z_j)}{\exp(z_k)}} + \frac{\alpha(K-1)}{K}\log\paren{\sum_{j=1}^K \exp(z_j)}  - \frac{\alpha}{K}\sum_{i\neq k}^K\log\paren{\exp(z_i)} \nonumber\\
    \;\geq\;& \paren{(1-\alpha)+\frac{\alpha}{K}}\log \paren{\frac{\sum_{j=1}^K \exp(z_j)}{\exp(z_k)}} + \frac{\alpha(K-1)}{K}\log\paren{\sum_{j=1}^K \exp(z_j)} -\frac{\alpha(K-1)}{K}\log\paren{\frac{1}{K-1}\sum_{i\neq k}^K \exp(z_i)} \label{lem:lls-lower-bound-inequality1}\\
    \;=\;& \paren{(1-\alpha)+\frac{\alpha}{K}}\log \paren{1+\underbrace{\frac{\sum_{i\neq k}^K \exp(z_i)}{\exp(z_k)}}_{m}} + \frac{\alpha(K-1)}{K}\log\paren{1+\frac{\exp(z_k)}{\sum_{i\neq k}^K \exp(z_i)}} + \frac{\alpha(K-1)}{K}\log\paren{K-1} \nonumber\\
    \;=\;& \paren{(1-\alpha)+\frac{\alpha}{K}}\log\paren{1+m}+\frac{\alpha(K-1)}{K}\log\paren{\frac{m+1}{m}}  + \frac{\alpha(K-1)}{K}\log\paren{K-1} \nonumber\\
    \;=\;& \paren{\log(1+m)-\frac{\alpha(K-1)}{K}\log m}+ \frac{\alpha(K-1)}{K}\log\paren{K-1} \nonumber\\
    \;\geq\;& \paren{\log(1+m)-\frac{\alpha(K-1)}{K}\paren{(1+c_1)\log(1+m)+c_1\log c_1 -(c_1+1)\log(c_1 + 1)}} + \frac{\alpha(K-1)}{K}\log\paren{K-1} \label{lem:lls-lower-bound-inequality2}\\
    \;=\;&\underbrace{(1-\frac{\alpha(K-1)(1+c_1)}{K})}_{c_2}\log(1+m) - \underbrace{\paren{\paren{c_1\log c_1 -(c_1+1)\log(c_1 + 1)}} + \frac{\alpha(K-1)}{K}\log\paren{K-1}}_{c_3} \nonumber\\
    \;=\;& c_2 \log \paren{ 1+ \sum_{i \not= k}\exp \paren{ z_i - z_k } } - c_3 \nonumber  \\
    \;\geq\;& c_2 \log \paren{  1+ (K-1) \exp \paren{ \sum_{i \not = k} \frac{z_i - z_k}{ K-1 }  } } -c_3 \label{lem:lls-lower-bound-inequality3} \\
    % \;=\;& c_2\log \paren{  \frac{c_4}{1+c_4} \frac{1+c_4}{c_4}  + \frac{1}{1+c_4} (1+c_4)  (K-1) \exp \paren{ \frac{ \sum_{i=1}^K z_i - K z_k }{K-1} } } +c_3 \nonumber\\
     \;\geq \;&  \frac{c_2}{1+c_4}  \log \paren{  (1+c_4)(K-1) \exp \paren{ \frac{ \sum_{i=1}^K z_i - K z_k }{K-1} } } + \frac{c_2c_4}{1+c_4} \log\paren{ \frac{1+c_4}{c_4} } - c_3 \label{lem:lls-lower-bound-inequality4} \\
     \;=\;& \frac{c_2}{1+c_4}\frac{ \paren{\sum_{i=1}^K z_i} - K z_k }{K-1} + \underbrace{  \frac{c_2}{1+c_4} \log\paren{ (1+c_4)(K-1) } + \frac{c_2c_4}{1+c_4} \log\paren{ \frac{1+c_4}{c_4} } -c_3 }_{c_5} \nonumber\\
     \;=\;& \frac{c_2}{1+c_4}\frac{ \paren{\sum_{i=1}^K z_i} - K z_k }{K-1} + c_5 \nonumber
\end{align}
where the first inequality \eqref{lem:lls-lower-bound-inequality1} and the third inequality \eqref{lem:lls-lower-bound-inequality3} follows from the Jensen's inequality that
\begin{align*}
     -\sum_{i\neq k}^K\log(\exp(z_i)) \;&=\; -(K-1) \sum_{i \not= k}^K \frac{1}{K-1}\log(\exp(z_i)) \;\geq\; -(K-1) \log\paren{\sum_{i \not= k}^K\frac{\exp(z_i)}{K-1}}, \nonumber\\
     \sum_{i \not= k}^K\exp \paren{ z_i - z_k } \;&=\; (K-1) \sum_{i \not= k}^K \frac{1}{K-1} \exp \paren{ z_i - z_k } \;\geq\; (K-1)   \exp \paren{\sum_{i \not= k}^K \frac{z_i - z_k}{K-1}  },
\end{align*}
both of which achieve the equality only when $z_i = z_j$ for all $i,j \not= k$. The second inequality \eqref{lem:lls-lower-bound-inequality2} and the last inequality \eqref{lem:lls-lower-bound-inequality4} follows from the concavity of the $\log(\cdot)$ function 
\begin{align*}
    \log \paren{ tx+(1-t)x'} \geq t \log x + (1-t) \log x',
\end{align*}
for any $x,x' \in \bb R$ and $t \in [0,1]$, which becomes an equality iff $x = x'$, or $t=0 $, or $t=1$.\\
By choosing $t=\frac{c_1}{1+c_1}$, $x=\frac{1+c_1}{c_1}$, $x'=(1+c_1)m$ and $c_1>0$, we can have the second inequality \eqref{lem:lls-lower-bound-inequality2} as following:
\begin{align*}
    \log(1+m) \;&=\; \log(\frac{c_1}{1+c_1}\frac{1+c_1}{c_1}+\frac{1}{1+c_1}(1+c_1)m)\\
    \;&\geq\; \frac{c_1}{1+c_1}\log（\frac{1+c_1}{c_1}） + \frac{1}{1+c_1}\log\paren{(1+c_1)m}\\
    \;&=\; \log(1+c_1)-\frac{c_1}{1+c_1}\log(c_1)+\frac{1}{1+c_1}\log(m)\\
    -\log(m) \;&\geq\; (1+c_1)\log(1+c_1)-c_1\log(c_1)-(1+c_1)\log(1+m)
\end{align*}
The inequality becomes an equality if any only if
\begin{align*}
    \frac{1+c_1}{c_1} \;=\;   (1+c_1)  m \quad \text{or} \quad  c_1\;=\; 0, \quad \text{or} \quad  c_1\;=\; +\infty . 
\end{align*}
However, when $c_4=0$ or $ c_4= +\infty $, the equality is trivial. Therefore, we have
\begin{align*}
    c_1 \;=\; \frac{1}{m}\;=\;\frac{\exp(z_k)}{\sum_{i\neq k}^K\exp(z_i)}.
\end{align*}
Similarly, if we set $t=\frac{c_4}{1+c_4}$, $x=\frac{1+c_4}{c_4}$, $x'=(1+c_4)(K-1)\exp{\paren{\frac{\sum_{i=1}^K z_i-Kz_k}{K-1}}}$, and $c_4>0$, we can obtain the last inequality \eqref{lem:lls-lower-bound-inequality4} as following: 
\begin{align*}
     &\log \paren{  1+ (K-1) \exp \paren{ \sum_{i \not = k} \frac{z_i - z_k}{ K-1 }  } } \\
     \;=\;& \log \paren{  \frac{c_4}{1+c_4} \frac{1+c_4}{c_4}  + \frac{1}{1+c_4} (1+c_4)  (K-1) \exp \paren{ \frac{ \sum_{i=1}^K z_i - K z_k }{K-1} } }\\
     \;\geq \;&  \frac{1}{1+c_4}  \log \paren{  (1+c_4)(K-1) \exp \paren{ \frac{ \sum_{i=1}^K z_i - K z_k }{K-1} } } + \frac{c_4}{1+c_4} \log\paren{ \frac{1+c_4}{c_4} }\\
     \;=\;& \frac{1}{1+c_4}\frac{ \paren{\sum_{i=1}^K z_i} - K z_k }{K-1} + \frac{1}{1+c_4} \log\paren{ (1+c_4)(K-1) } + \frac{c_4}{1+c_4} \log\paren{ \frac{1+c_4}{c_4} },
\end{align*}
as desired. The last inequality becomes an equality if any only if
\begin{align*}
    \frac{1+c_4}{c_4} \;=\;   (1+c_4)  (K-1) \exp \paren{ \frac{ \sum_{i=1}^K z_i - K z_k }{K-1} } \quad \text{or} \quad  c_4\;=\; 0, \quad \text{or} \quad  c_4\;=\; +\infty . 
\end{align*}
However, when $c_4=0$ or $ c_4= +\infty $, the equality is trivial. Therefore, we have
\begin{align*}
    c_4 \;=\; \brac{(K-1) \exp \paren{  \frac{ \paren{\sum_{i=1}^K z_i} - K z_k}{K-1} }  }^{-1},
\end{align*}
as desired.
\end{proof}
