# Supplementary material for: Are All Losses Created Equal: A Neural Collapse Perspective
Source: arXiv:2210.02192 source file (2022-10-08)
Supplement: Supplementary file 8 [file experiments.tex]

{In this section, we provide with more details for reproducing the experiments presented in the paper. In particular, we emphasize that the datasets involved in the paper, namely MNIST and CIFAR10, are publicly available for academic usage: MNIST dataset is made available under the terms of the Creative Commons Attribution-Share Alike 3.0 license, and CIFAR10 dataset is made available under the MIT license. All experiments are conducted on a single RTX3090 GPU  with 24GB memory.}

\subsection{Metrics for Measuring \NC\;During Network Training.} \label{subsection:metric-NC-appendix}
We measure \NC\; for the learned last-layer classifiers and features based on the properties presented in \Cref{sec:intro}. Some of the metrics are similar to those presented in \cite{papyan2020prevalence}. First, we define the global mean and class mean of the last-layer features $\Brac{ \mb h_{k,i} }  $ as 
%\zz{Not sure if it is a good idea to use $\star$ here since $\star$ means the global minimizer in \Cref{thm:global-minima}.}
\begin{align*}
    \mb h_G \;=\; \frac{1}{nK} \sum_{k=1}^K  \sum_{i=1}^n \vh_{k,i},\quad \ol{\mb h}_k \;=\; \frac{1}{n} \sum_{i=1}^n \vh_{k,i} \;(1\leq k\leq K).
\end{align*}

\begin{itemize}[leftmargin=*]
    \item \textbf{\emph{Within-class Variability Collapse for the Learned Features $\mb H$.}} We introduce the within-class and between-class covariance matrices as
\begin{align*}
    \mb \Sigma_W \;:=\; \frac{1}{nK} \sum_{k=1}^K \sum_{i=1}^n \paren{  \mb h_{k,i}  -  \ol{\mb h}_k } \paren{ \mb h_{k,i} - \ol{\mb h}_k }^\top   ,\quad \mb \Sigma_B \;:=\; \frac{1}{K} \sum_{k=1}^K \paren{ \ol{\mb h}_k - \mb h_G } \paren{ \ol{\mb h}_k - \mb h_G }^\top.
\end{align*}
Thus, we can measure the within-class variability collapse by measuring the magnitude of the between-class covariance $\mb \Sigma_B \in \bb R^{d \times d} $ compared to the within-class covariance $\mb \Sigma_W \in \bb R^{d \times d} $ of the learned features via
    \begin{align}\label{eq:NC1}
    \mc {NC}_1\;:=\;\frac{1}{K}\trace\parans{\mSigma_ W\mSigma_B^\dagger},
\end{align}
where $\mSigma_B^\dagger$ denotes the pseudo inverse of $\mSigma_B$.
\item \textbf{\emph{Convergence of the Learned Classifier $\mb W$ to a Simplex ETF.}} For the learned classifier $\mW \in\R^{K\times d}$, we quantify its closeness to a Simplex ETF up to scaling by % \begin{align}\label{eq:NC2}
% \mc {NC}_2\;:=\; \frac{\sqrt{K-1}}{K}  \norm{ \frac{K}{\norm{\mW }{F}^2} \mW \mW^{\top}\;-\; \frac{K}{K-1}  \paren{ \mb I_K - \frac{1}{K} \mb 1_K \mb 1_K^\top } }{F},
% \end{align}
\begin{align}\label{eq:NC2}
\mc {NC}_2\;:=\;  \norm{ \frac{\mW \mW^\top}{\norm{\mW \mW^\top}{F}} \;-\; \frac{1}{\sqrt{K-1}}  \paren{ \mb I_K - \frac{1}{K} \mb 1_K \mb 1_K^\top } }{F},
\end{align}
where we rescale the ETF in \eqref{eqn:simplex-ETF-closeness} so that $\frac{1}{\sqrt{K-1}}  \paren{ \mb I_K - \frac{1}{K} \mb 1_K \mb 1_K^\top } $ has unit energy (in Frobenius norm).
%where $\frac{\sqrt{K}}{\norm{\mW }{F}}\mW$ is the scaled version of $\mW$ such that it has the same energy (in Frobenius norm) with the Simplex ETF, as shown in \Cref{def:simplex-ETF} in the appendix.  
It should be noted that our metric $\mc {NC}_2$ combines two metrics used in \cite{papyan2020prevalence} to quantity to what extent the classifier approaches equiangularity and maximal-angle equiangularity.
\item \textbf{\emph{Convergence to Self-duality.}} Next, we measure the collapse of the learned features $\mb H$ to its dual $\mb W$. Let us define the centered class-mean matrix as
\begin{align*}
    \ol{\mb H} \;:=\; \begin{bmatrix}
\ol{\mb h}_1 - \mb h_G & \cdots & \ol{\mb h}_K - \mb h_G
\end{bmatrix} \in \bb R^{d \times K}.
\end{align*}
Thus, we measure the duality between the classifiers $\mb W$ and the centered class-means $\ol{\mb H}$ by
% \begin{align}\label{eq:NC3}
%     \mc {NC}_3\;:=\; \norm{ \frac{\mW^{\top}}{ \norm{\mW}{F}} - \frac{\ol{\mH} }{ \norm{\ol{\mH}}{F} } }{F}.
% \end{align}
%\zz{Maybe the following term}
\begin{align}\label{eq:NC3}
 \mc {NC}_3\;:=\; \norm{\frac{\mW \ol{\mH}}{\norm{\mW\ol{\mb H}}{F}}   \;-\; \frac{1}{\sqrt{K-1}}  \paren{ \mb I_K - \frac{1}{K} \mb 1_K \mb 1_K^\top} }{F}.
\end{align}
 
\item \textbf{\emph{Collapse of the Bias.}} In many cases, the global mean $\mb h_G$ of the features might not be zero,\footnote{For example, as discussed after \Cref{thm:global-minima} all the feature vectors in $\mb H$ would be nonnegative, because the nonnegative nonlinear operator ReLU has been applied at the end of the penultimate layer.} and the bias term $\vb$ would compensate for the global mean $\mb h_G$ in the sense that 
\begin{align*}
    \mb W \mb h_{k,i} + \mb b\;=\;  \mb W \paren{\mb h_{k,i} - \mb h_G} + \underbrace{ \mb W\mb h_G +  \mb b}_{= \mb 0}.
\end{align*}
Thus, we capture this collapsing phenomenon by measuring 
\begin{align}\label{eq:NC4}
    \mc {NC}_4 \;:=\; \norm{\vb + \mW \vh_G}{2}. 
\end{align}
\end{itemize}

\subsection{Additional Experiments}

\subsubsection{The Prevalence of \NC\;Across Different Optimization Algorithms}%\label{sec:exp-NC}

\begin{figure}[t]
    \centering
    \subfloat[$\mc {NC}_1$ (MNIST)]{\includegraphics[width=0.24\textwidth]{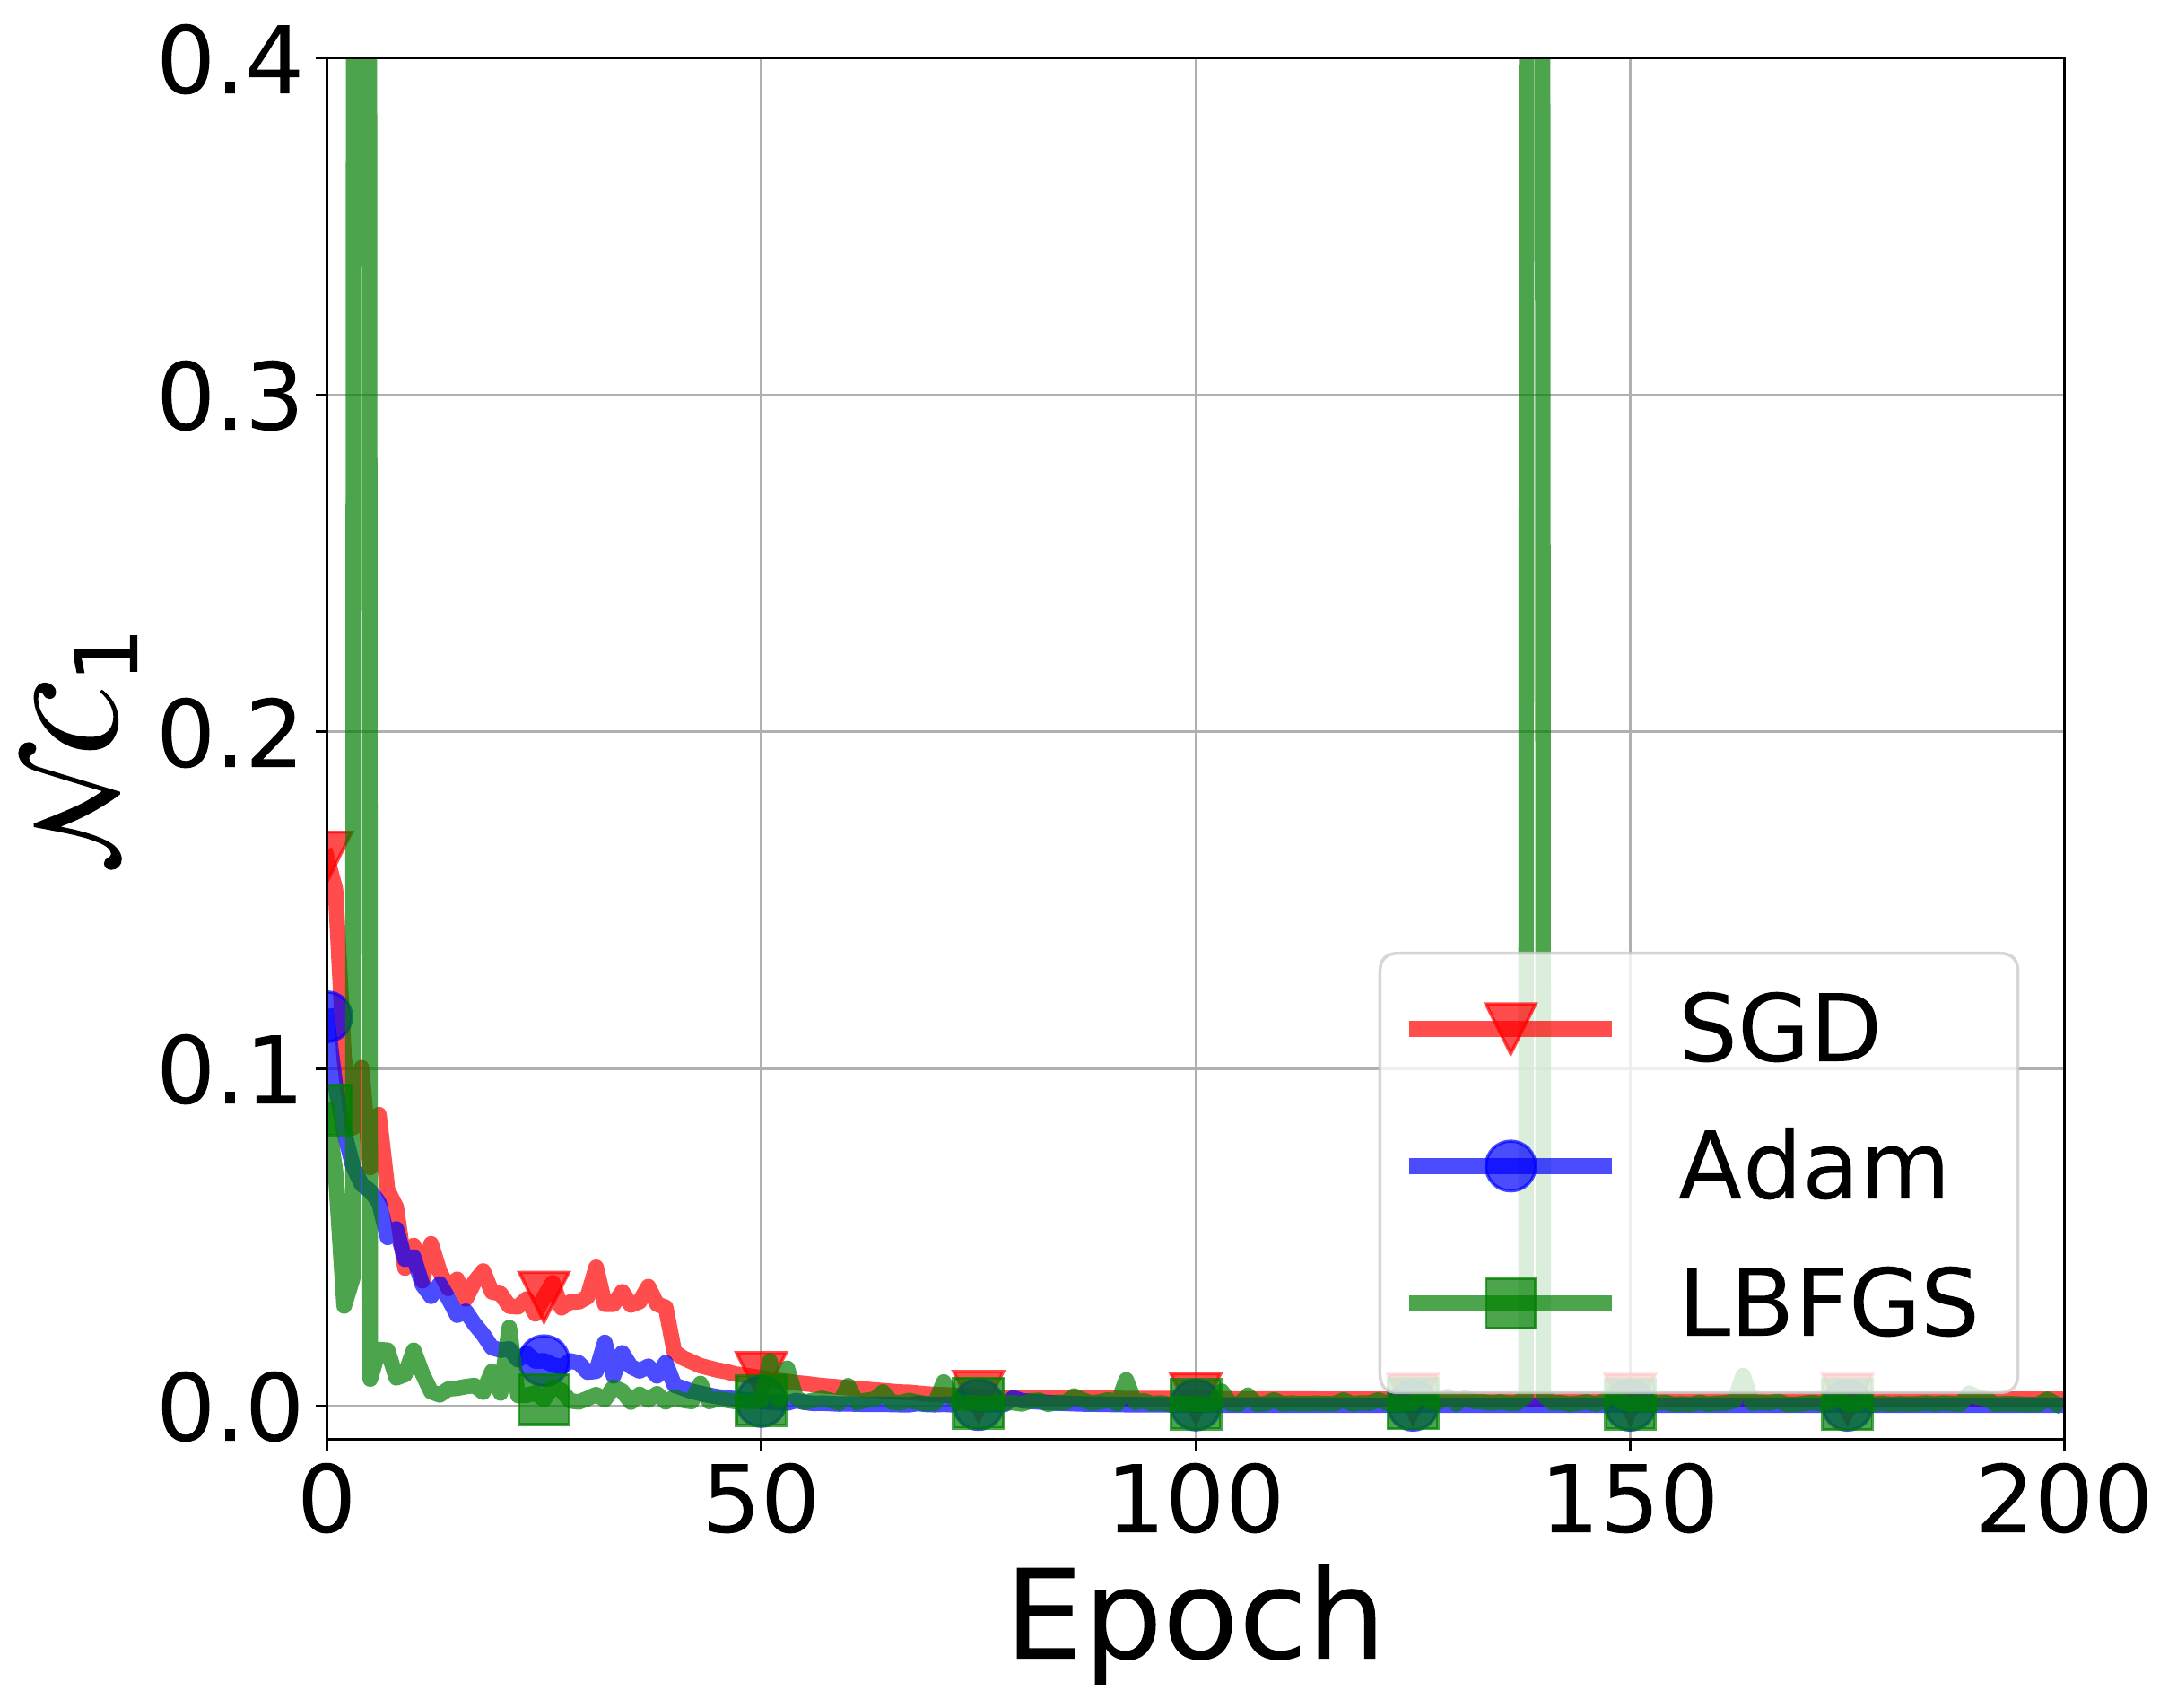}} \
    \subfloat[$\mc {NC}_2$ (MNIST)]{\includegraphics[width=0.24\textwidth]{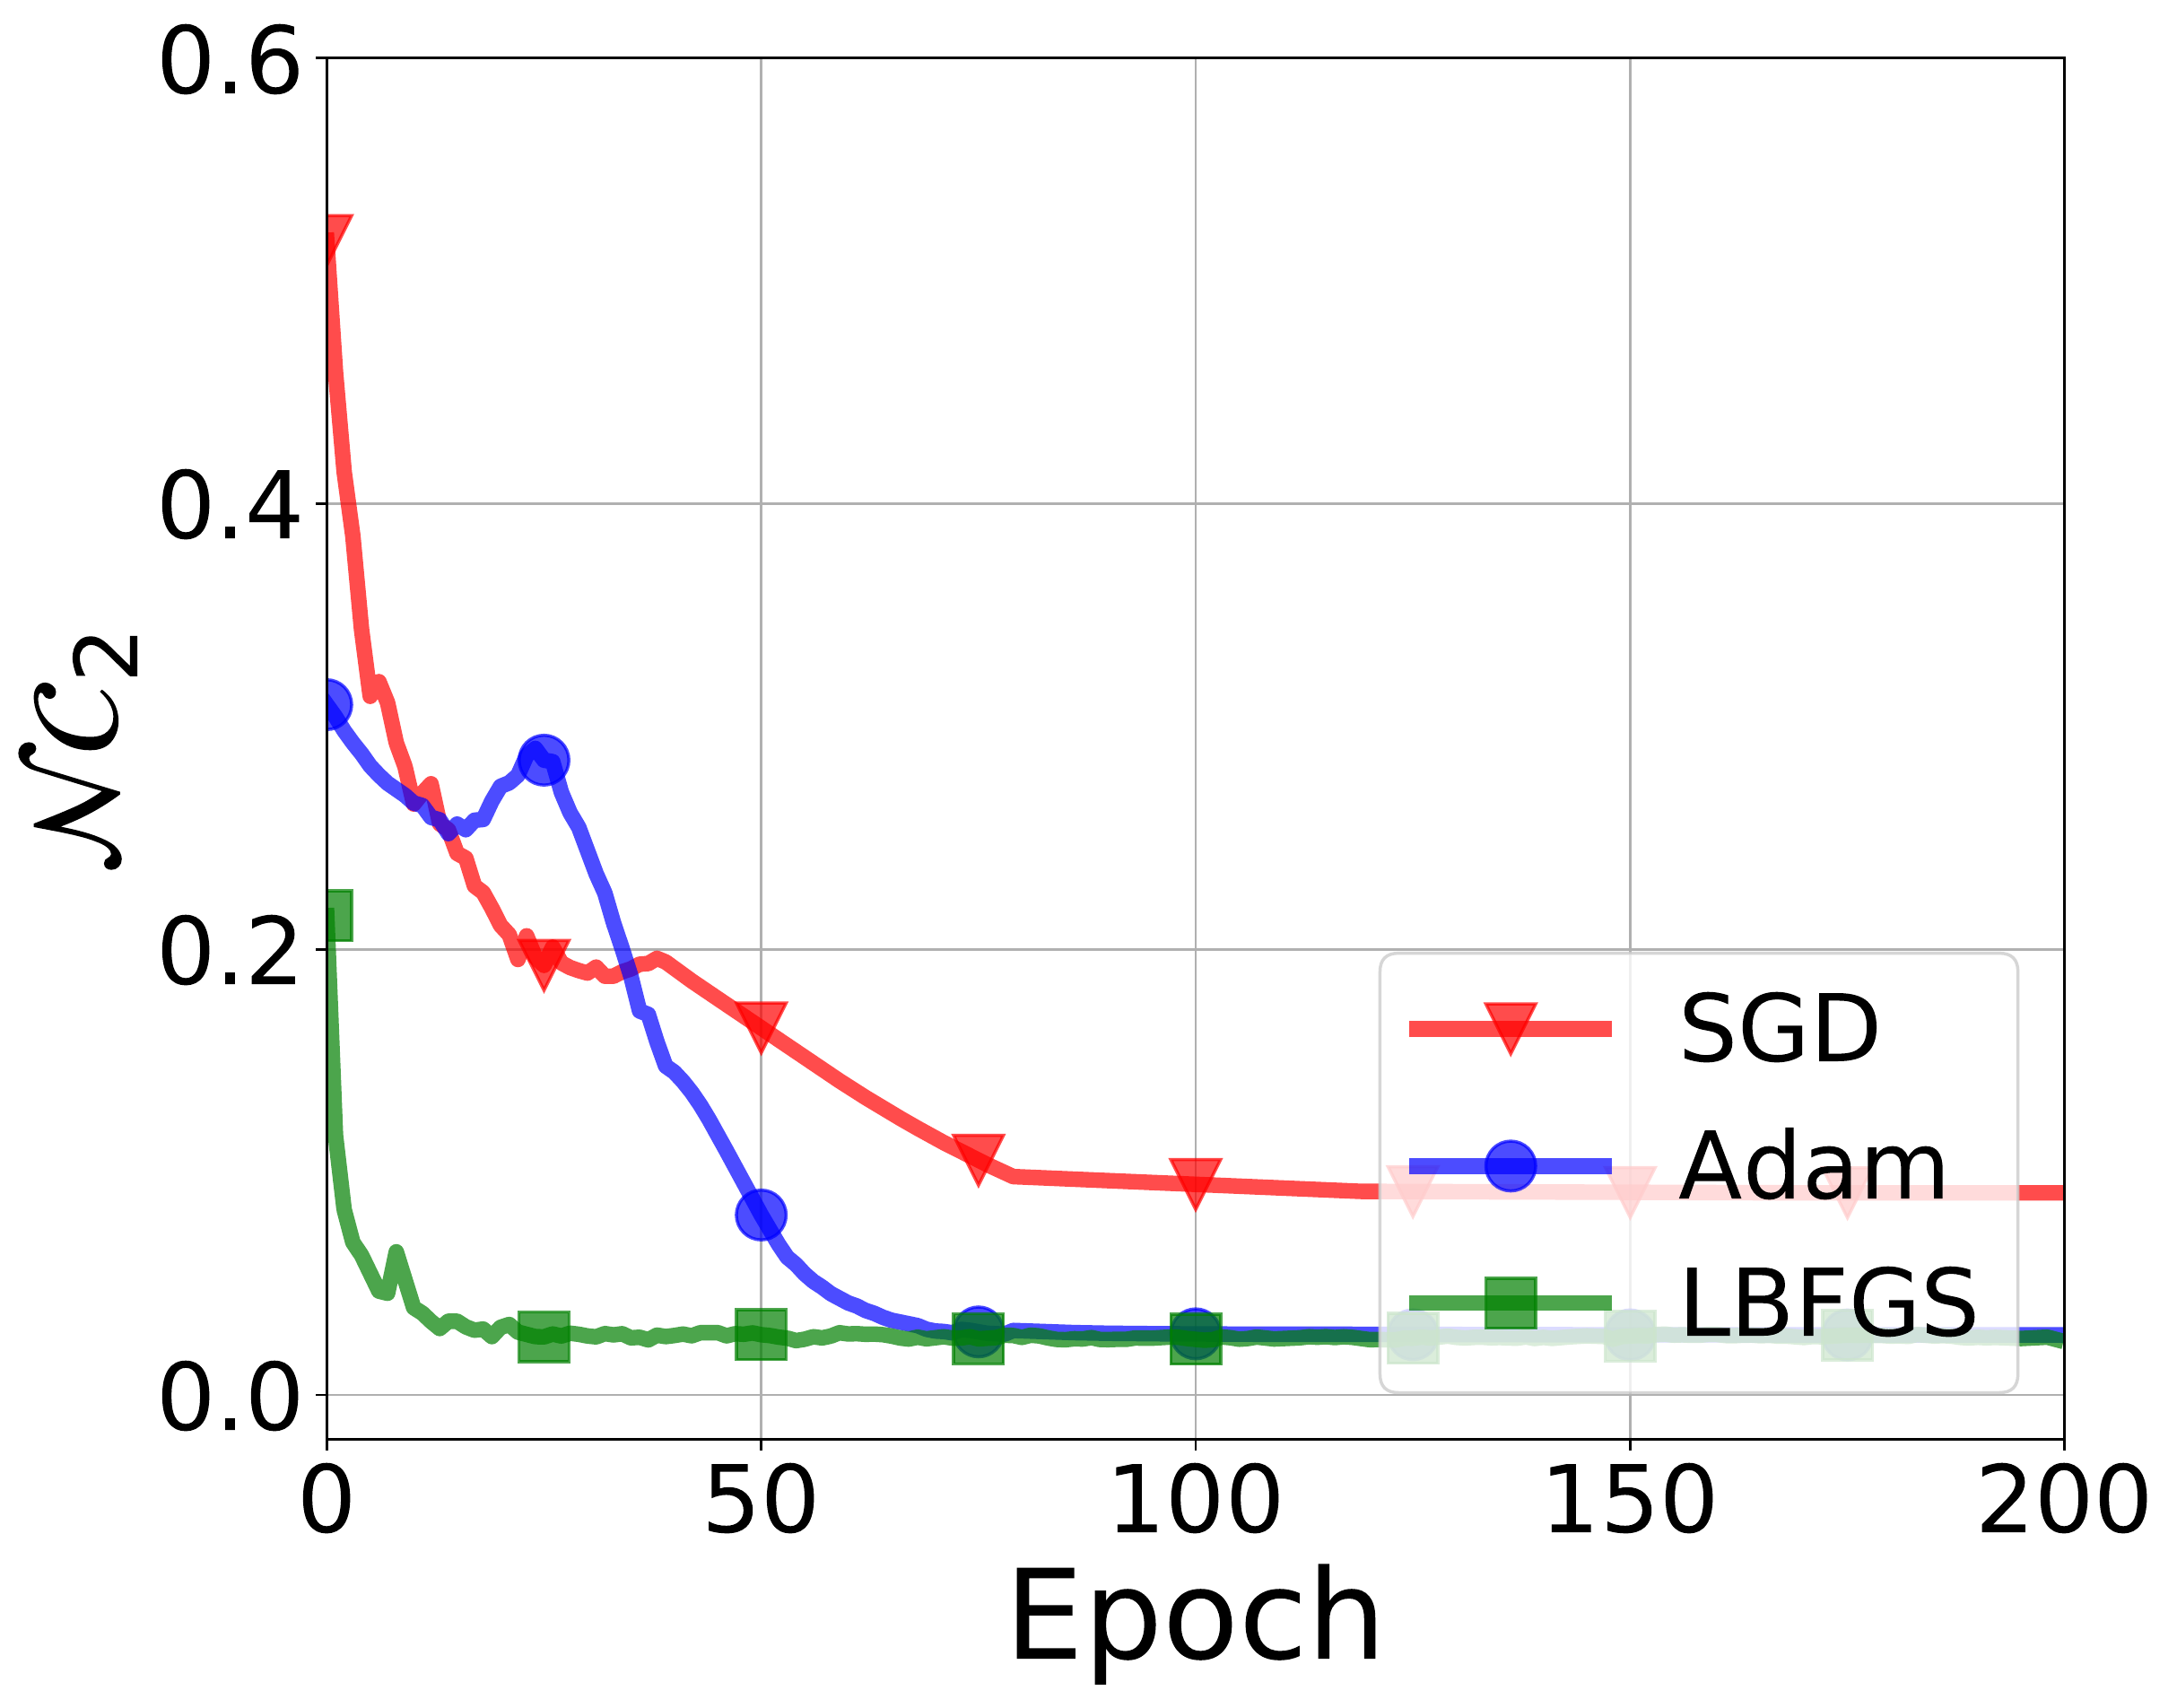}} \
    \subfloat[$\mc {NC}_3$ (MNIST)]{\includegraphics[width=0.24\textwidth]{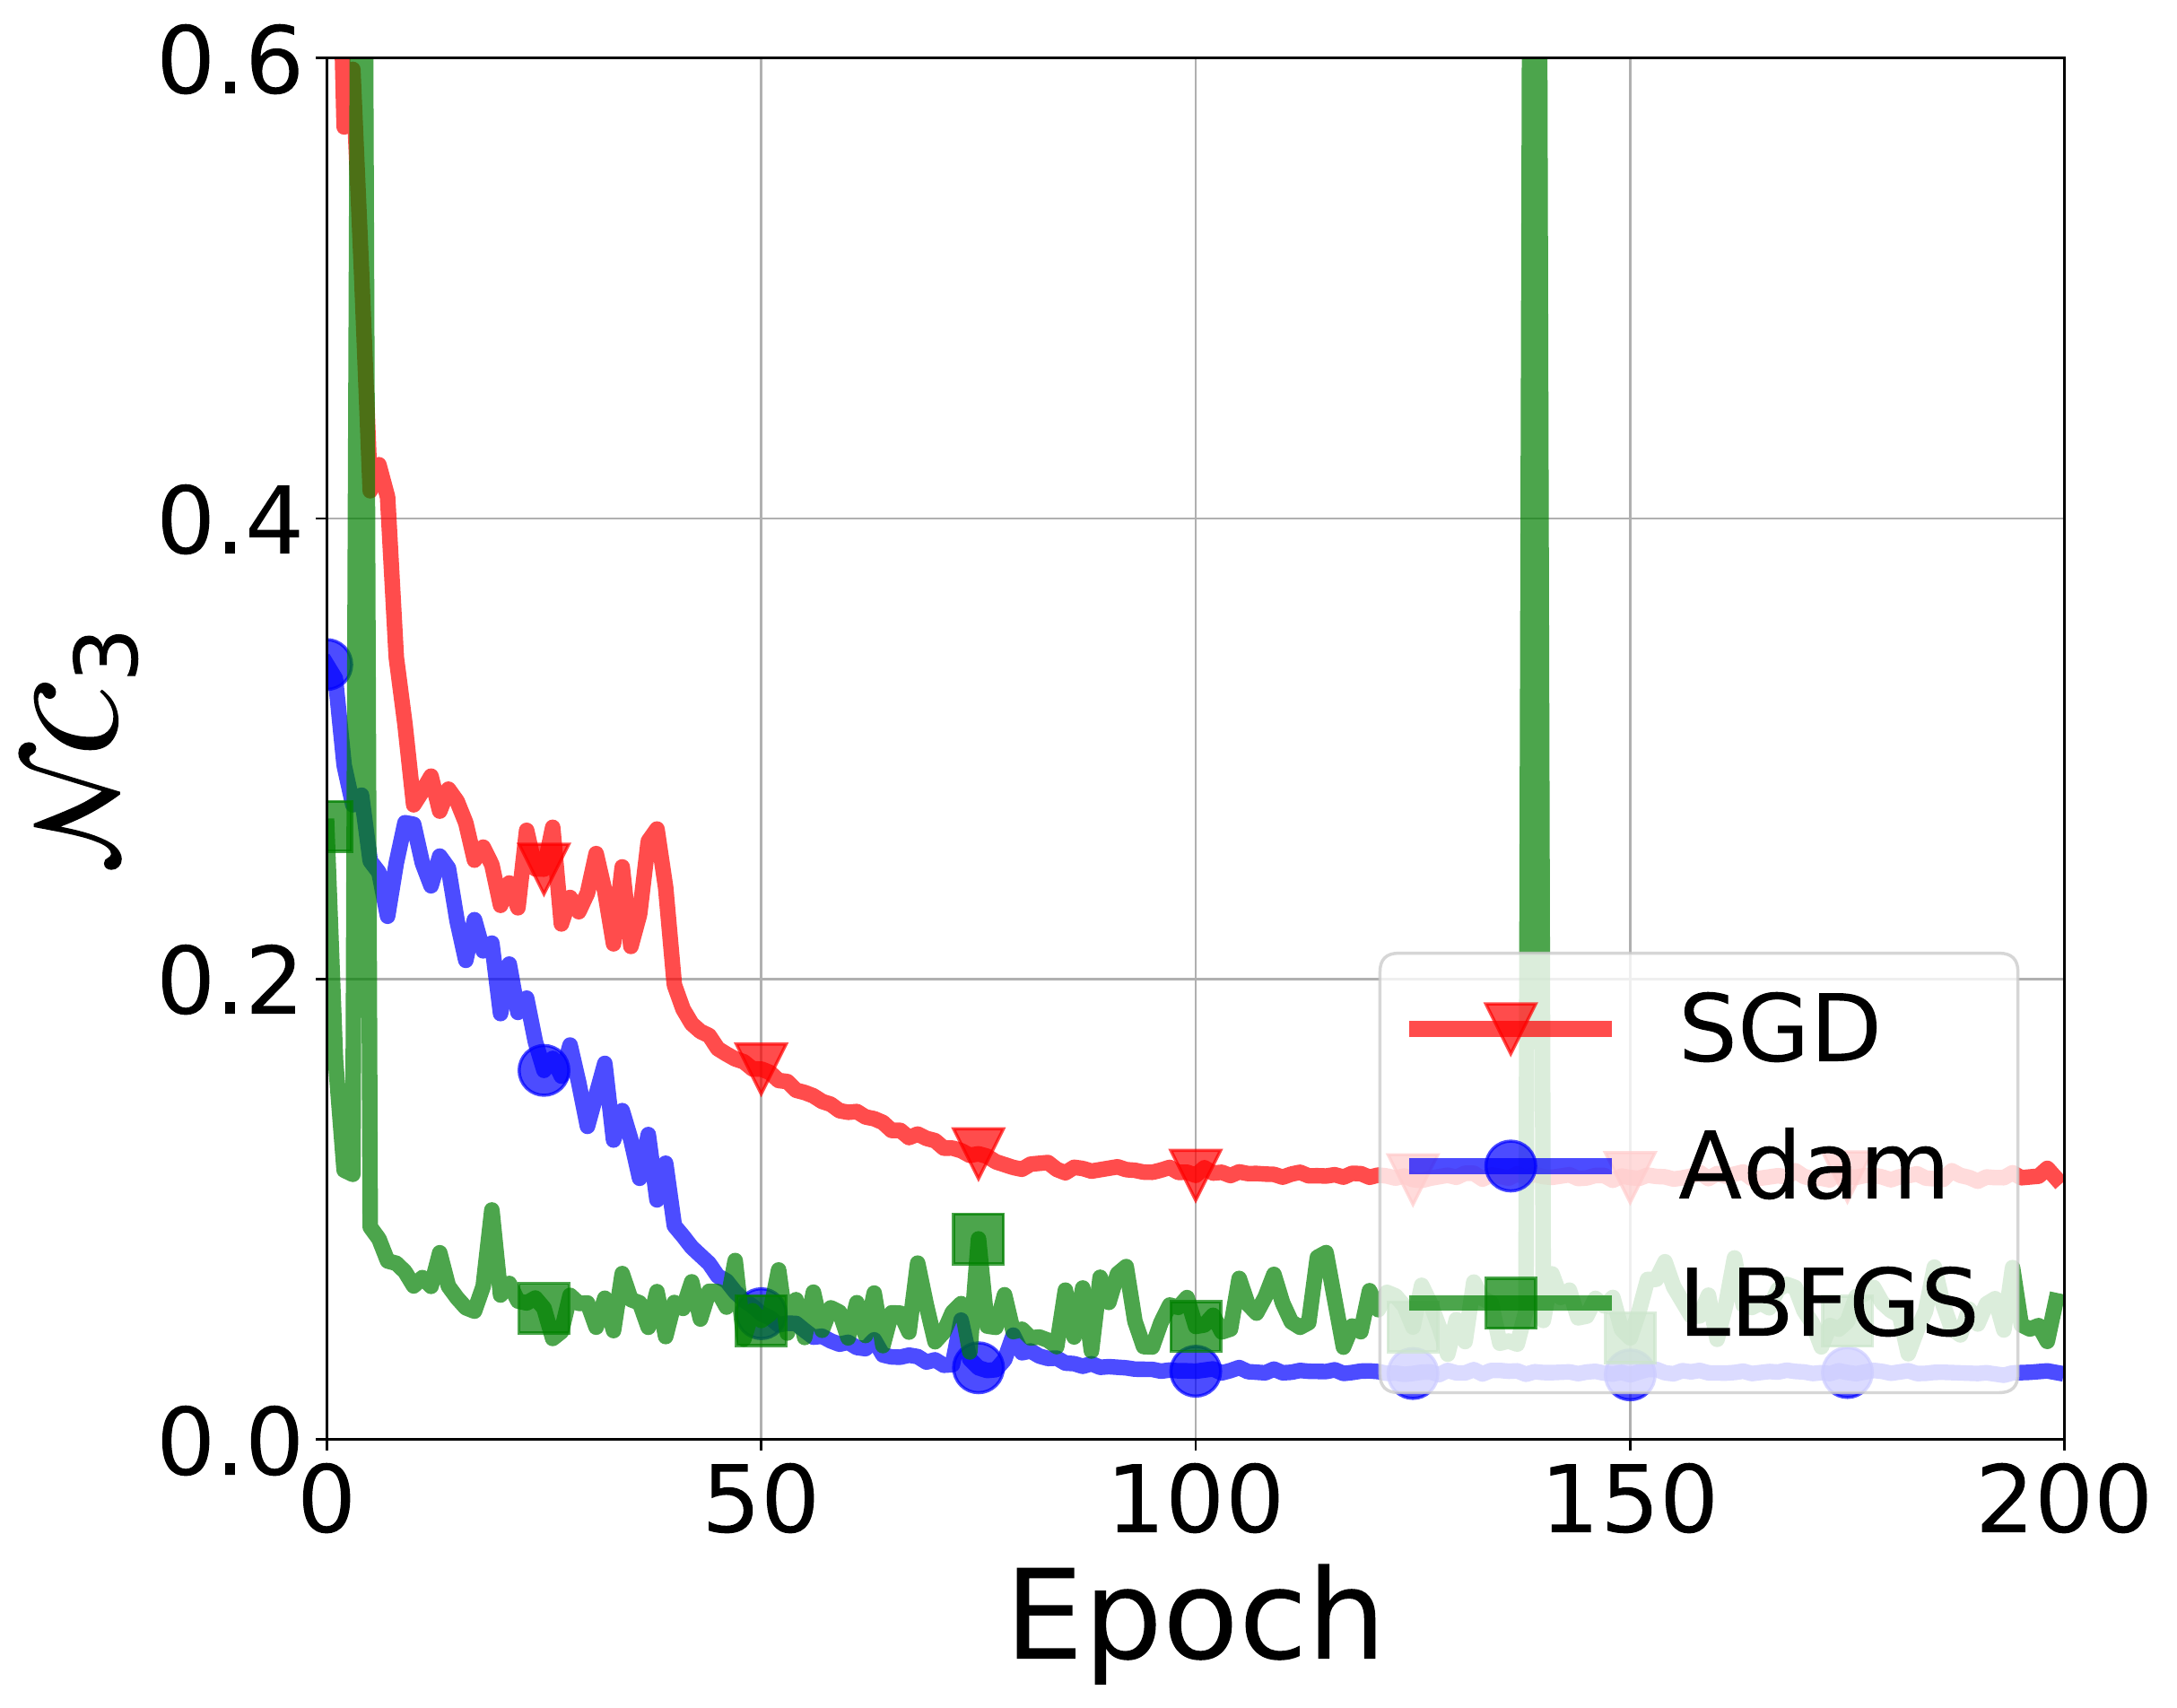}} \
    \subfloat[$\mc {NC}_4$ (MNIST)]{\includegraphics[width=0.24\textwidth]{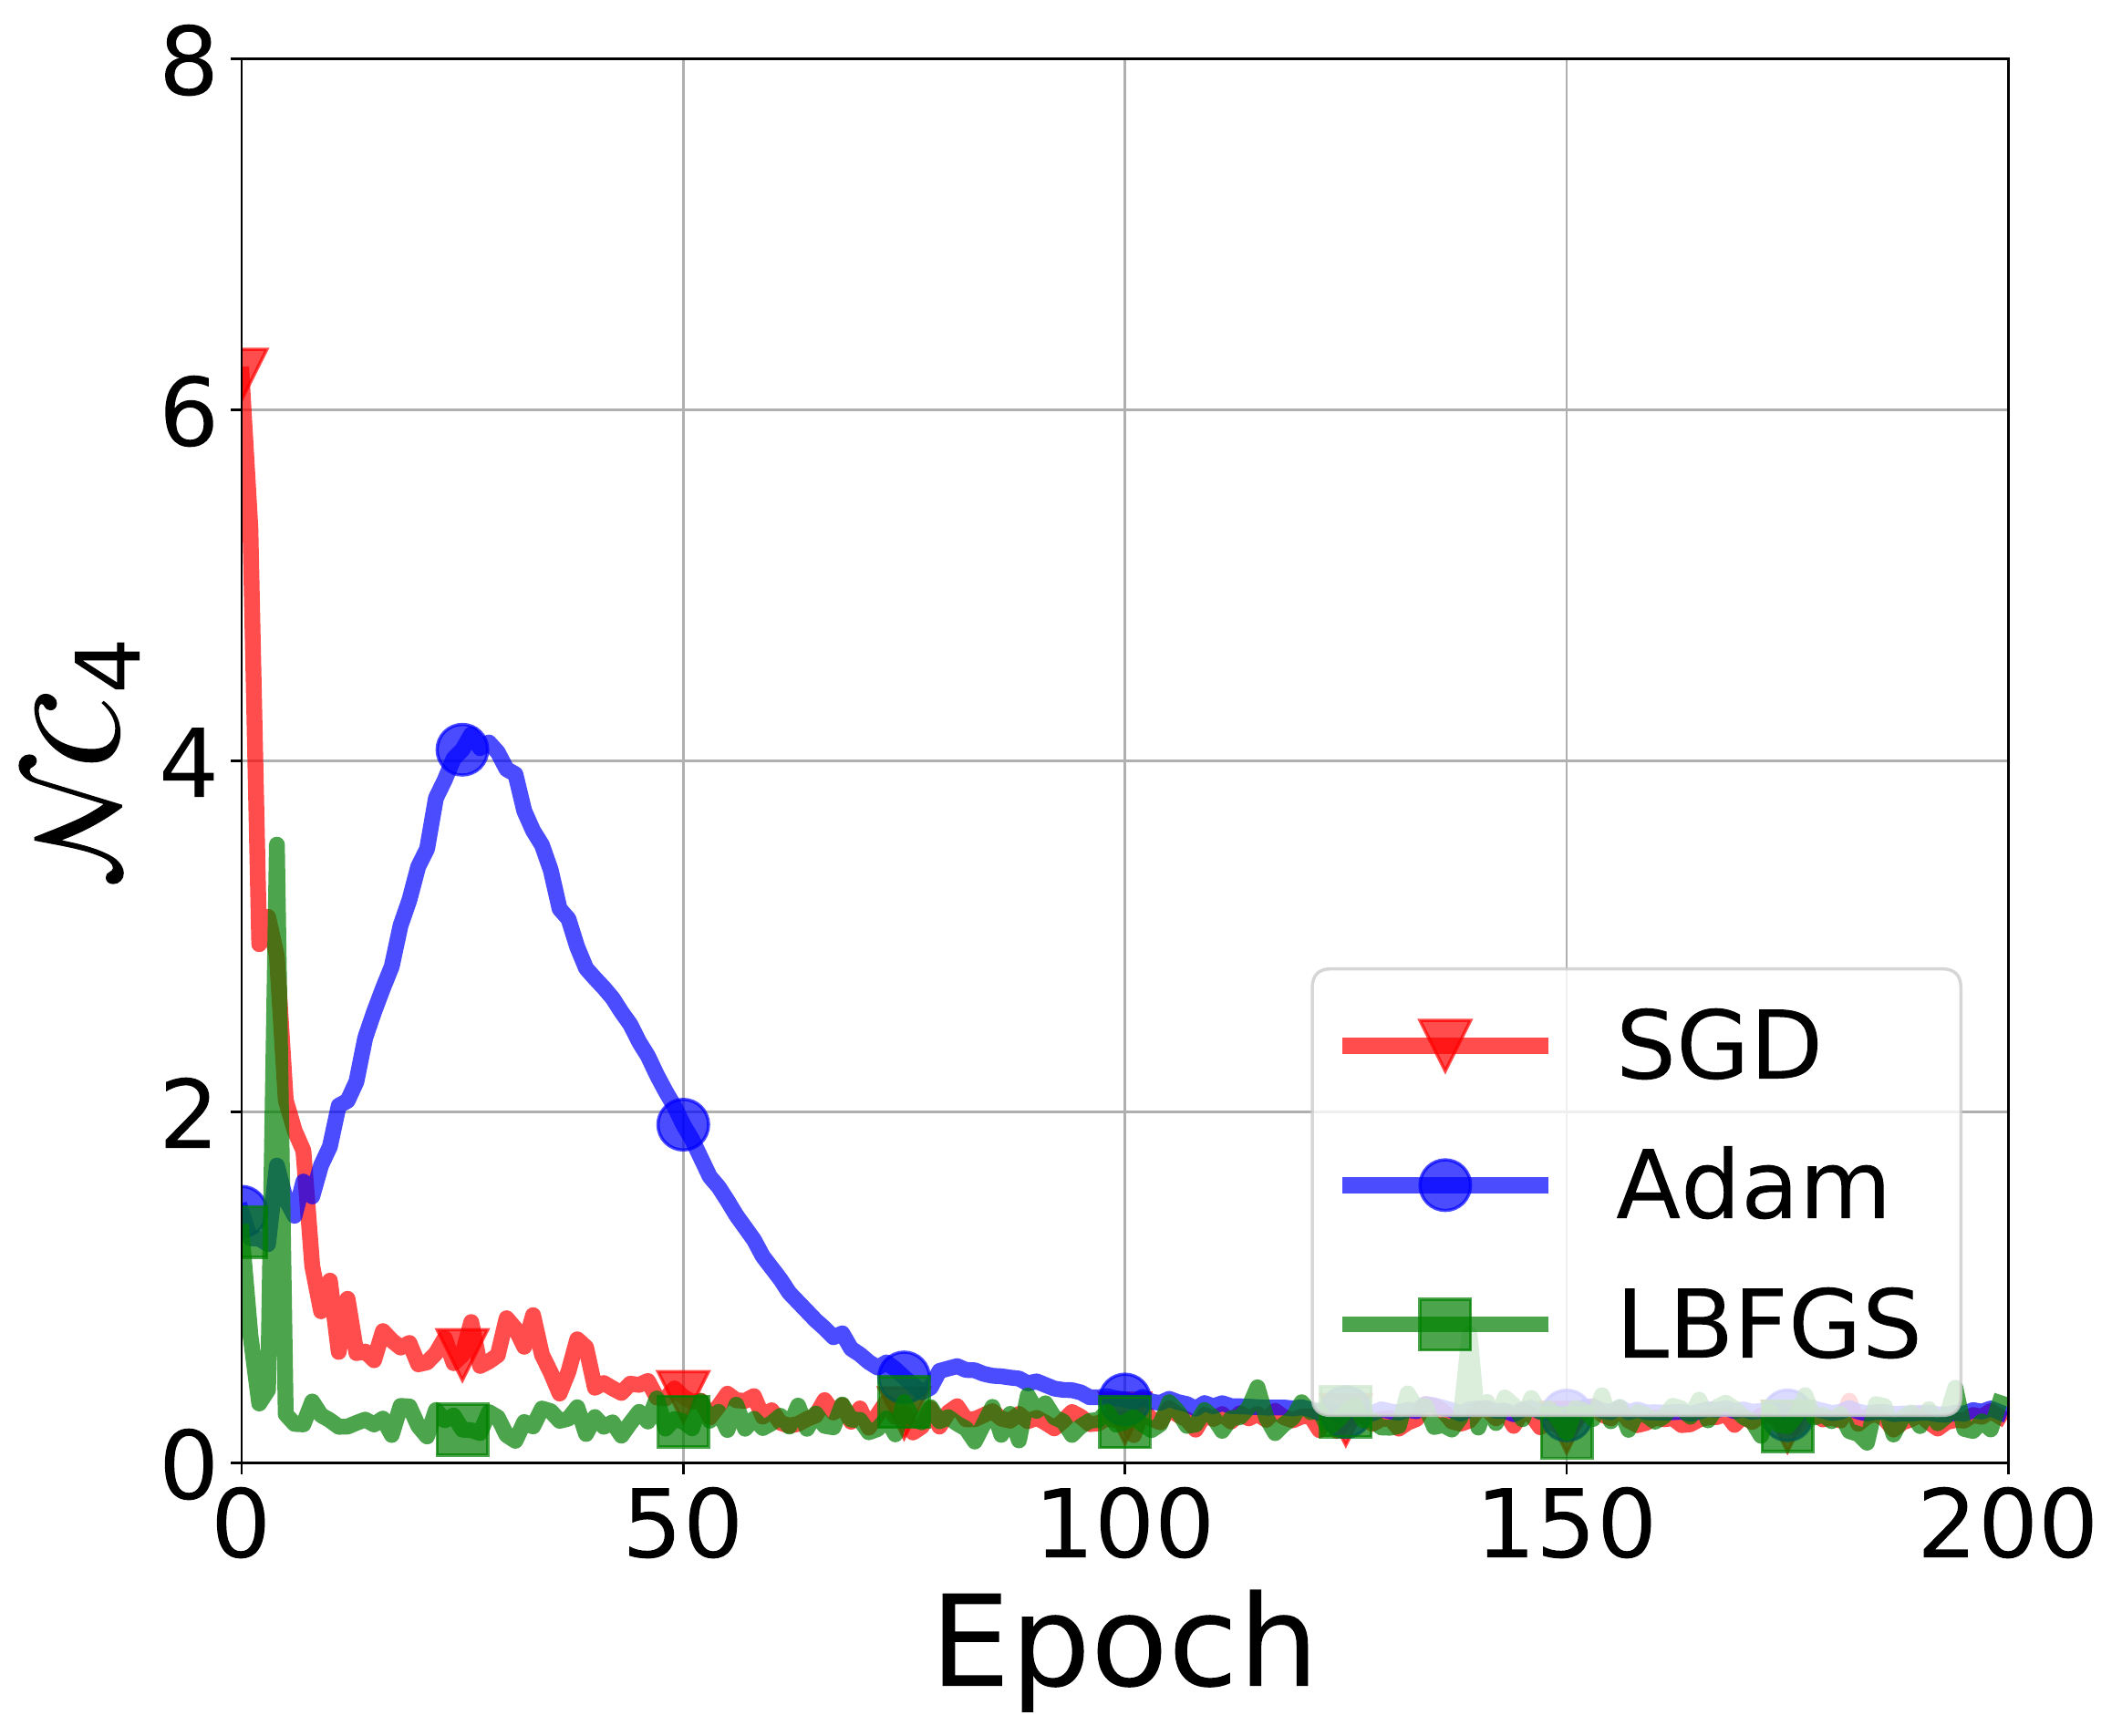}}
    \caption{\textbf{Illustration of \NC\;across different training algorithms} with ResNet18 on MNIST. From the left to the right, the plots show the four metrics, $\mc {NC}_1, \mc {NC}_2, \mc {NC}_3$, and $\mc {NC}_4$, for measuring \NC,  defined in \eqref{eq:NC1}, \eqref{eq:NC2}, \eqref{eq:NC3}, and \eqref{eq:NC4}, respectively. 
    }
    \label{fig:NC-MNIST-CIFAR10-appendix}
\end{figure}

%Our result in \Cref{thm:global-geometry} reveals a benign global landscape for the optimization of neural networks under the unconstrained feature model, which further implies that the prevalence of \NC\ is independent of the choice of particular training methods. In this subsection, we validate our theoretical discovery on modern network architectures and standard datasets. We show different types of training methods (e.g., SGD, Adam, and LBFGS) all achieve \NC\ during the terminal phase of training. 

In \Cref{fig:NC-MNIST-CIFAR10-appendix} and \Cref{fig:Accuracy-MNIST-CIFAR10}, we run all the experiments with ResNet18 on MNIST and CIFAR10 without modification. The results lead to the following observations:
\begin{itemize}[leftmargin=*]
    \item {\textbf{\emph{\NC\;is Algorithm Independent}.}} 
    Similar to \Cref{fig:NC-MNIST-CIFAR10}, we consistently observe from \Cref{fig:NC-MNIST-CIFAR10-appendix} that all four metrics collapse to zero, trained by different types of algorithms -- SGD, Adam, and LBFGS. This implies that \NC\ happens regardless of the choice of training methods. The last-layer features learned by the network are always maximally linearly separable, and correspondingly the last-layer classifier is a perfect linear classifier for the features.
    
  %  These results imply that the last-layer features learned by the network are maximally linearly separable, and the last-layer classifer  the last-layer classifiers of neural networks always converge These results imply that neural networks always converge to a classifier in which the peeled-off layers learn maximally separated features, and the final layer learns a max-margin linear classifier for the learned features.
    %from the first column that the within-class variation collapses, from the second column that the weights of the classifier converge to a Simplex ETF, from the third column that the classifiers converge to the training class-means, and from the forth column that the bias compensates for the global mean of the features. Moreover, such neural collapse phenomena occur for all the three learning algorithms, SGD, Adam and LBFGS. These results illustrate the fact that neural networks always converge to a classifier in which the peeled-off layers learn maximally separated features, and the final layer learns a max-margin linear classifier for the learned features.
    \item {\textbf{\emph{Relationship between \NC\;and Generalization.}}} %The results in \Cref{fig:NC-MNIST-CIFAR10} manifest the fact that neural networks always converge to a perfect linear classifier in which the peeled-off layers learn maximally separated features and the final layer learns a maximal margin linear classifier for the learned features.
    \Cref{fig:Accuracy-MNIST-CIFAR10} depicts the learning curves in terms of both the training and test accuracy for all three optimization algorithms (i.e., SGD, Adam, and LBFGS). These experimental results\footnote{Note that here we use the default version of LBFGS in PyTorch. %\zz{Please verify if this is correct}. 
    Other variants of quasi-Newton methods \cite{bollapragada2018progressive,ren2021kronecker} may give different or better generalization performance.} show that different training algorithms learn neural networks with notably different generalization performances, even though all of them exhibit \NC. Since \NC\;is only a characterization of the training data, it does not directly translate to unseen data. As the network is highly overparameterized, there are infinitely many networks that produce the same $\mb H$ with \NC\ for a particular training dataset, but with different generalization performance. This suggests that study generalization needs to consider the algorithmic bias and the learned weights for the feature $\mb H$. A thorough investigation between \NC\; and generalization is the subject of future work.
    %Therefore, the universality of \NC\;actually shows that such a phenomenon cannot fully explain network generalization. A pertinent study of generalization will necessarily require a scrutiny into the peeled-off layers, where different optimization method imposes different implicit bias on the learned network parameters.
\end{itemize}

%First, we corroborate \Cref{thm:global-geometry} 

%we confirm the \emph{prevalence} of \NC\;in network training, which is independent of 

%Our result in \Cref{thm:global-geometry} reveals a benign global landscape for the optimization of neural networks under the unconstrained feature model. This benign landscape implies that neural collapse is \emph{universal}, in the sense that it occurs not only with gradient descent but also with other local search algorithms in general. %This is in sharp contrast to work on implicit algorithmic bias, which emphasizes the pivotal role of optimization algorithm in determining the solution that the network converges to. In the following experiment, we validate the universality of neural collapse by showing that \NC~ indeed occurs for networks optimized with SGD, Adam and LBFGS. %We first use the original datasets MNIST and CIFAR10 without modification, and we train a ResNet18 with the three different learning algorithms mentioned above. The results lead us to make the following observations:

%\paragraph{True Labels} 

\begin{figure}[t]
    \centering
    \subfloat[MNIST: Training (left) vs. Testing (right)]{\includegraphics[width=0.24\textwidth]{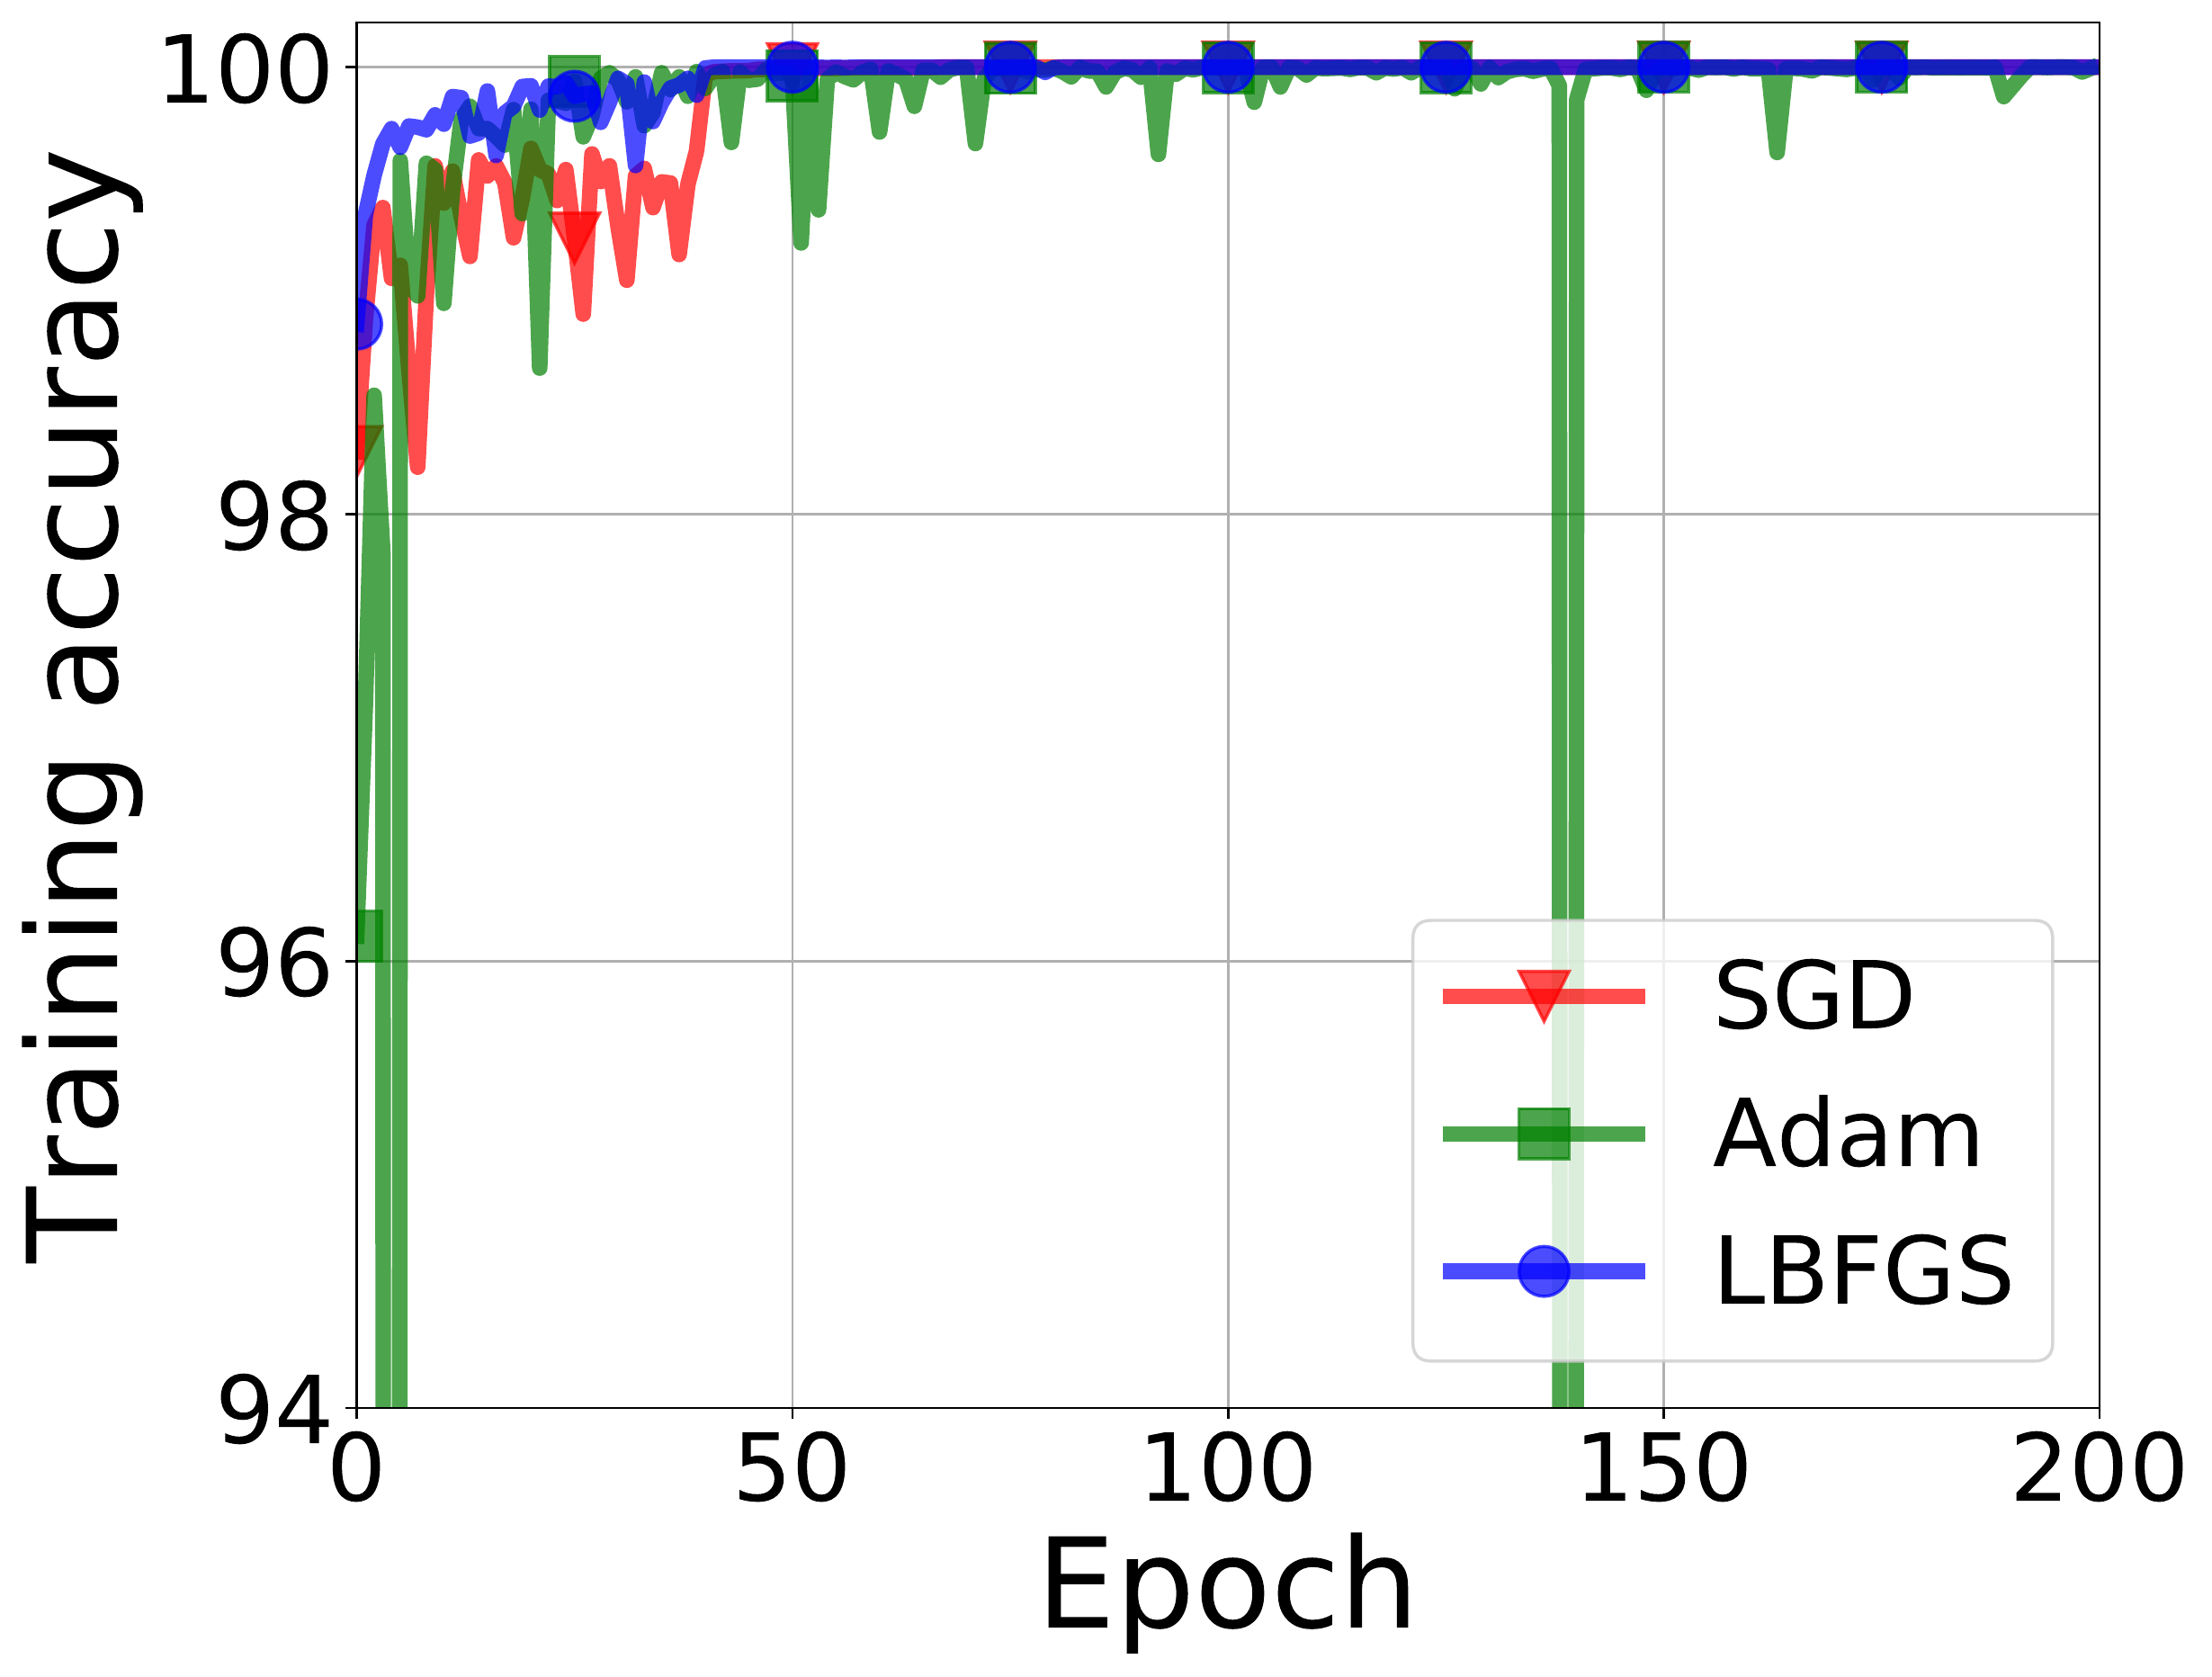} \includegraphics[width=0.24\textwidth]{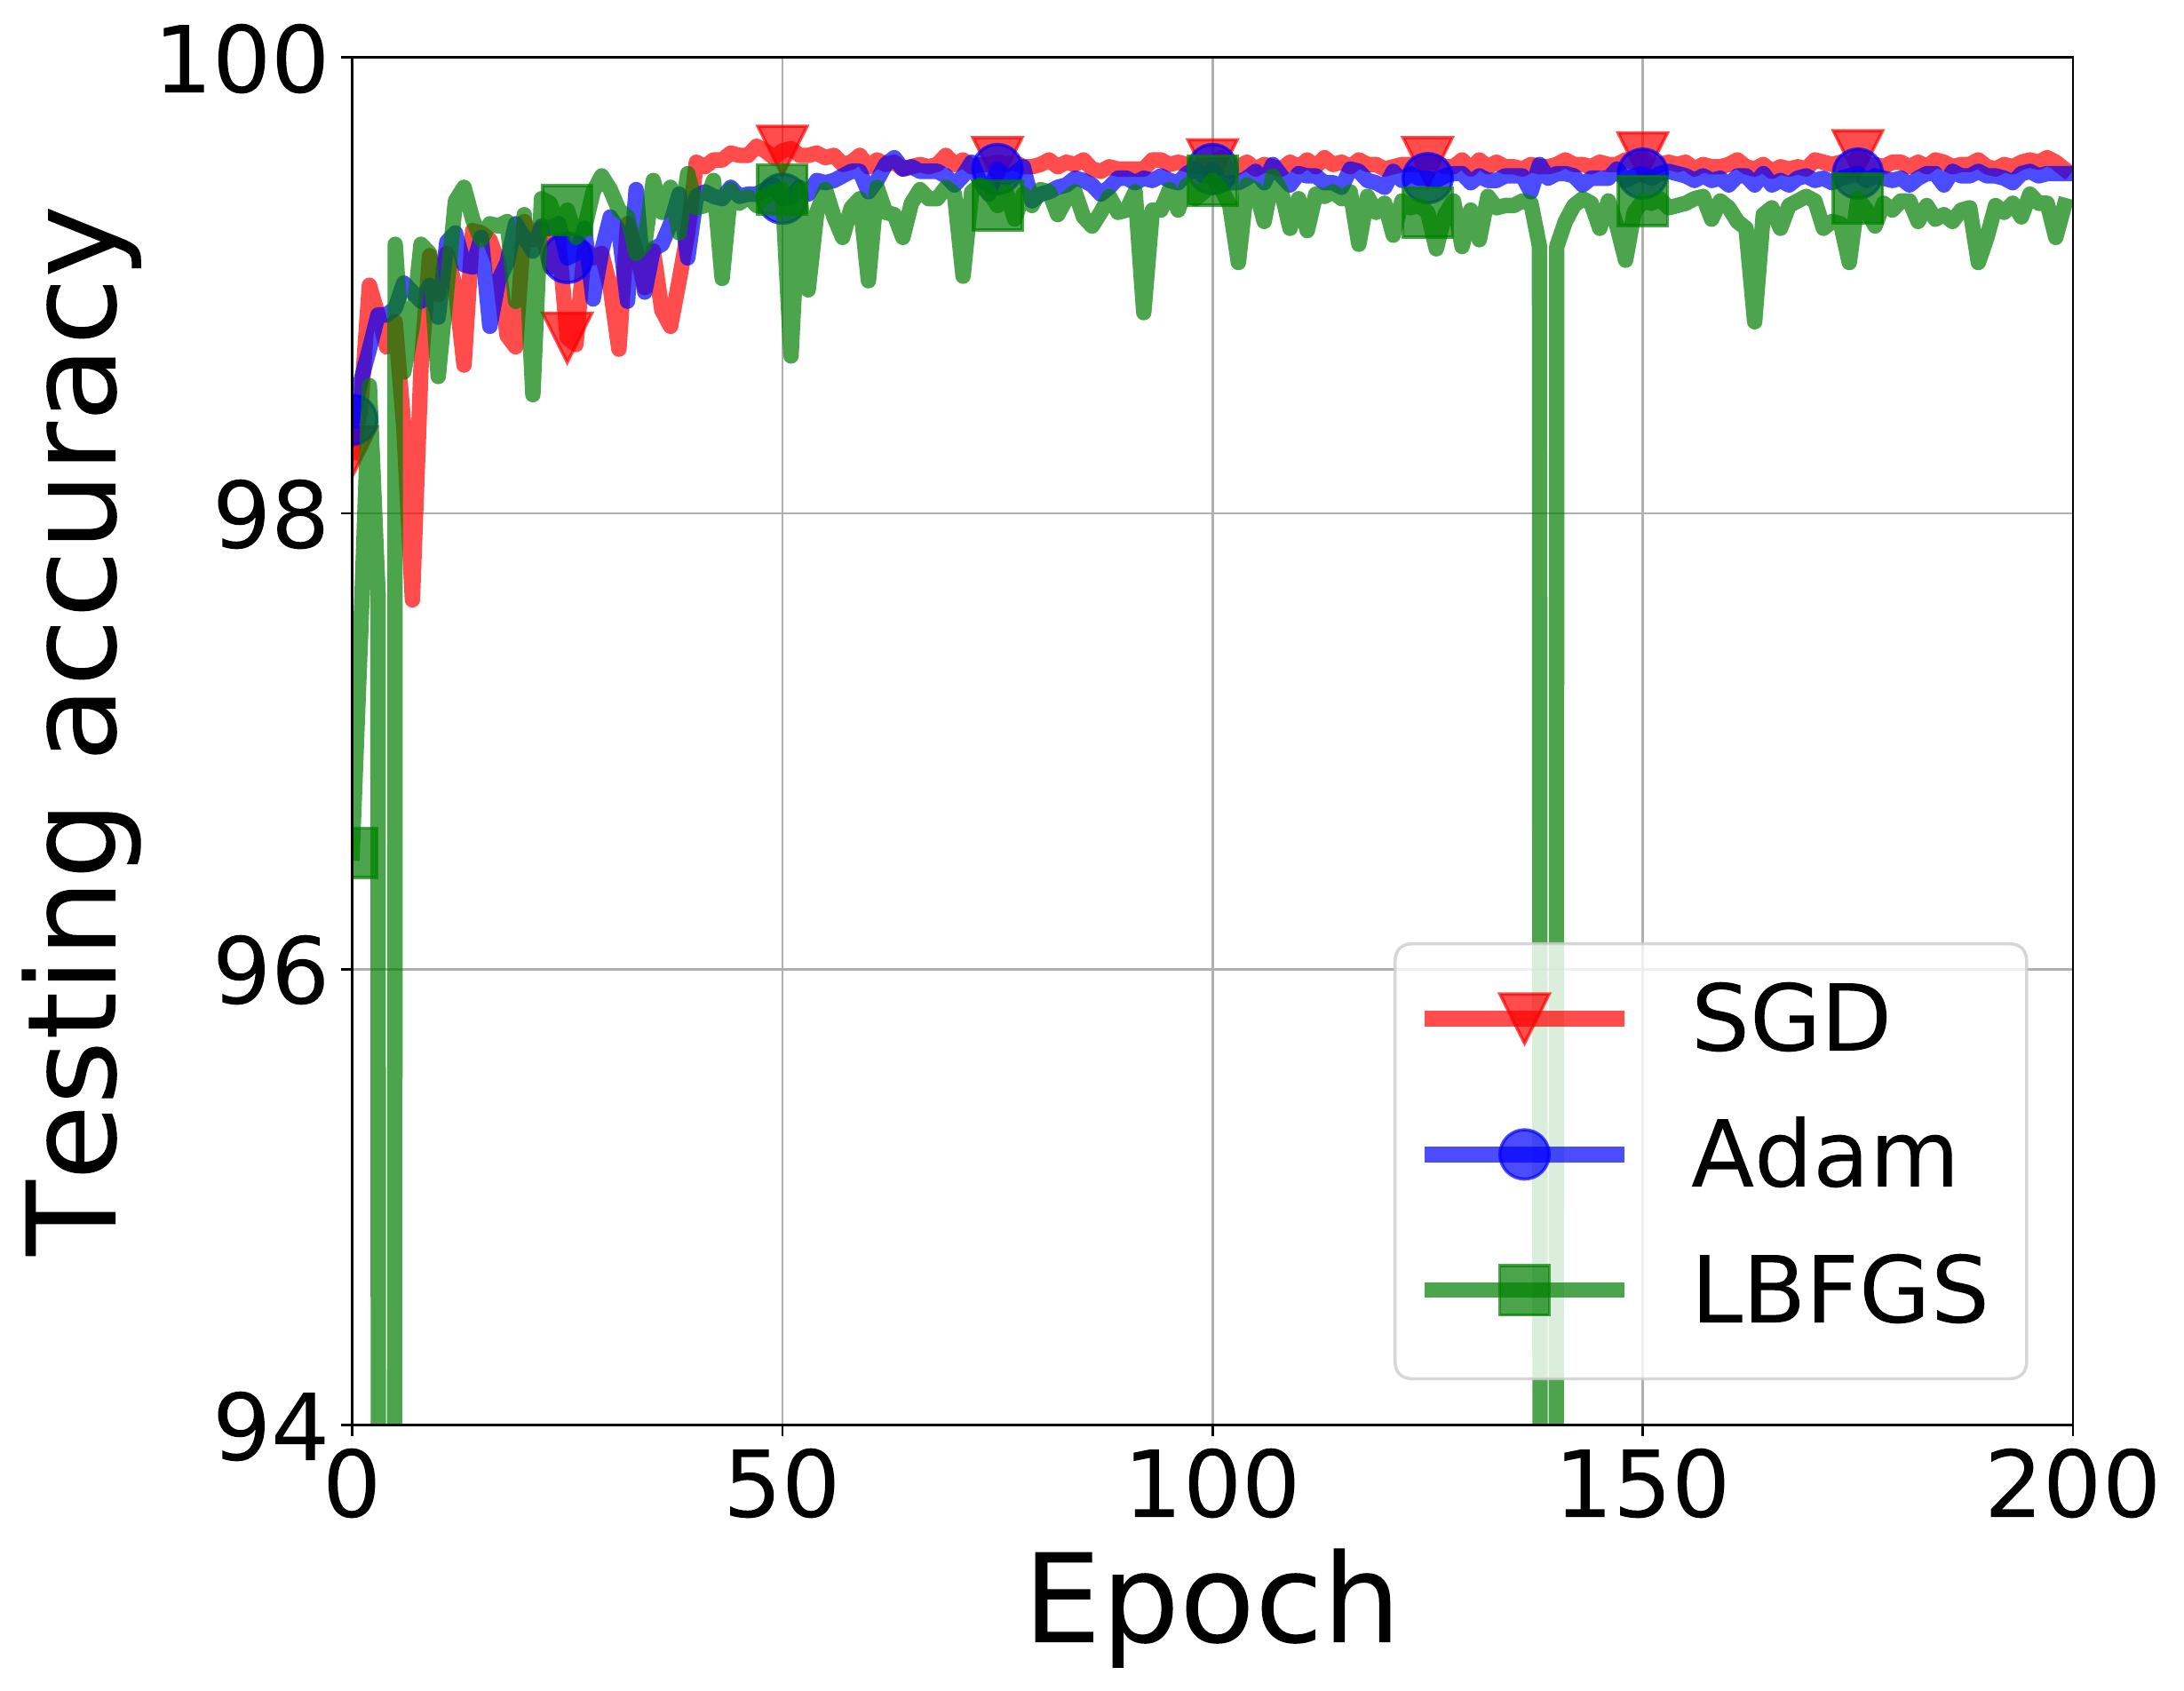}} \
    \subfloat[CIFAR10: Training (left) vs. Testing (right)]{\includegraphics[width=0.24\textwidth]{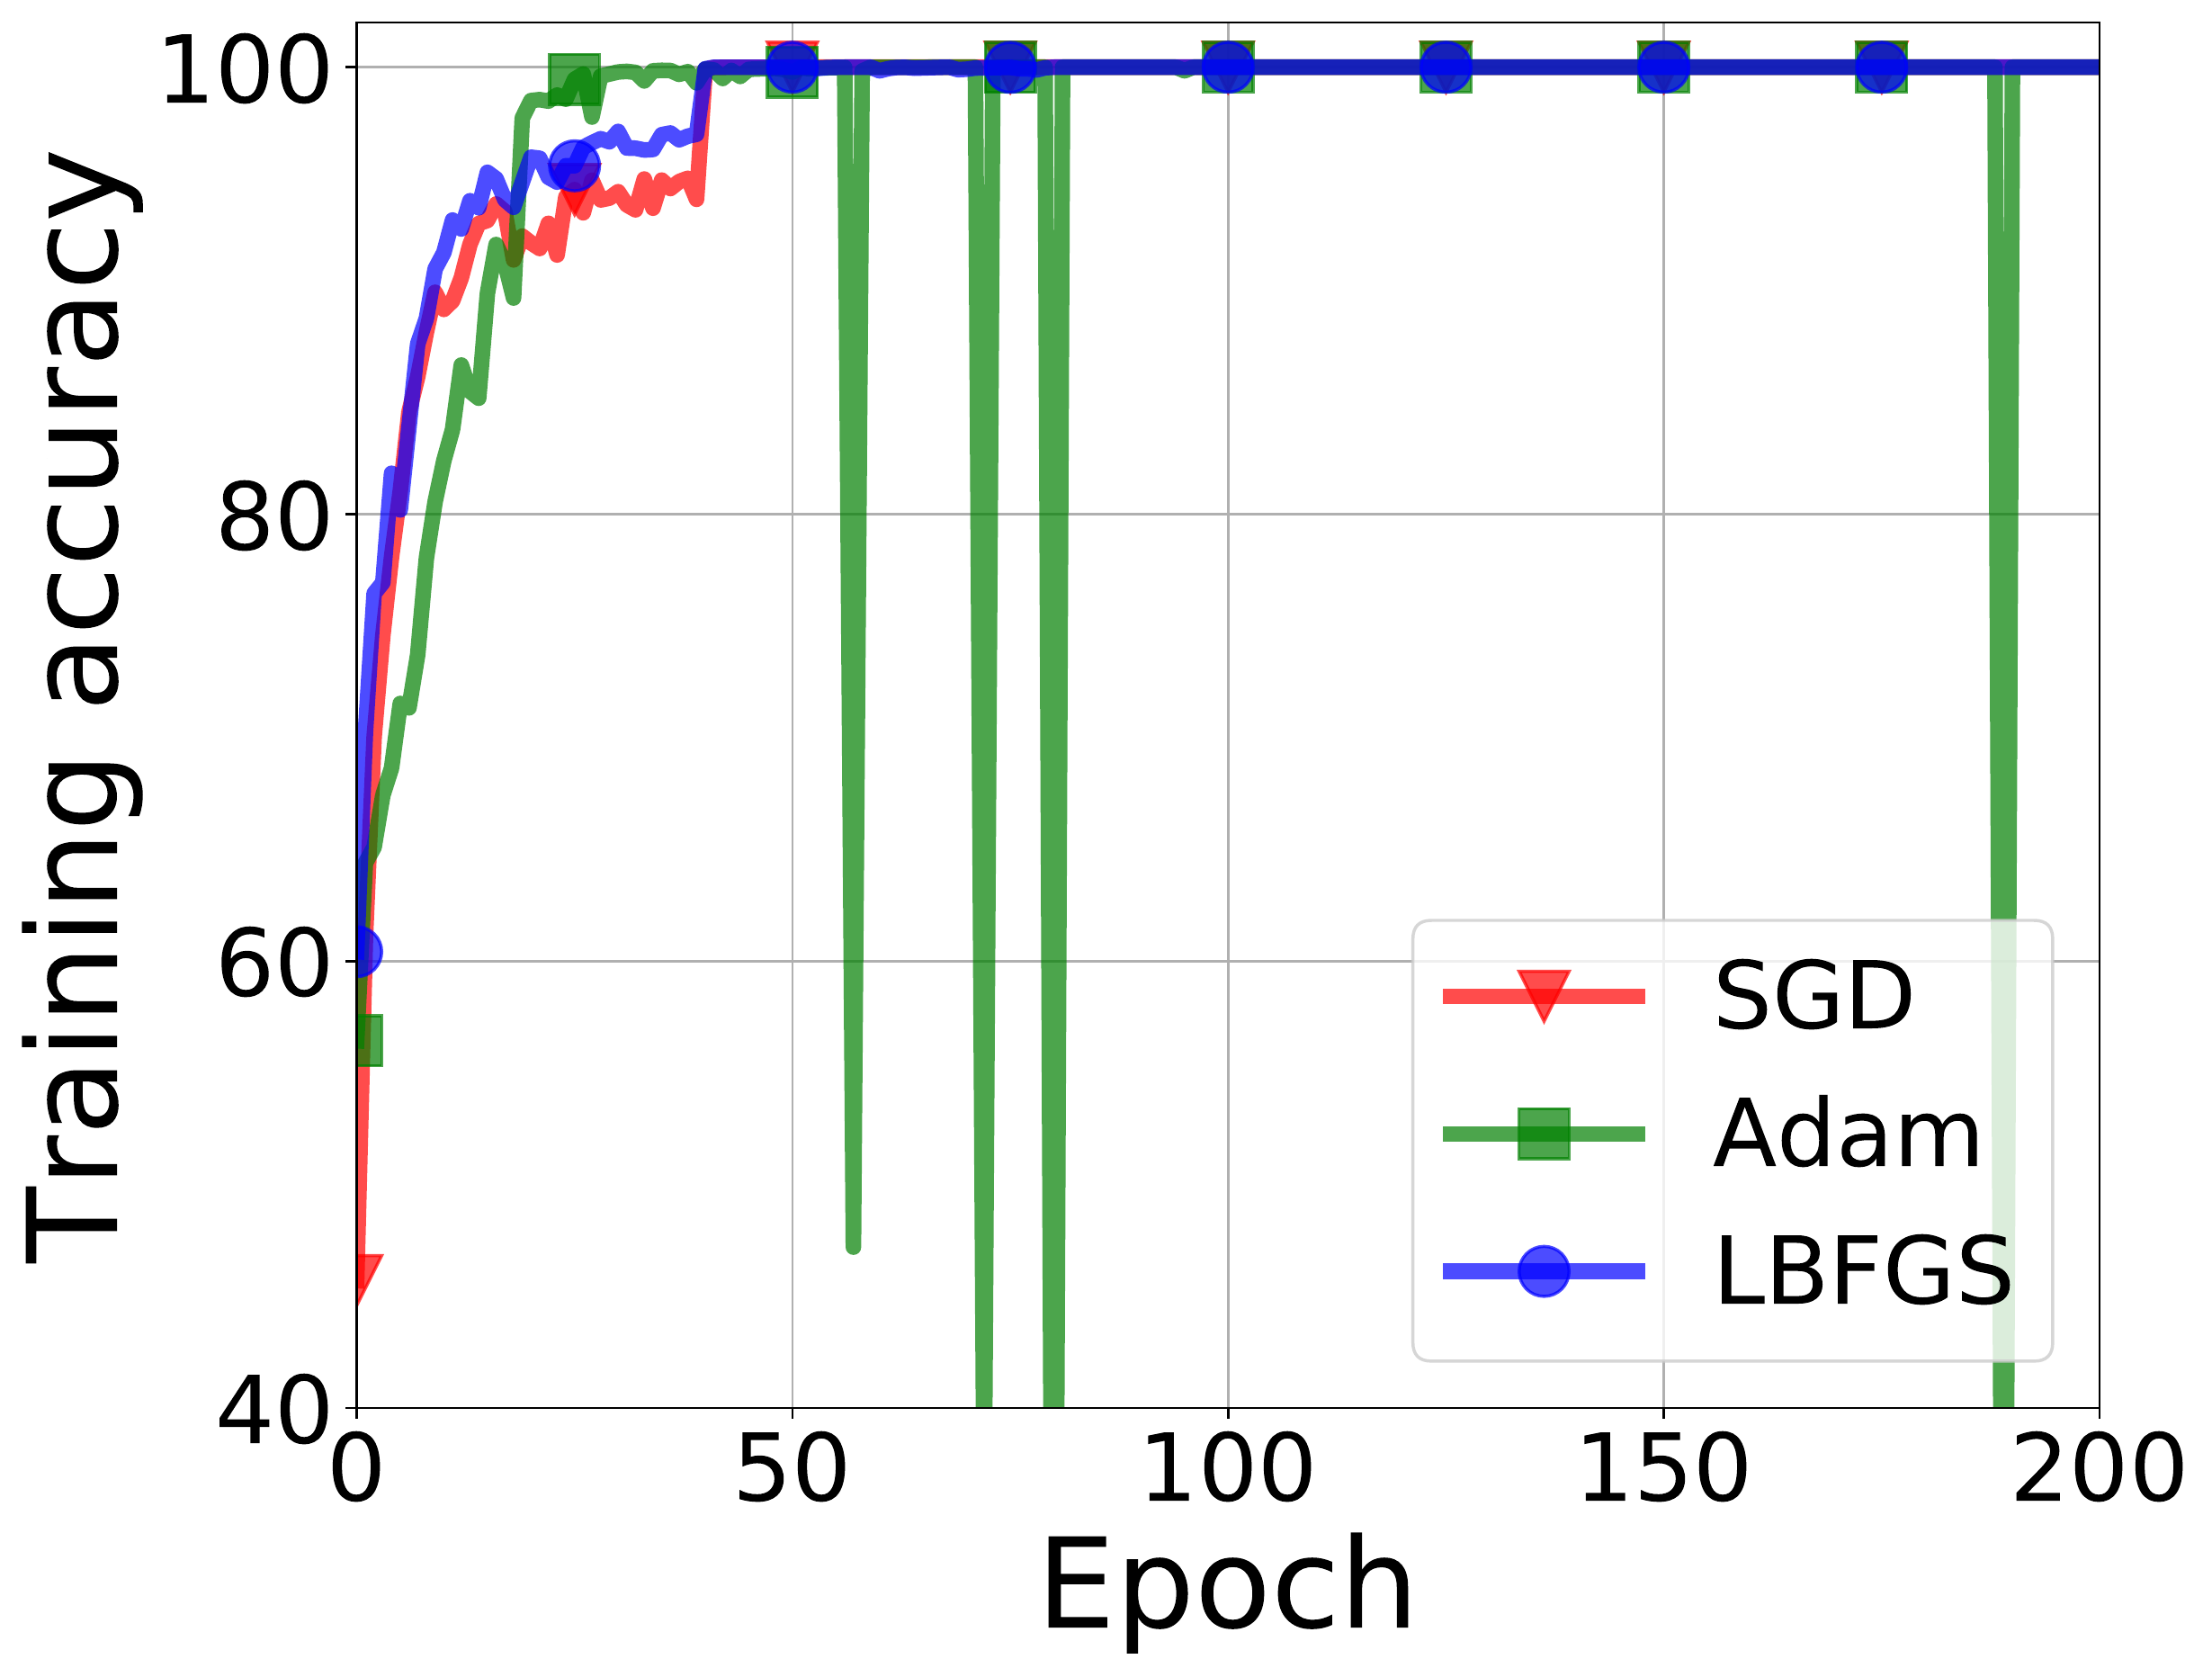}\includegraphics[width=0.24\textwidth]{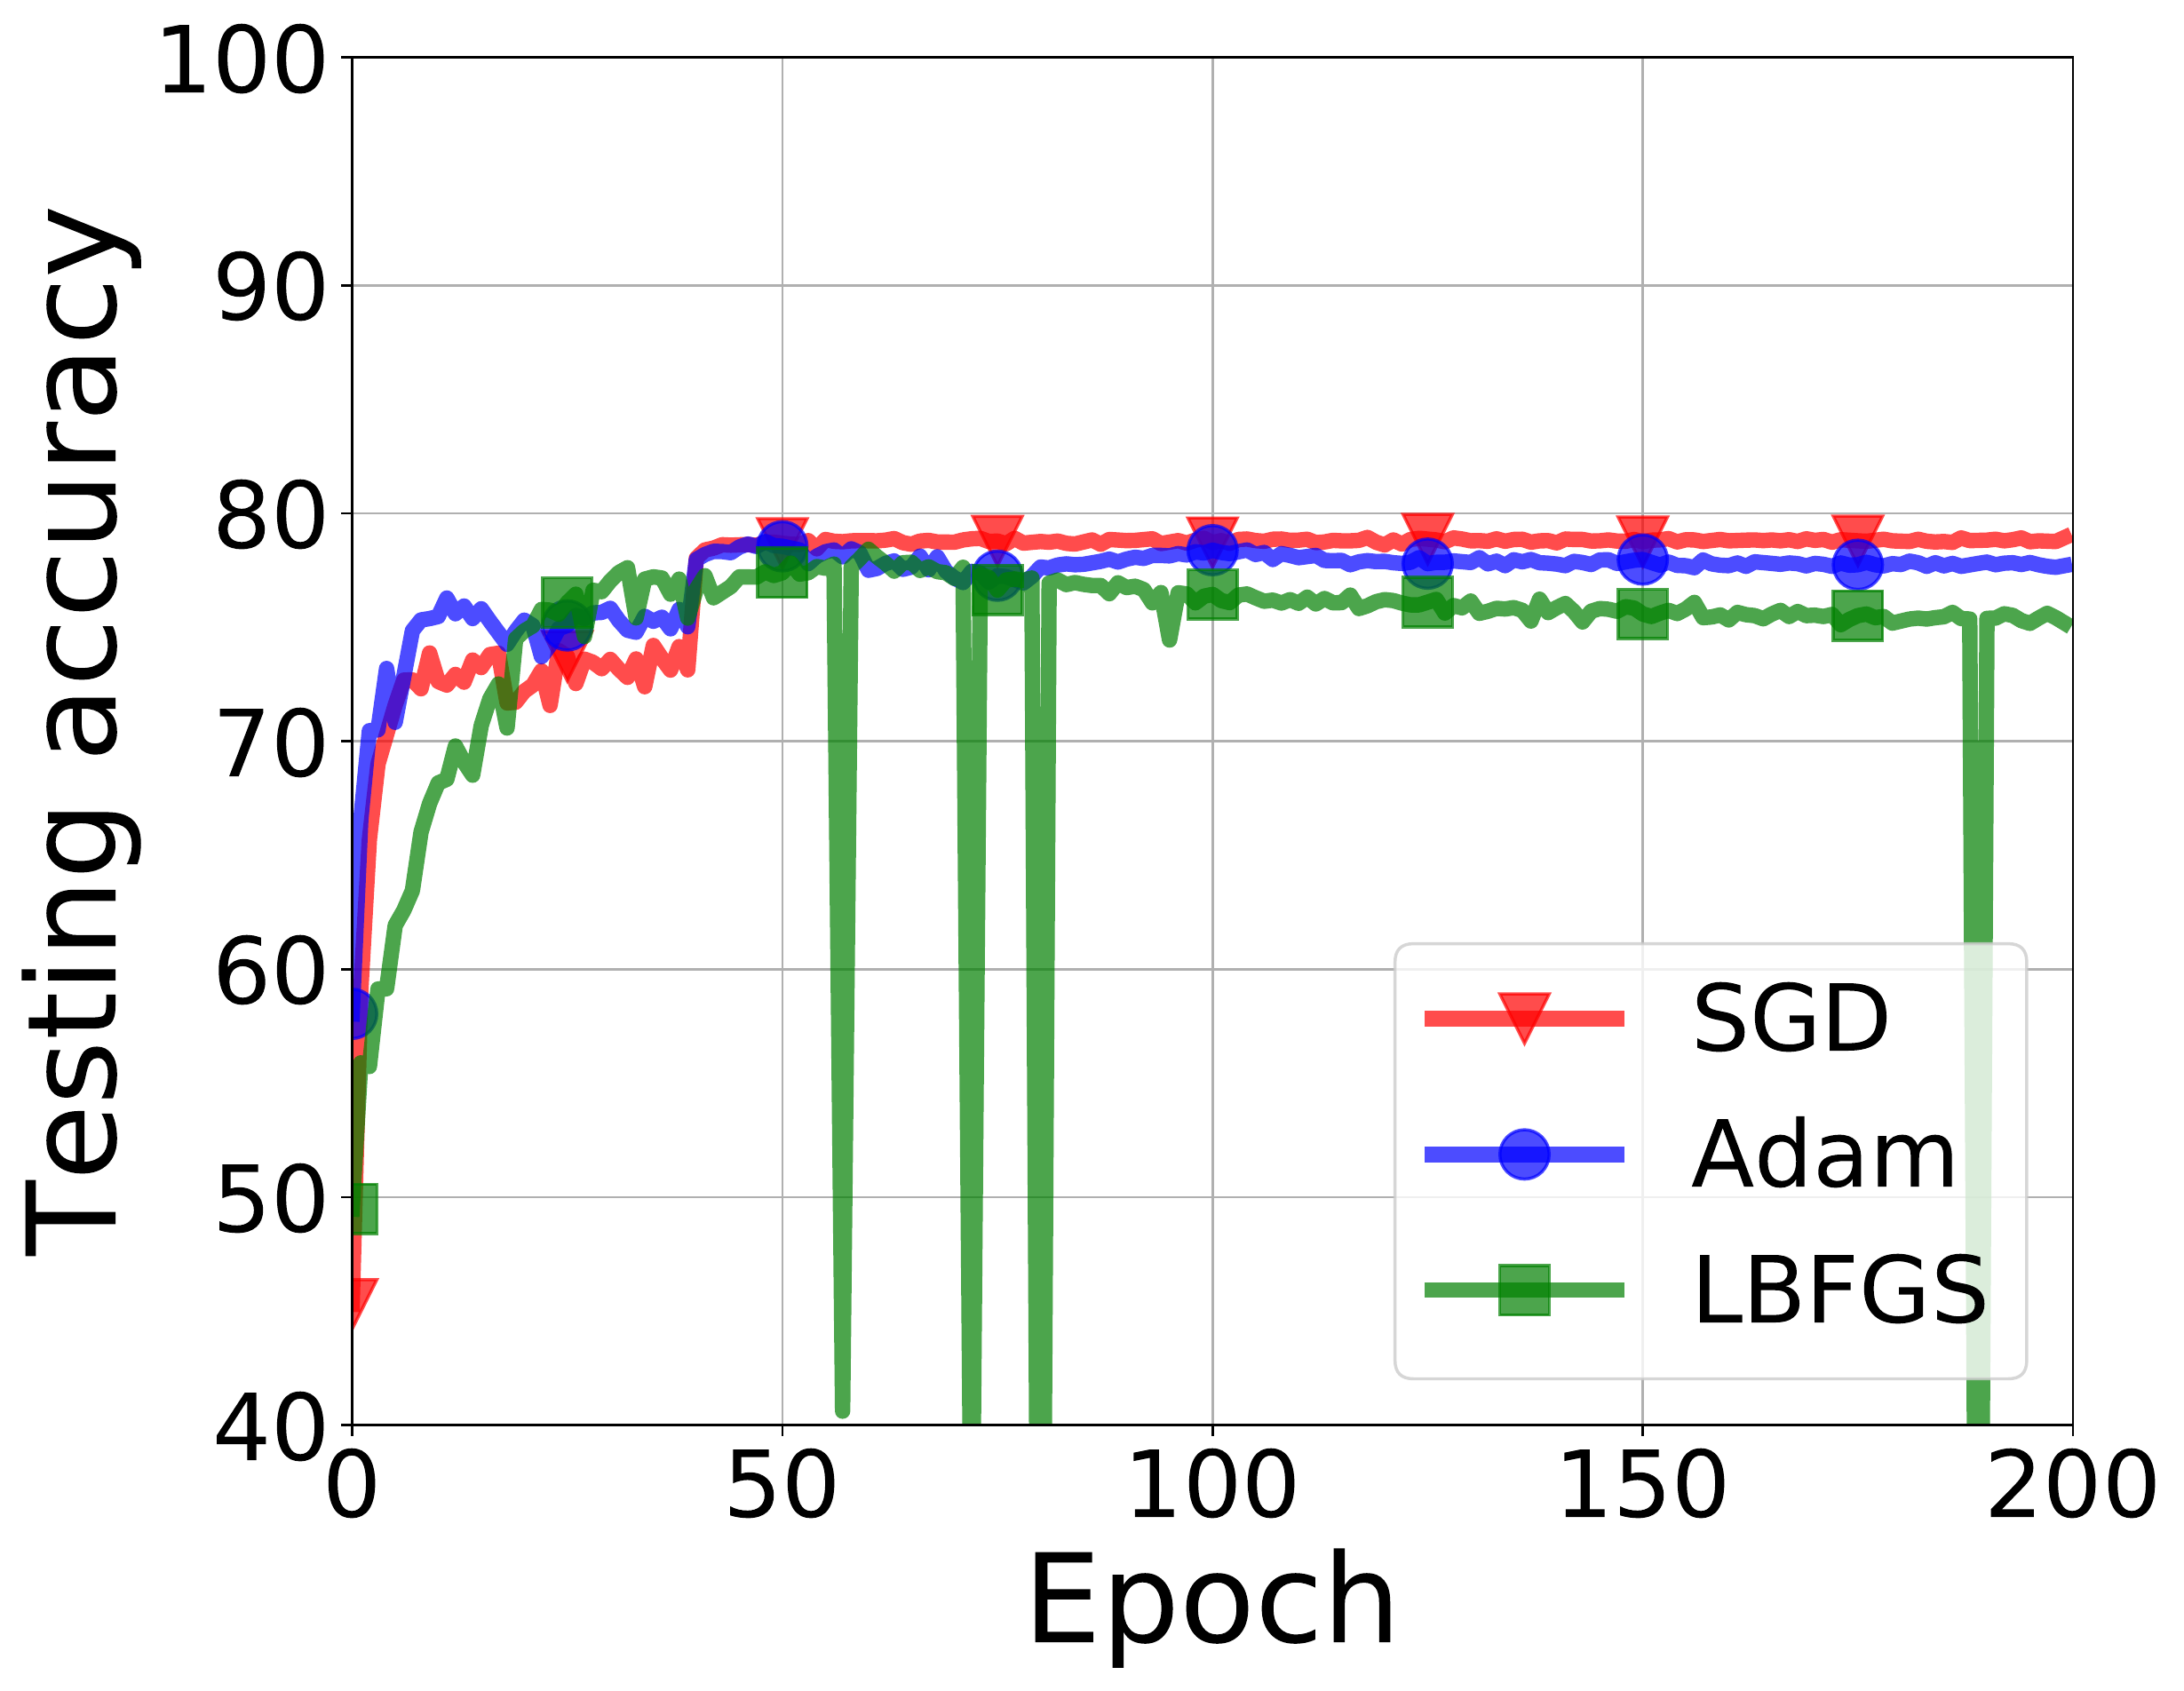}}
    \caption{\textbf{Illustrations of training and test accuracy} for three different training algorithms (i.e., SGD, Adam, and LBFGS) with ResNet18 on MNIST and CIFAR10.  %\zz{Also add the training accuracy to illustrate all the algorithms achieve (almost) zero training error?}
    %\zz{Remove the plot for $Std(b_k)$.}%\zz{Does this case have the ReLu at the end of the penultimate layer? If yes, for the bias term, could you also plot $\|\vb + \mW\valpha\|_2^2$, where $\valpha$ is the global mean of the entire features.}
    }
    \label{fig:Accuracy-MNIST-CIFAR10}
\end{figure}

\subsubsection{The Validity of \eqref{eq:obj} Based on Unconstrained Feature Models for \NC}%\label{subsec:exp-validity}

%\paragraph{Random Labels.} 
The premise of our global landscape analysis of \eqref{eq:obj} for studying \NC\ in deep neural networks is based upon the unconstrained feature model introduced in \Cref{sec:layer-peeled-model}, which simplifies the network by synthesizing the first $L-1$ layers as a universal approximator that generates a simple decision variable for each training sample. Here, we demonstrate through experiments that such a simplification is reasonable for overparameterized networks, at least sufficient for characterizing \NC\ in practical network training.

\paragraph{The Validity of Unconstrained Feature Models.} 
For the ease of studying the effects of model sizes (i.e., overparameterization) on \NC, we also train 4-layer multilayer perceptrons (MLP) of different network width using SGD with learning rate $0.01$ and weight decay $10^{-4}$. We report the corresponding \NC\ behaviors in \Cref{fig:random_label_MLP-appendix}, which shows how training misclassification rate and \NC\ evolve over epochs of training for networks with different widths. \Cref{fig:random_label_MLP-appendix} shows similar results to \Cref{fig:random_label} with ResNet18, in the sense that the training accuracy is highly correlated with \NC\ in the sense that a larger network (i.e., larger width) tends to exhibit severe \NC\ and achieves smaller training error.

\begin{figure}[t]
    \centering
    % \subfloat[$\mc {NC}_1$ (MLP)]{\includegraphics[width=0.24\textwidth]{figs/random_label/rc_collapse_NC1.pdf}} \
    % \subfloat[$\mc {NC}_2$ (MLP)]{\includegraphics[width=0.24\textwidth]{figs/random_label/rc_ETF_NC2.pdf}} \
    % \subfloat[$\mc {NC}_3$ (MLP)]{\includegraphics[width=0.24\textwidth]{figs/random_label/rc_W-H_NC3.pdf}} \
    % \subfloat[Training Error]{\includegraphics[width=0.24\textwidth]{figs/random_label/rc_train_error.pdf}} \\
    \subfloat[Random Label CIFAR10-MLP (from left to right): $\mc {NC}_1$ (log scale), $\mc {NC}_2$, $\mc {NC}_3$, Training Error Rate]
        {\includegraphics[width=0.24\textwidth]{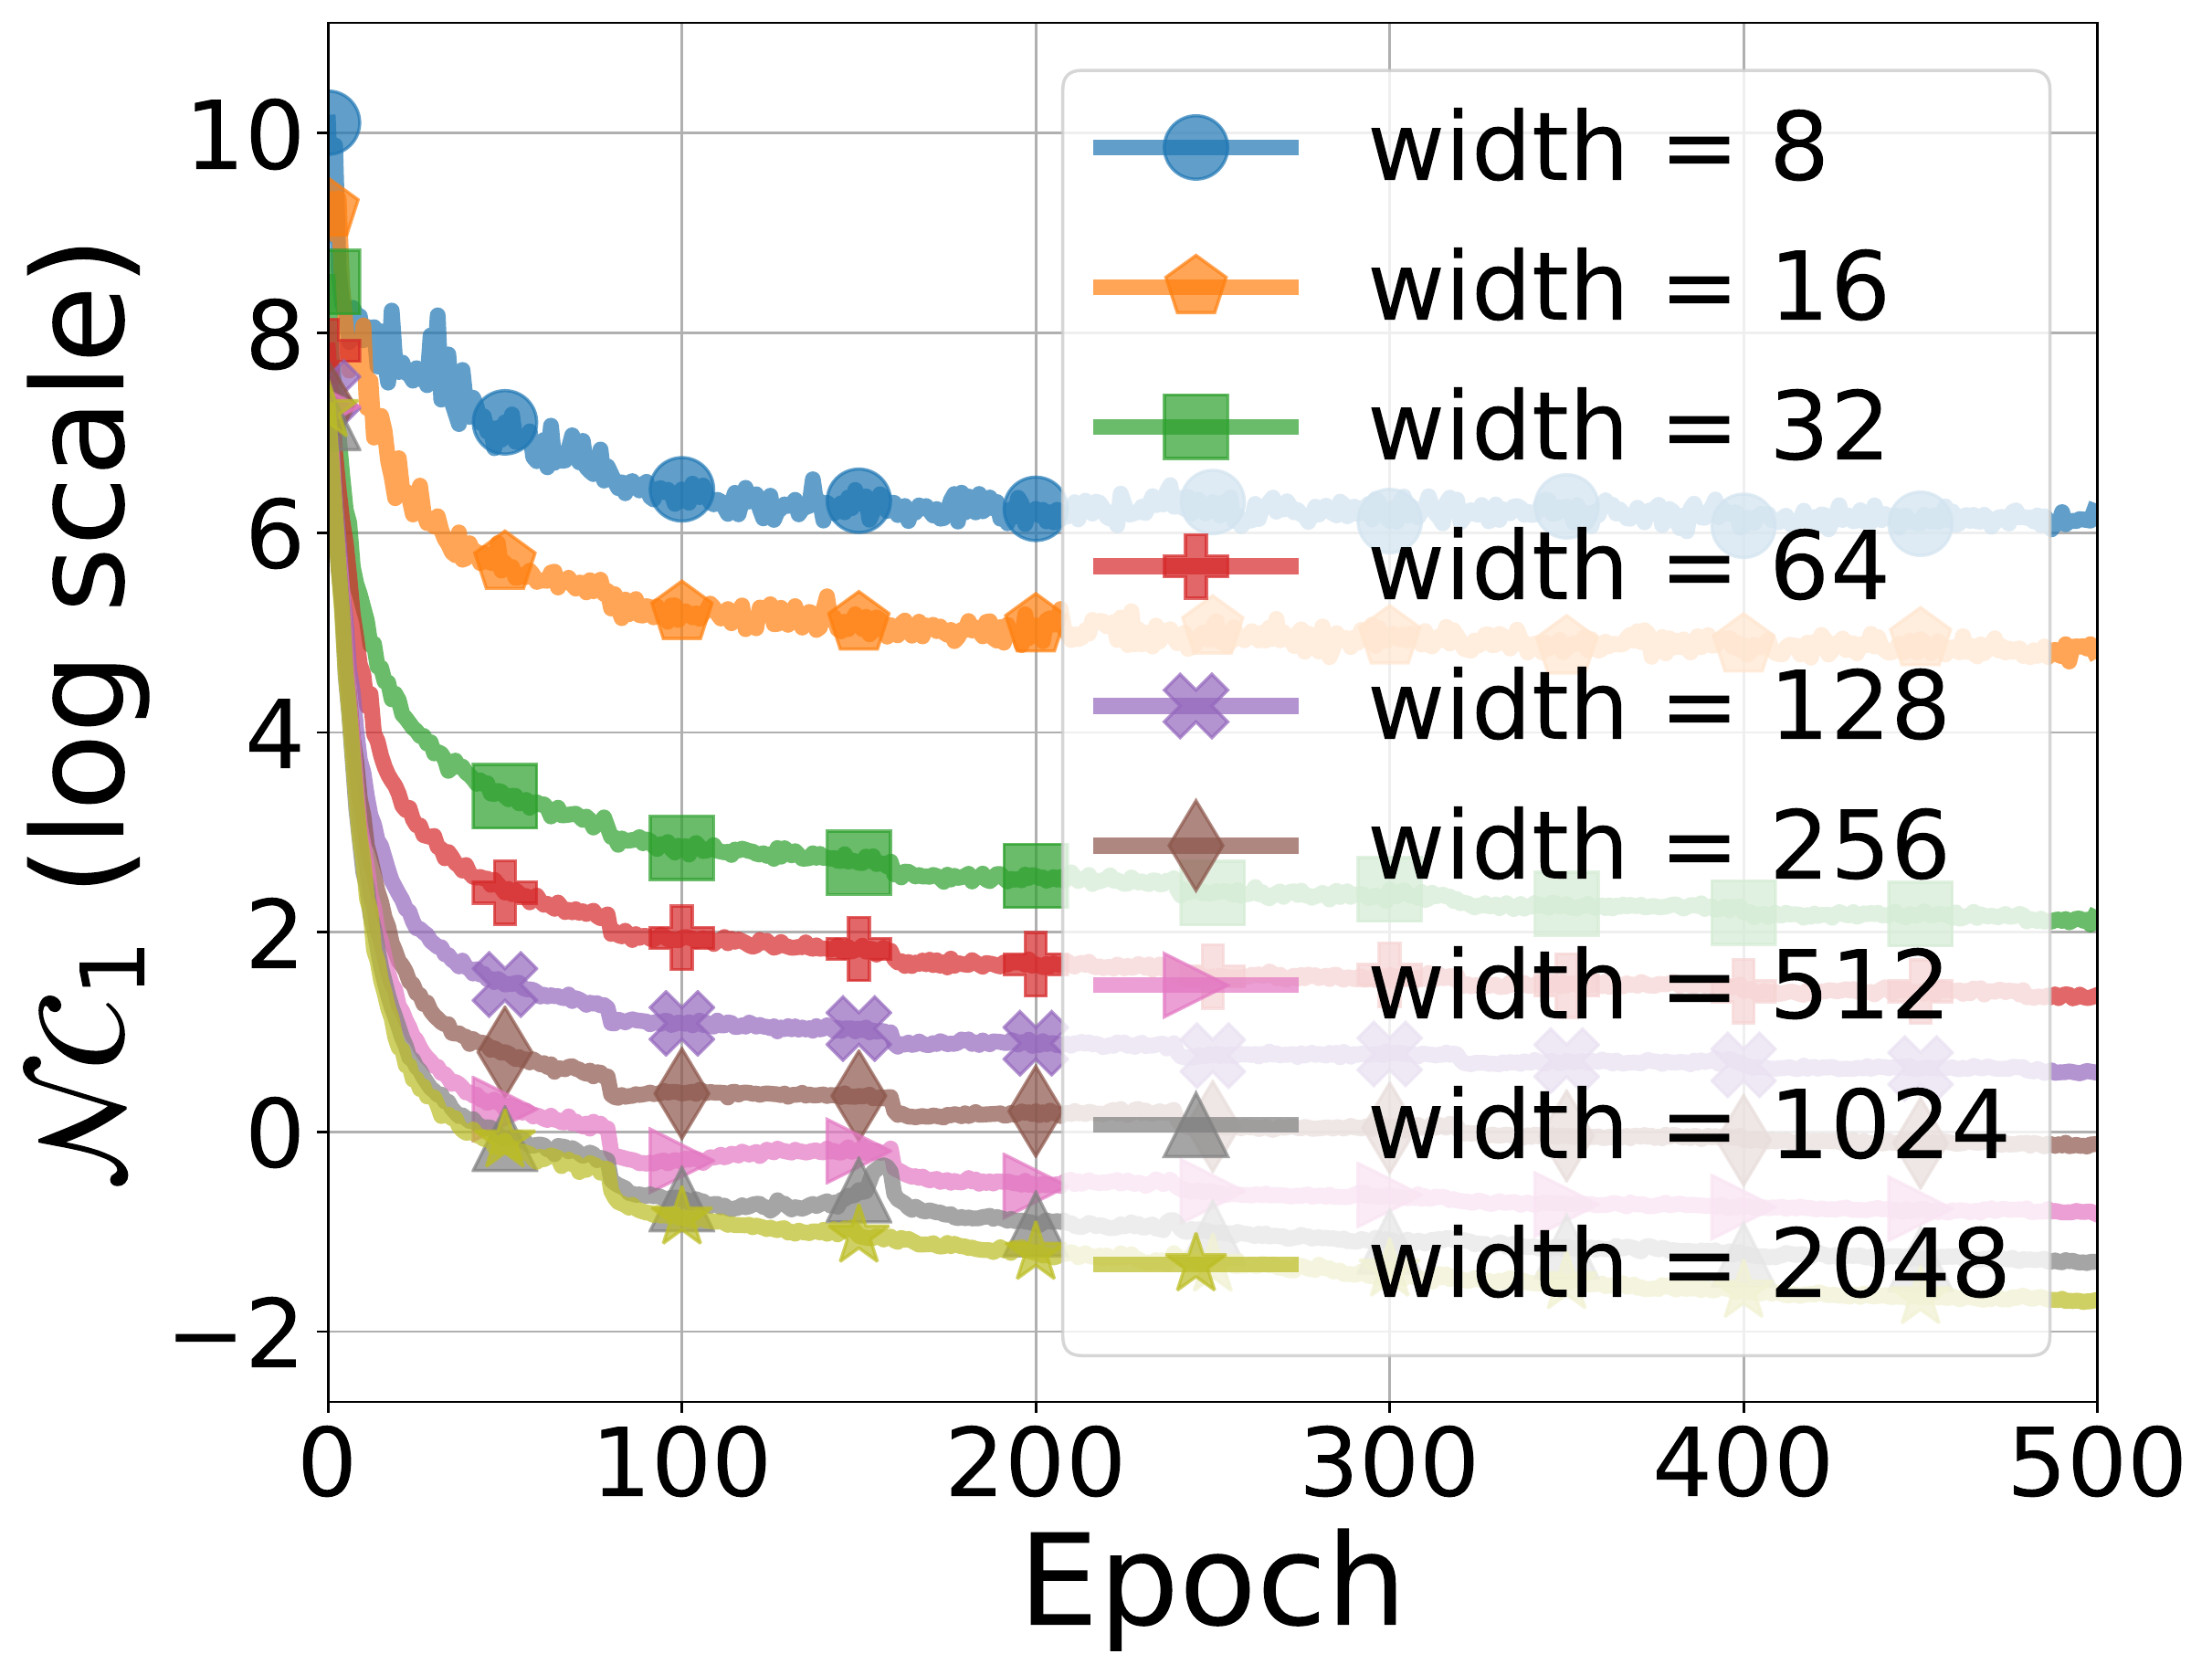} \
        \includegraphics[width=0.24\textwidth]{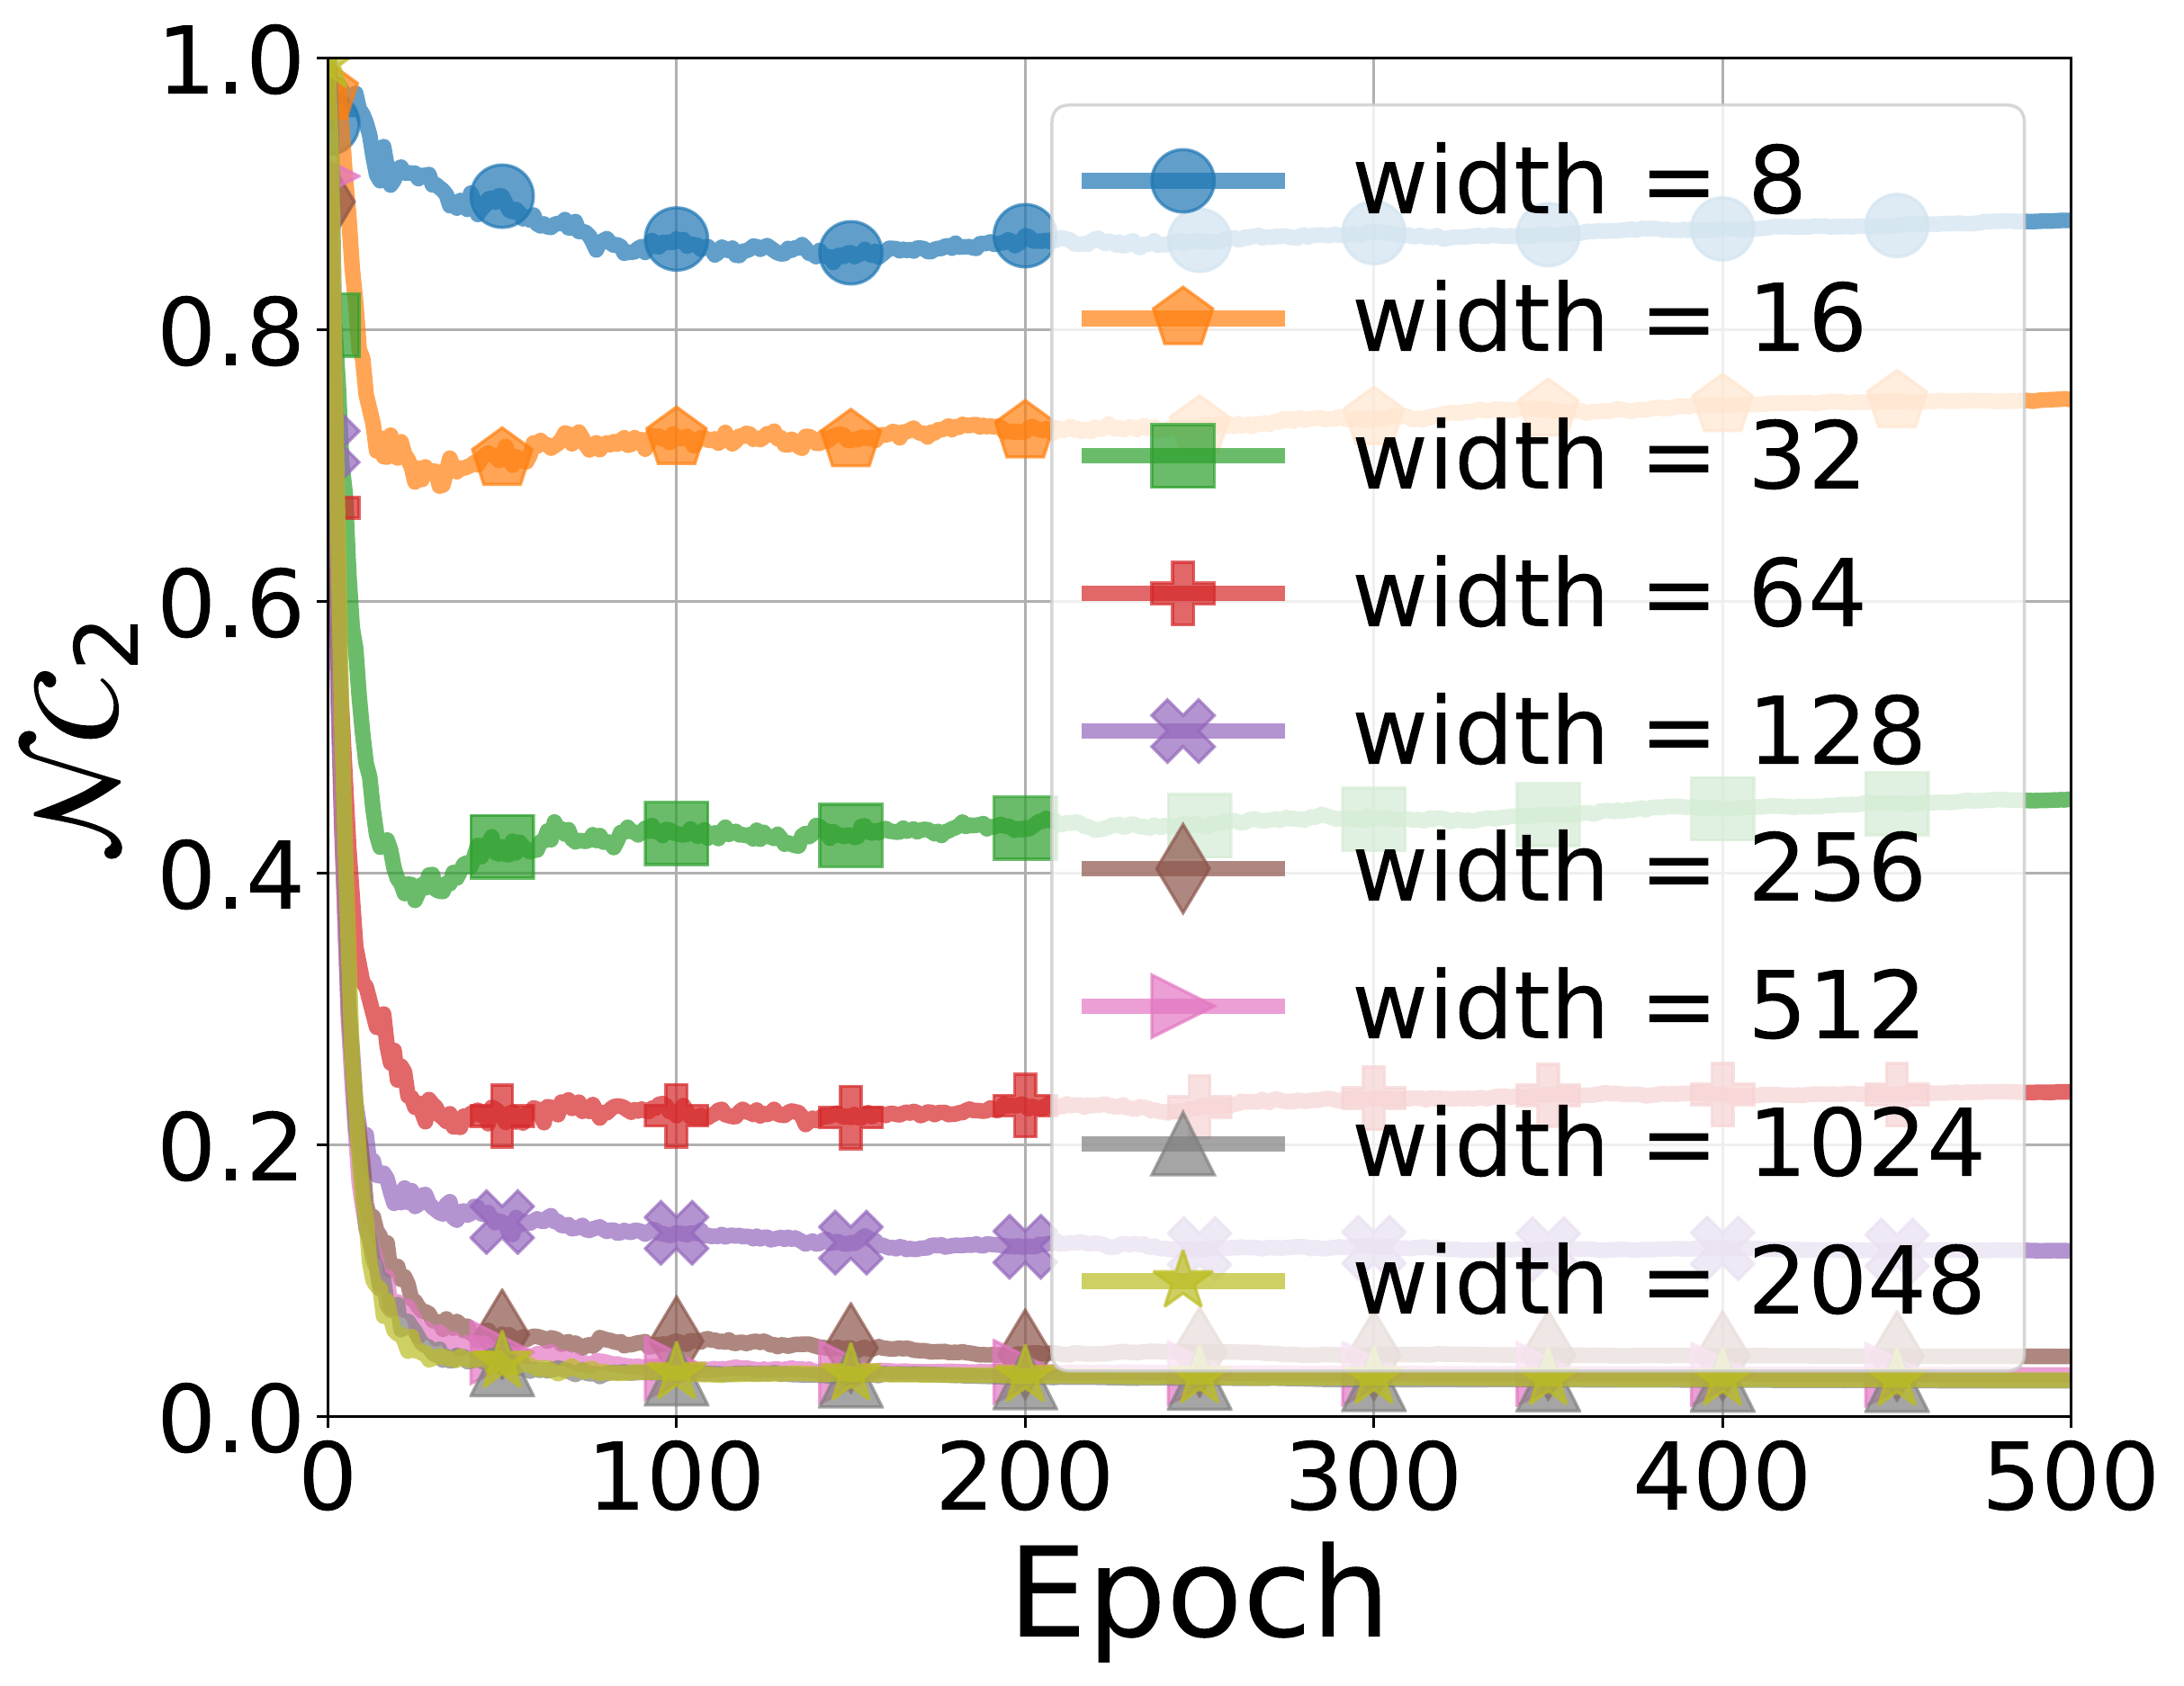} \
        \includegraphics[width=0.24\textwidth]{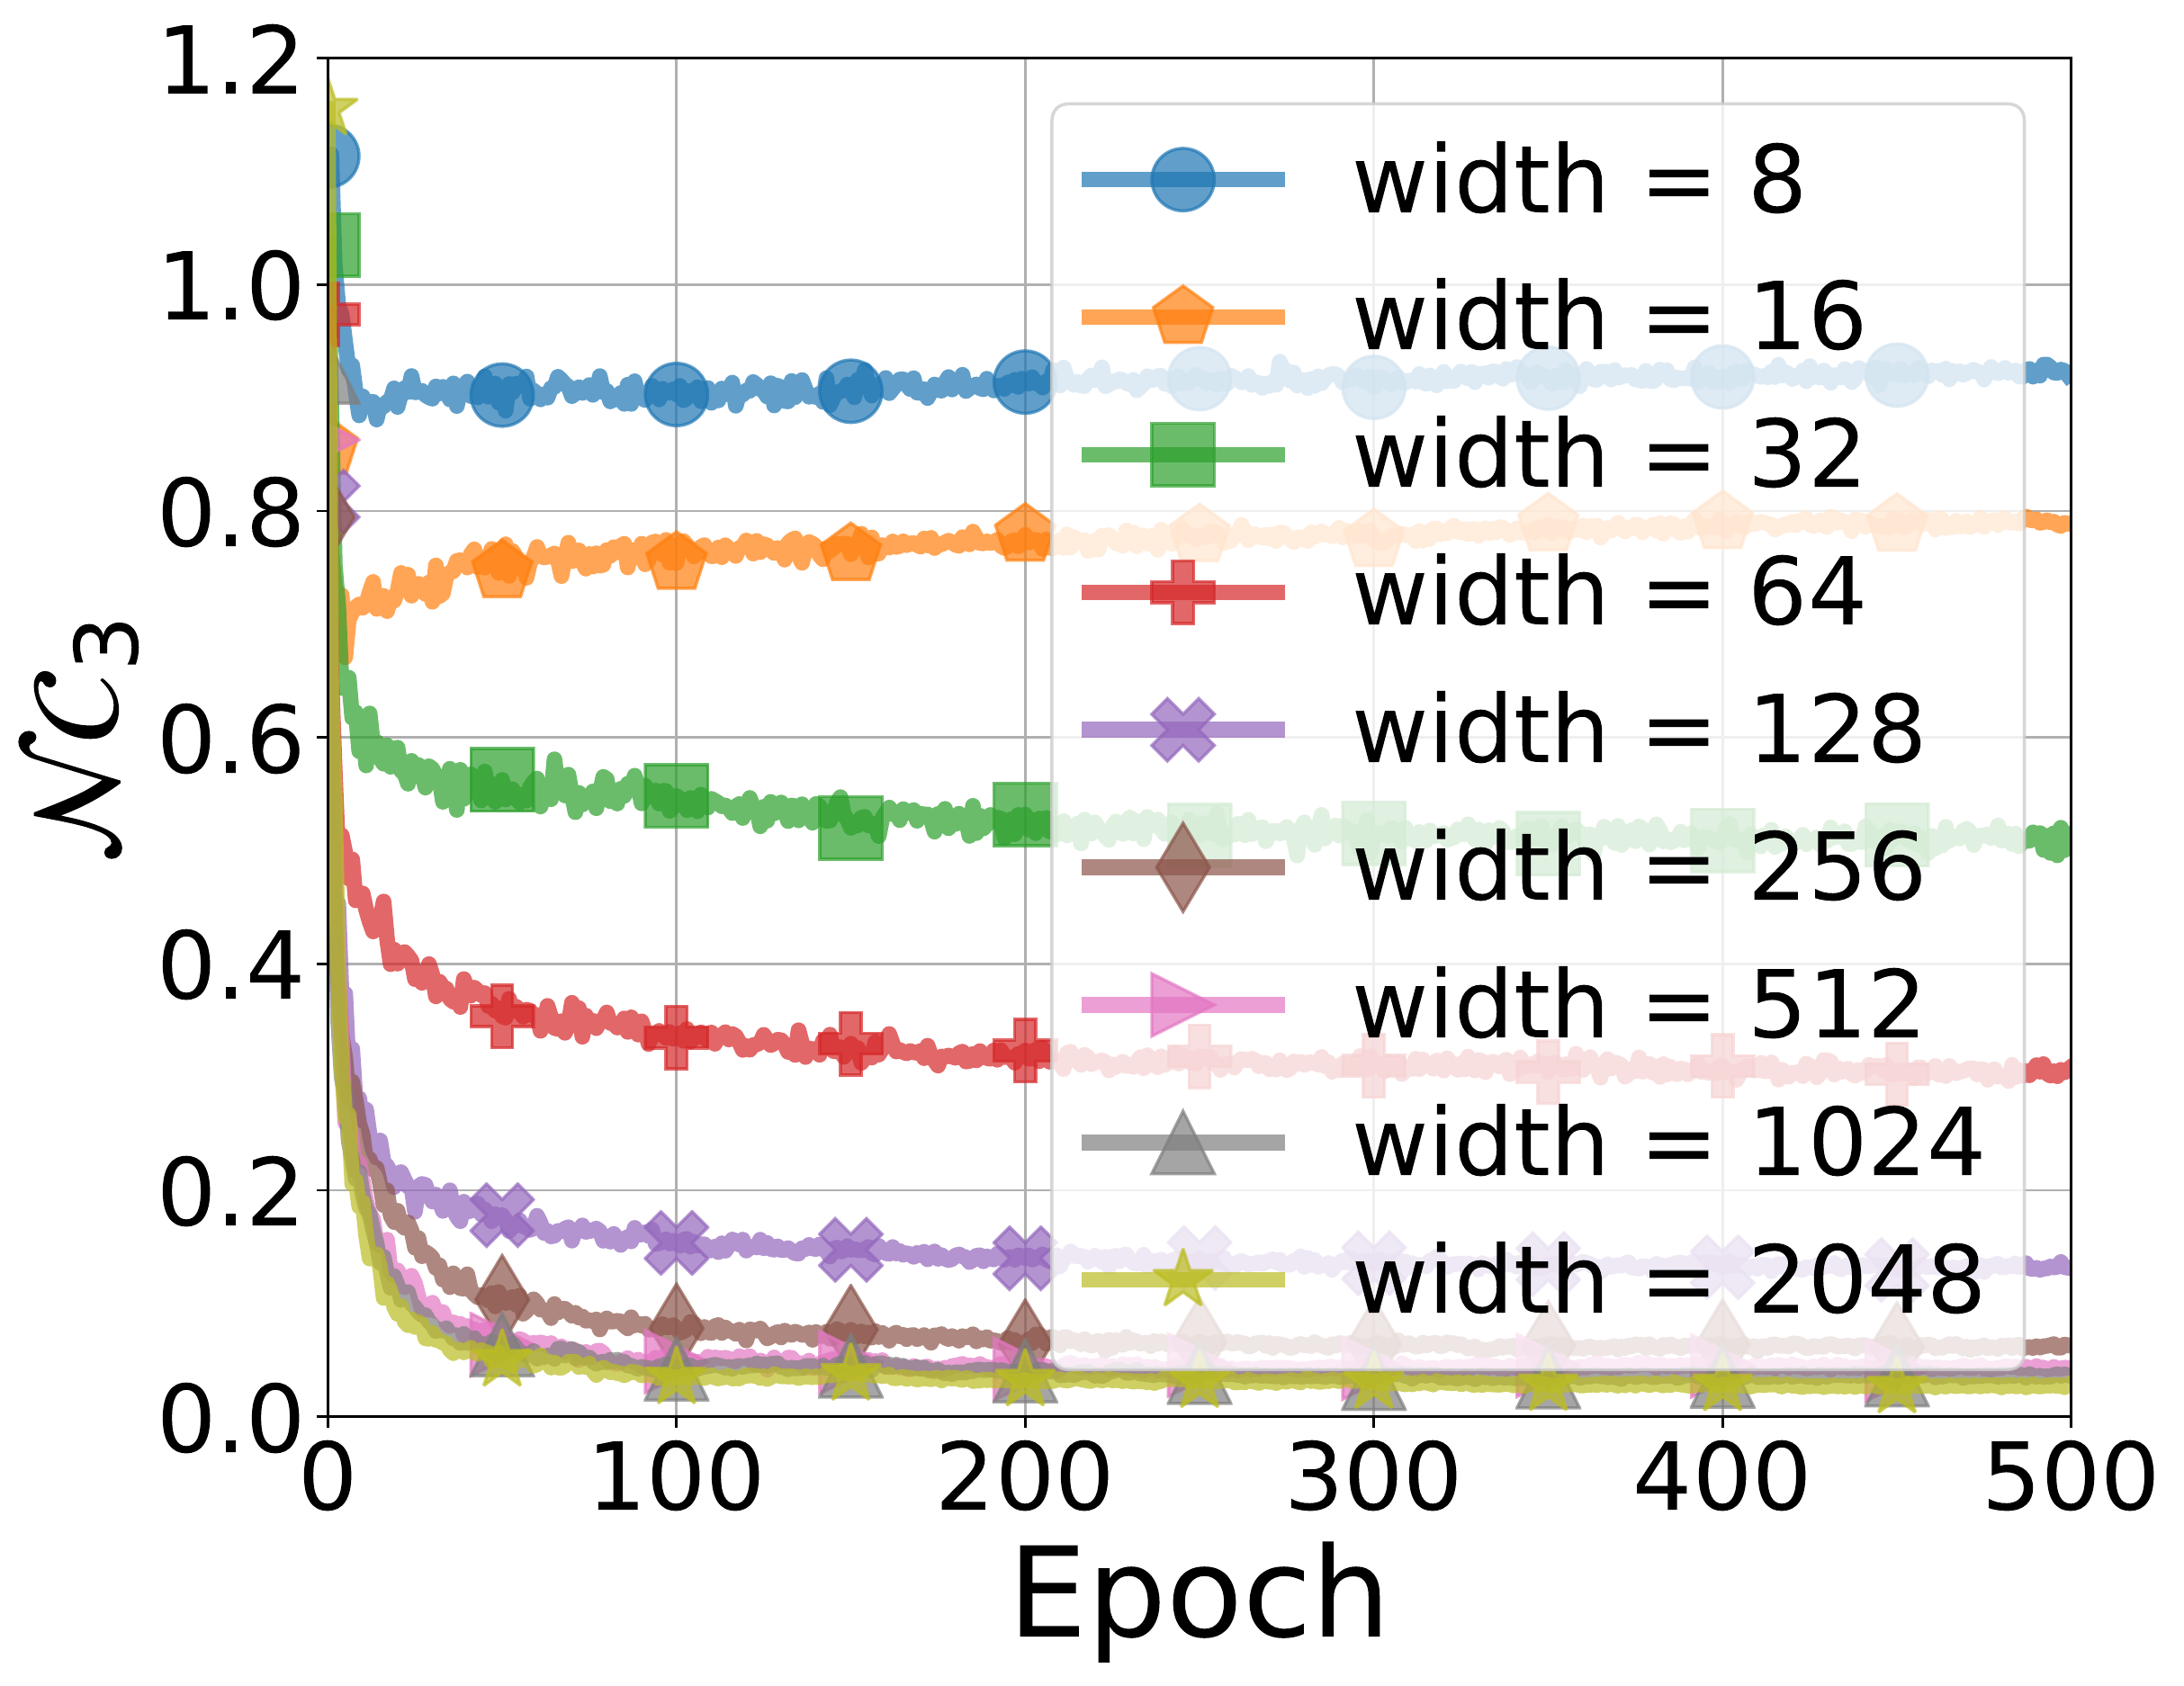} \
        \includegraphics[width=0.24\textwidth]{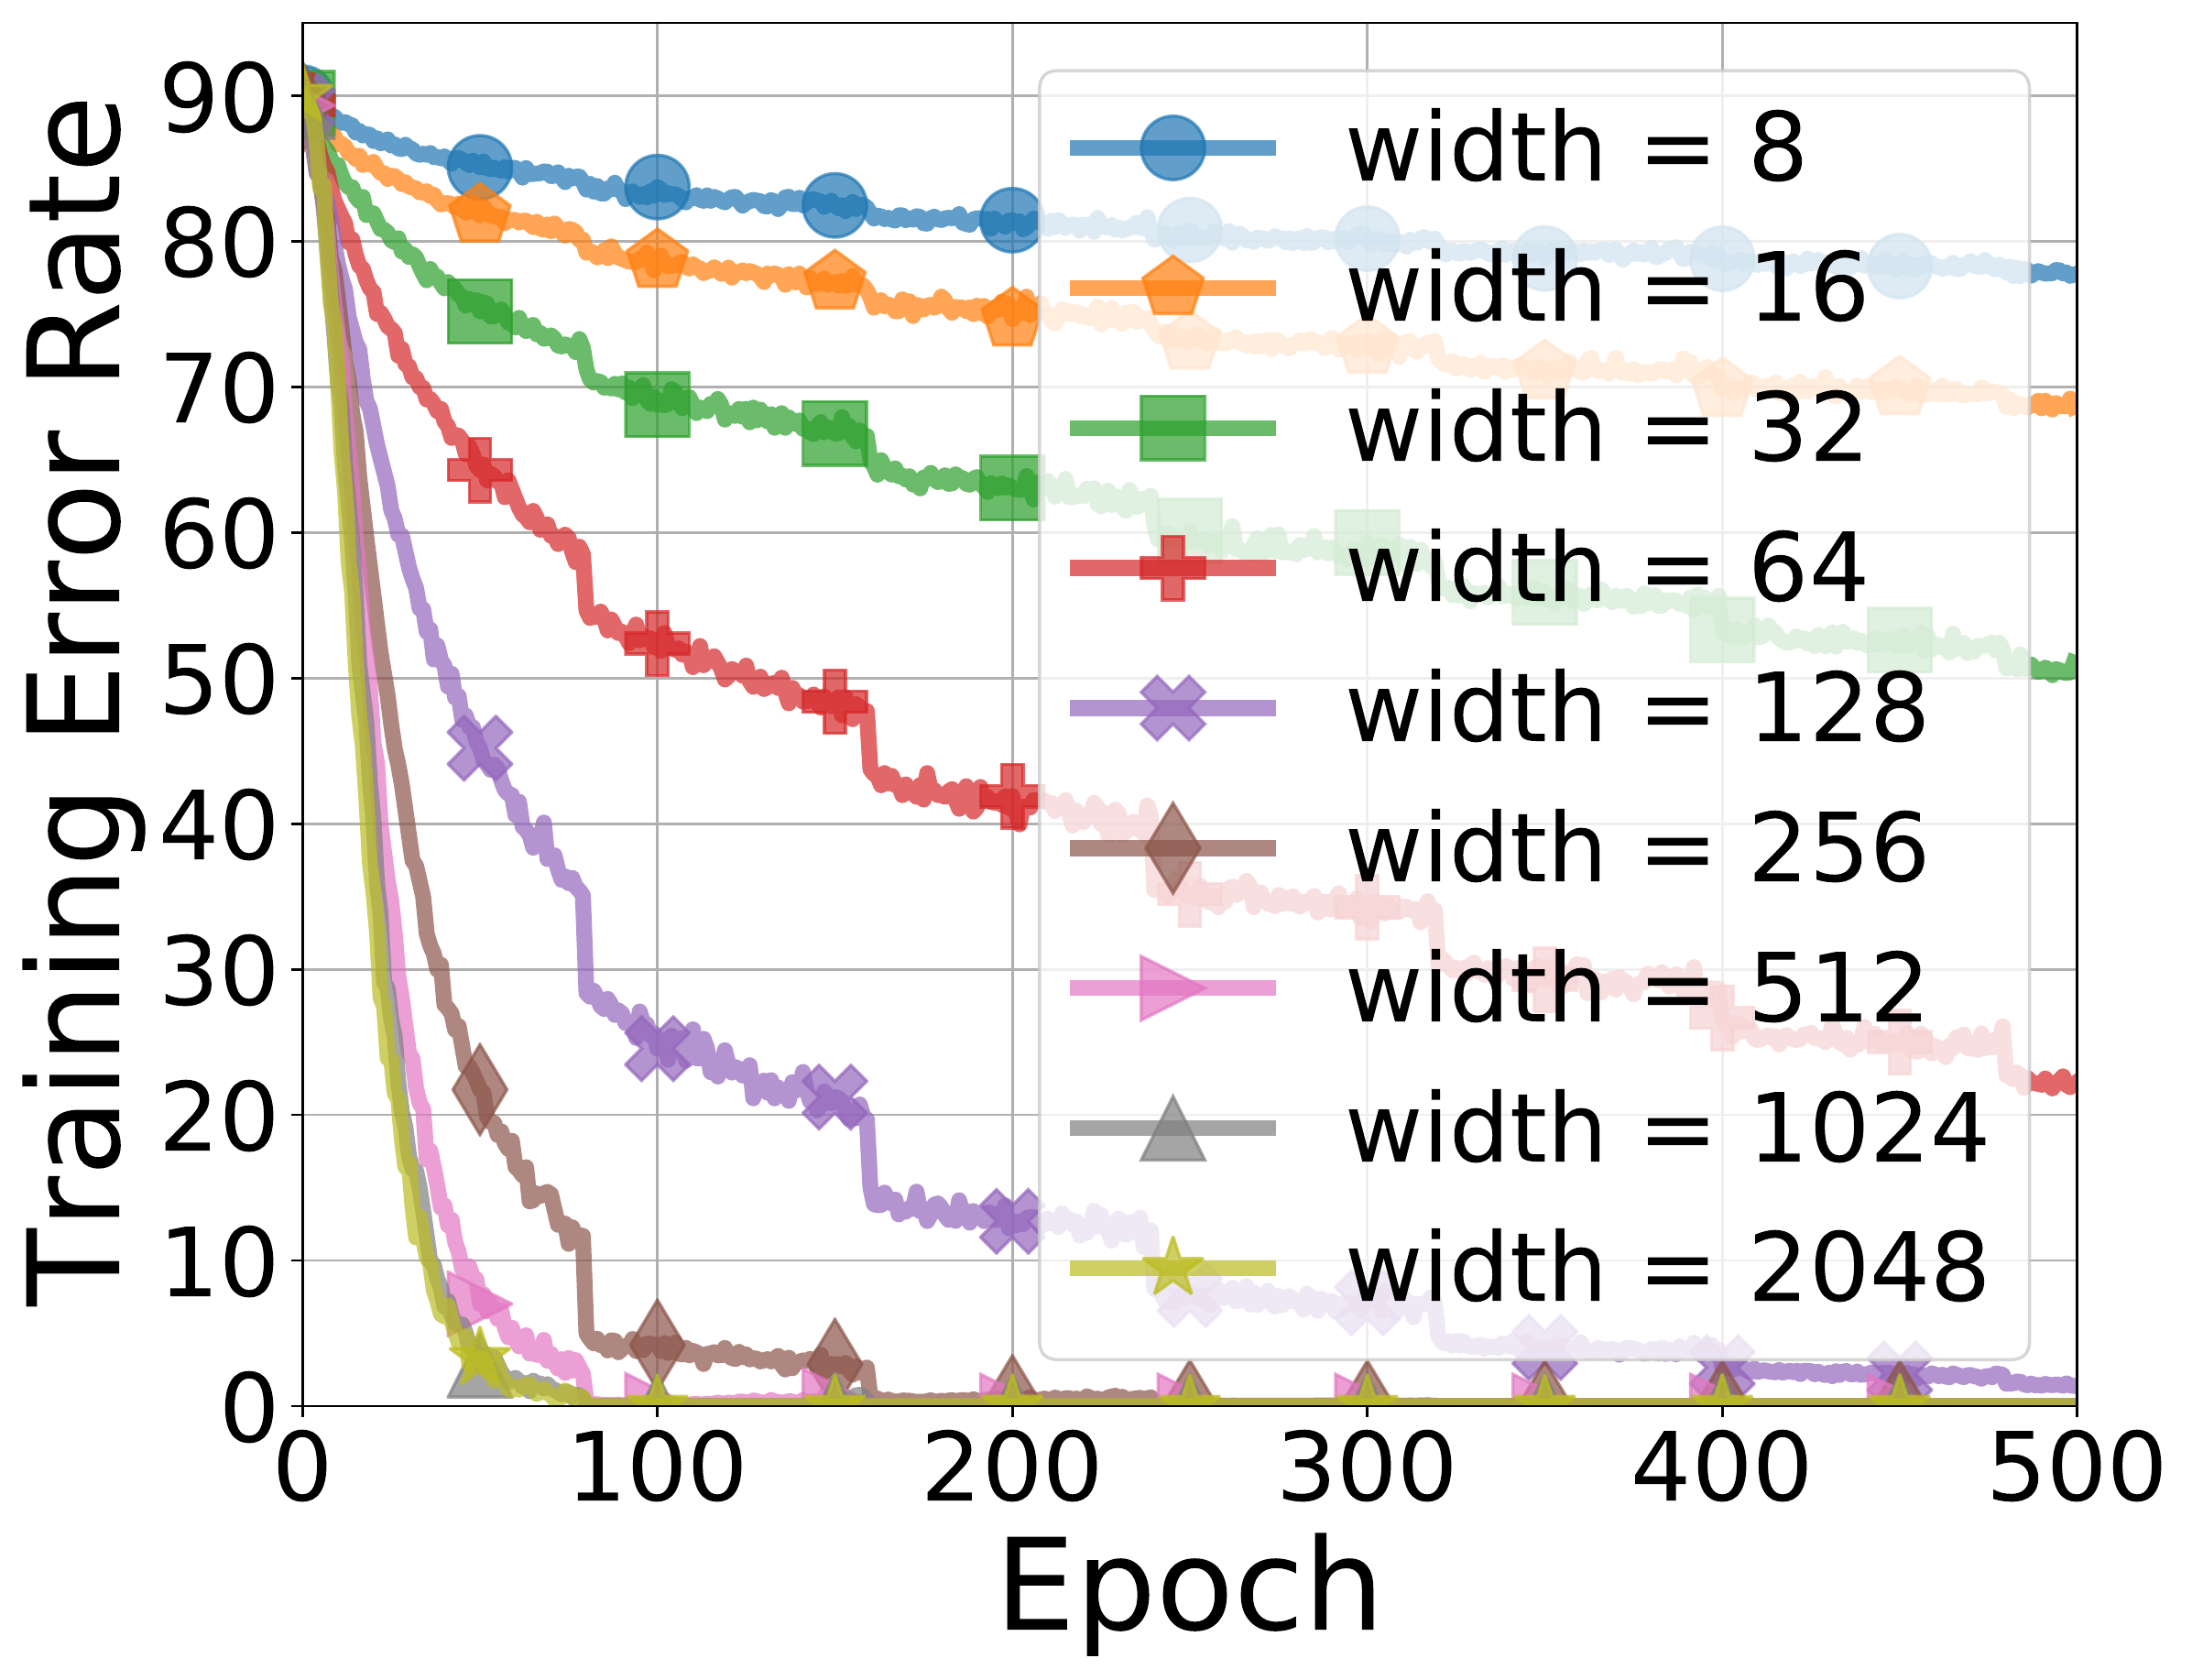}} 
    \caption{\textbf{Training results of CIFAR10 with completely random label.} Multilayer perceptron (MLP) of a fixed depth of $4$ is used with various feature width. Note that the right column is the misclassification percentage of all samples in training. %\zz{Change the Labels for the first two figures. Also the fond for the Yticks can be bigger. Maybe we can plot training error and then we can easily observe similar curves among these three figures.}
    }
    \label{fig:random_label_MLP-appendix}
\end{figure}

\paragraph{Comparison of Weight Decay on the Network Parameter $\mb \Theta$ vs. on the Features $\mb H$ in \eqref{eq:obj}.} 
In comparison to typical training protocols of deep networks which enforce weight decay on all the network weights $\mb \Theta$, our problem formulation \eqref{eq:obj} based on the unconstrained feature model replaced $\mb \Theta$ by penalizing the feature $\mb H$ produced by the $L-1$ ``peeled-off'' layers. To check the practicality of such formulation, we empirically run experiments using ResNet18 on MNIST and CIFAR10. \Cref{fig:NC-WD} shows the \NC\ evolution for both the classical formulation and our ``peeled'' formulation, we notice that the \NC\ behavior happens in both scenarios comparably. We also point that without extensive hyper-parameter tuning, the models trained under the ``peeled'' set-up could already achieve test accuracy of $99.57\%$ and $77.92\%$ on MNIST and CIFAR10 respectively. We note that such performances are on-par with the test accuracy of the 
classical formulation \eqref{eqn:dl-ce-loss}, with test accuracy of $99.60\%$ and $78.42\%$ on MNIST and CIFAR10 as reported in \Cref{fig:Accuracy-MNIST-CIFAR10}.
%In \textbf{xx}, we demonstrate that such a difference leads to comparable performance in practice -- the performance of the trained network remains similar, and \NC\ still occurs. 

%While the practice of deep learning adopts weight decay on the parameters $\mb \theta$ of the $L-1$ ``peeled-off'' layers, the unconstrained feature model proposes to instead penalize the norm of the features $\mb H$ that are produced by the ``peeled-off'' layers. In the following, we demonstrate that such a difference is negligible in practice: even if we replace the weight decay on $\mb \theta$ -- as in a typical training protocol of deep networks-- with weight decay on $\mb H$, t

%\zz{Any results yet? We may add this later.}

\begin{figure}[t]
    \centering
    \subfloat[$\mc {NC}_1$ (MNIST)]{\includegraphics[width=0.24\textwidth]{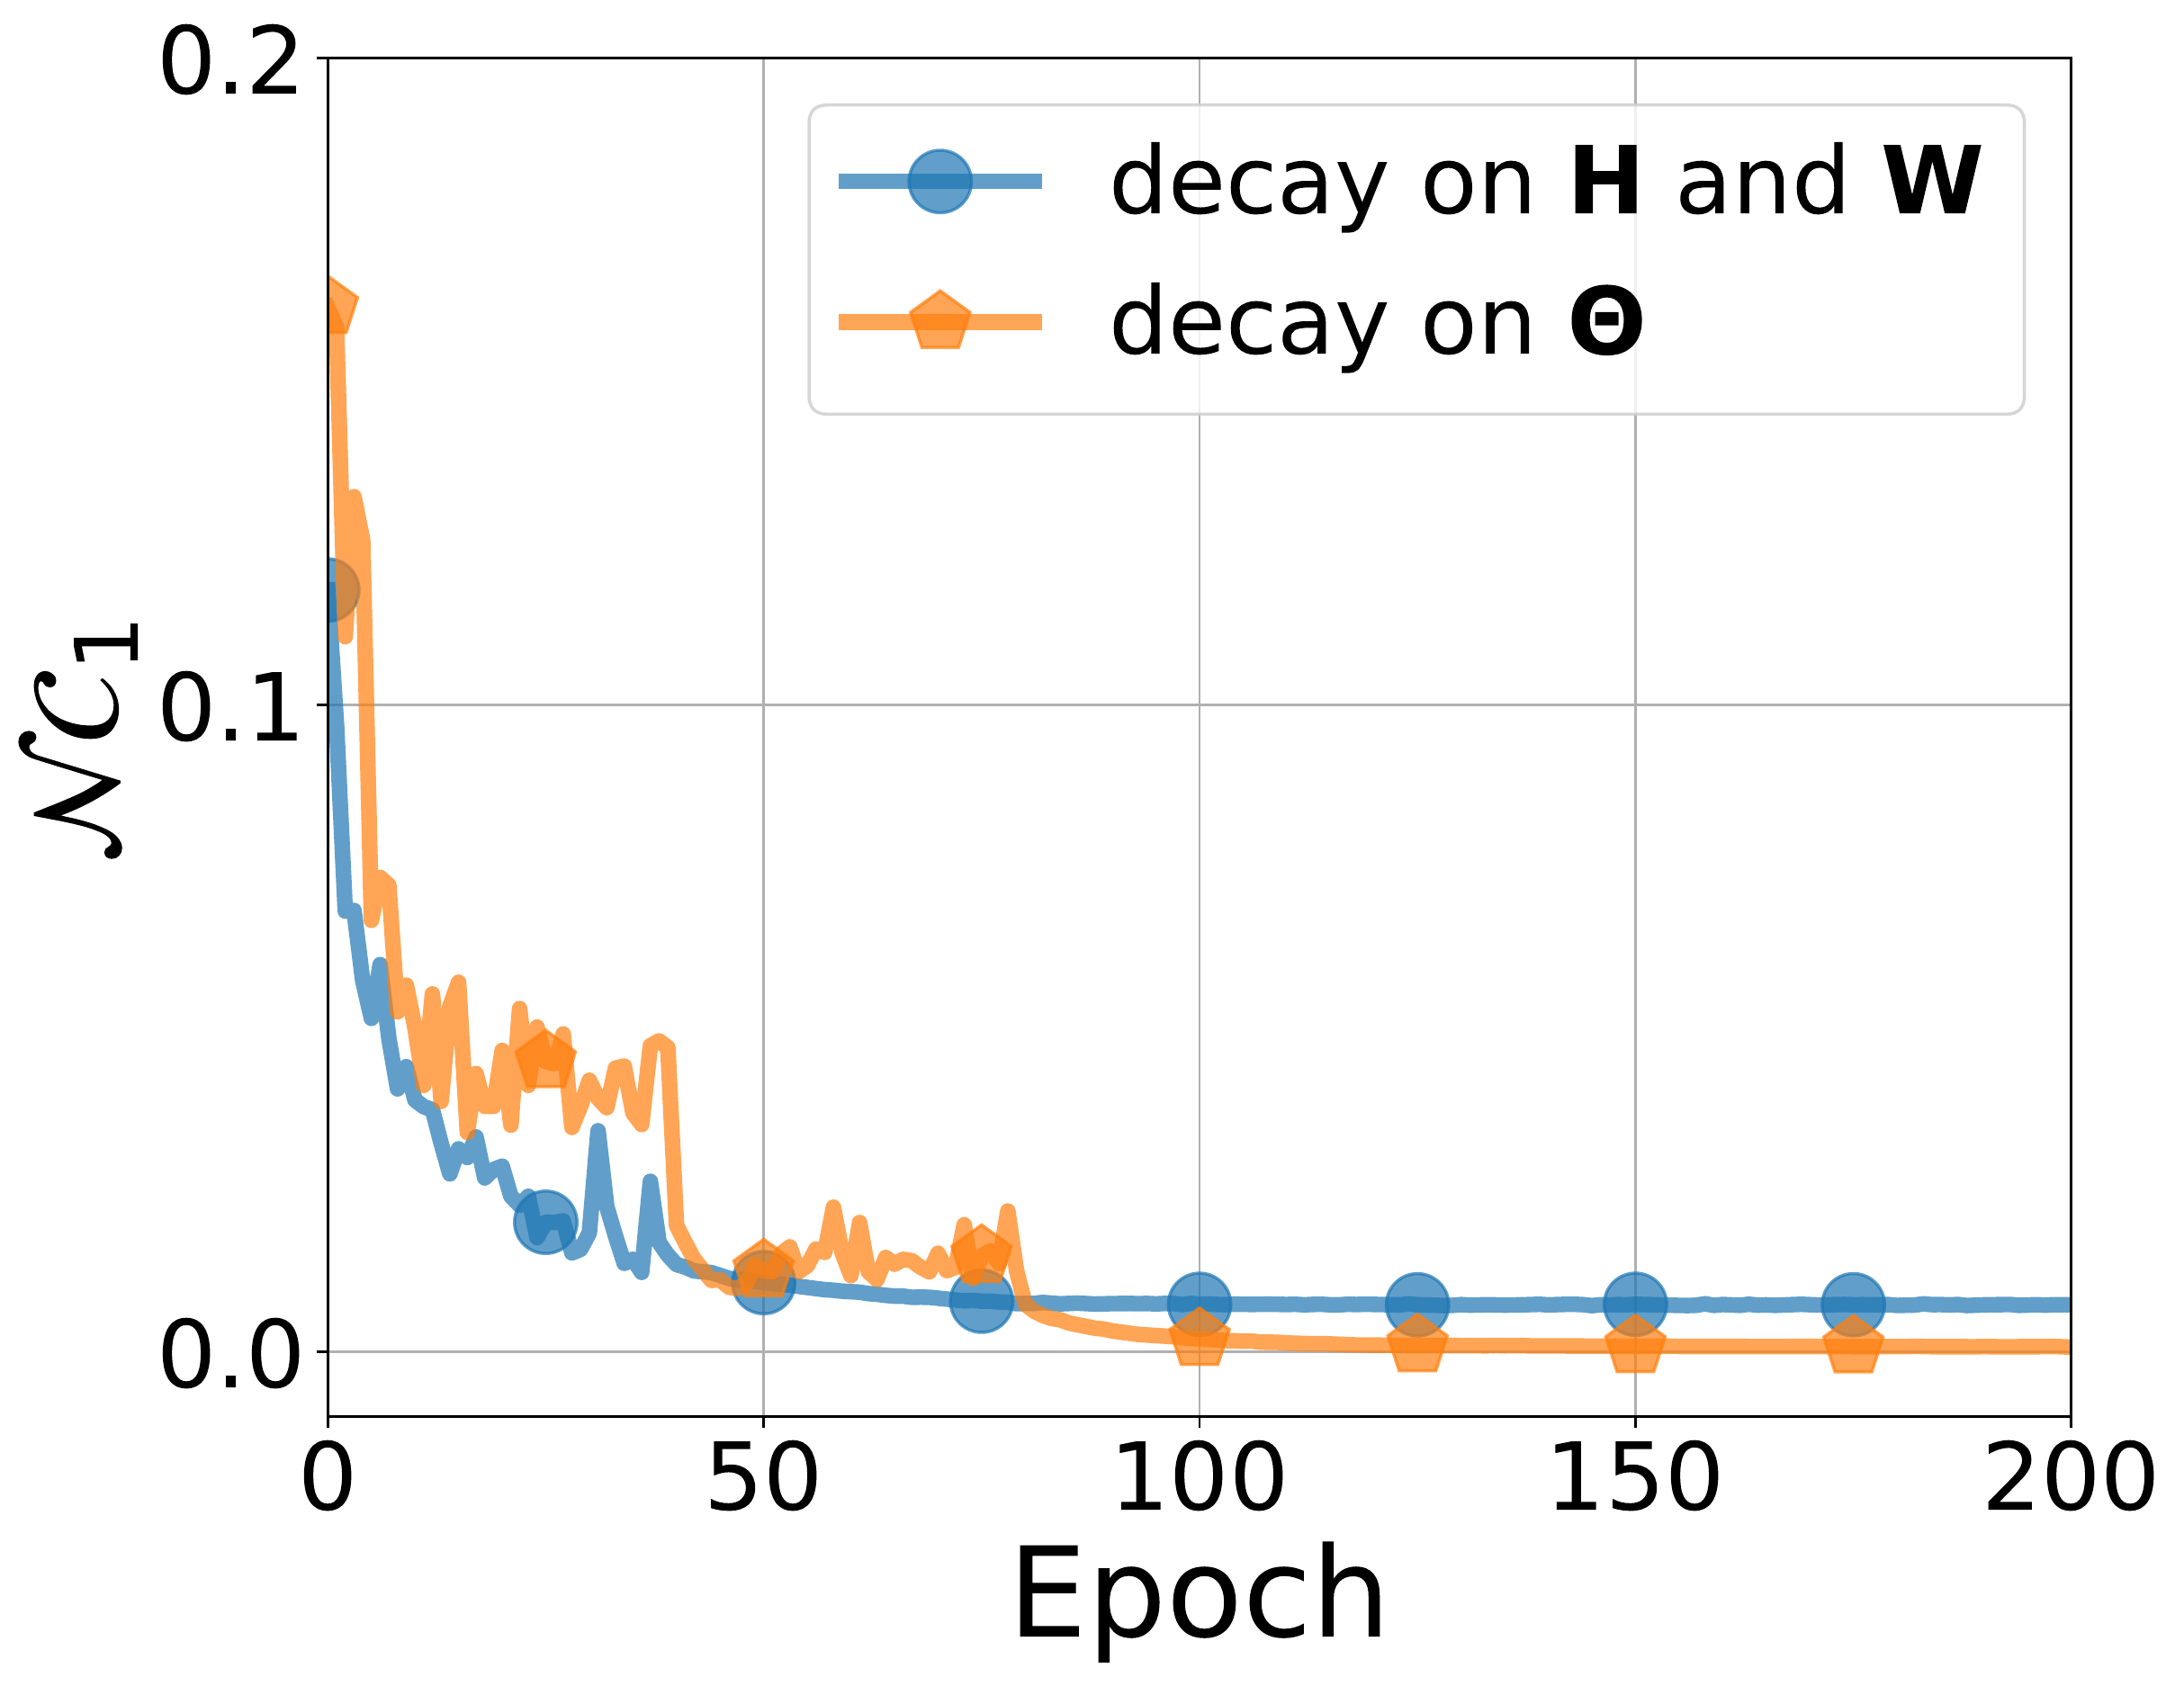}} \
    \subfloat[$\mc {NC}_2$ (MNIST)]{\includegraphics[width=0.24\textwidth]{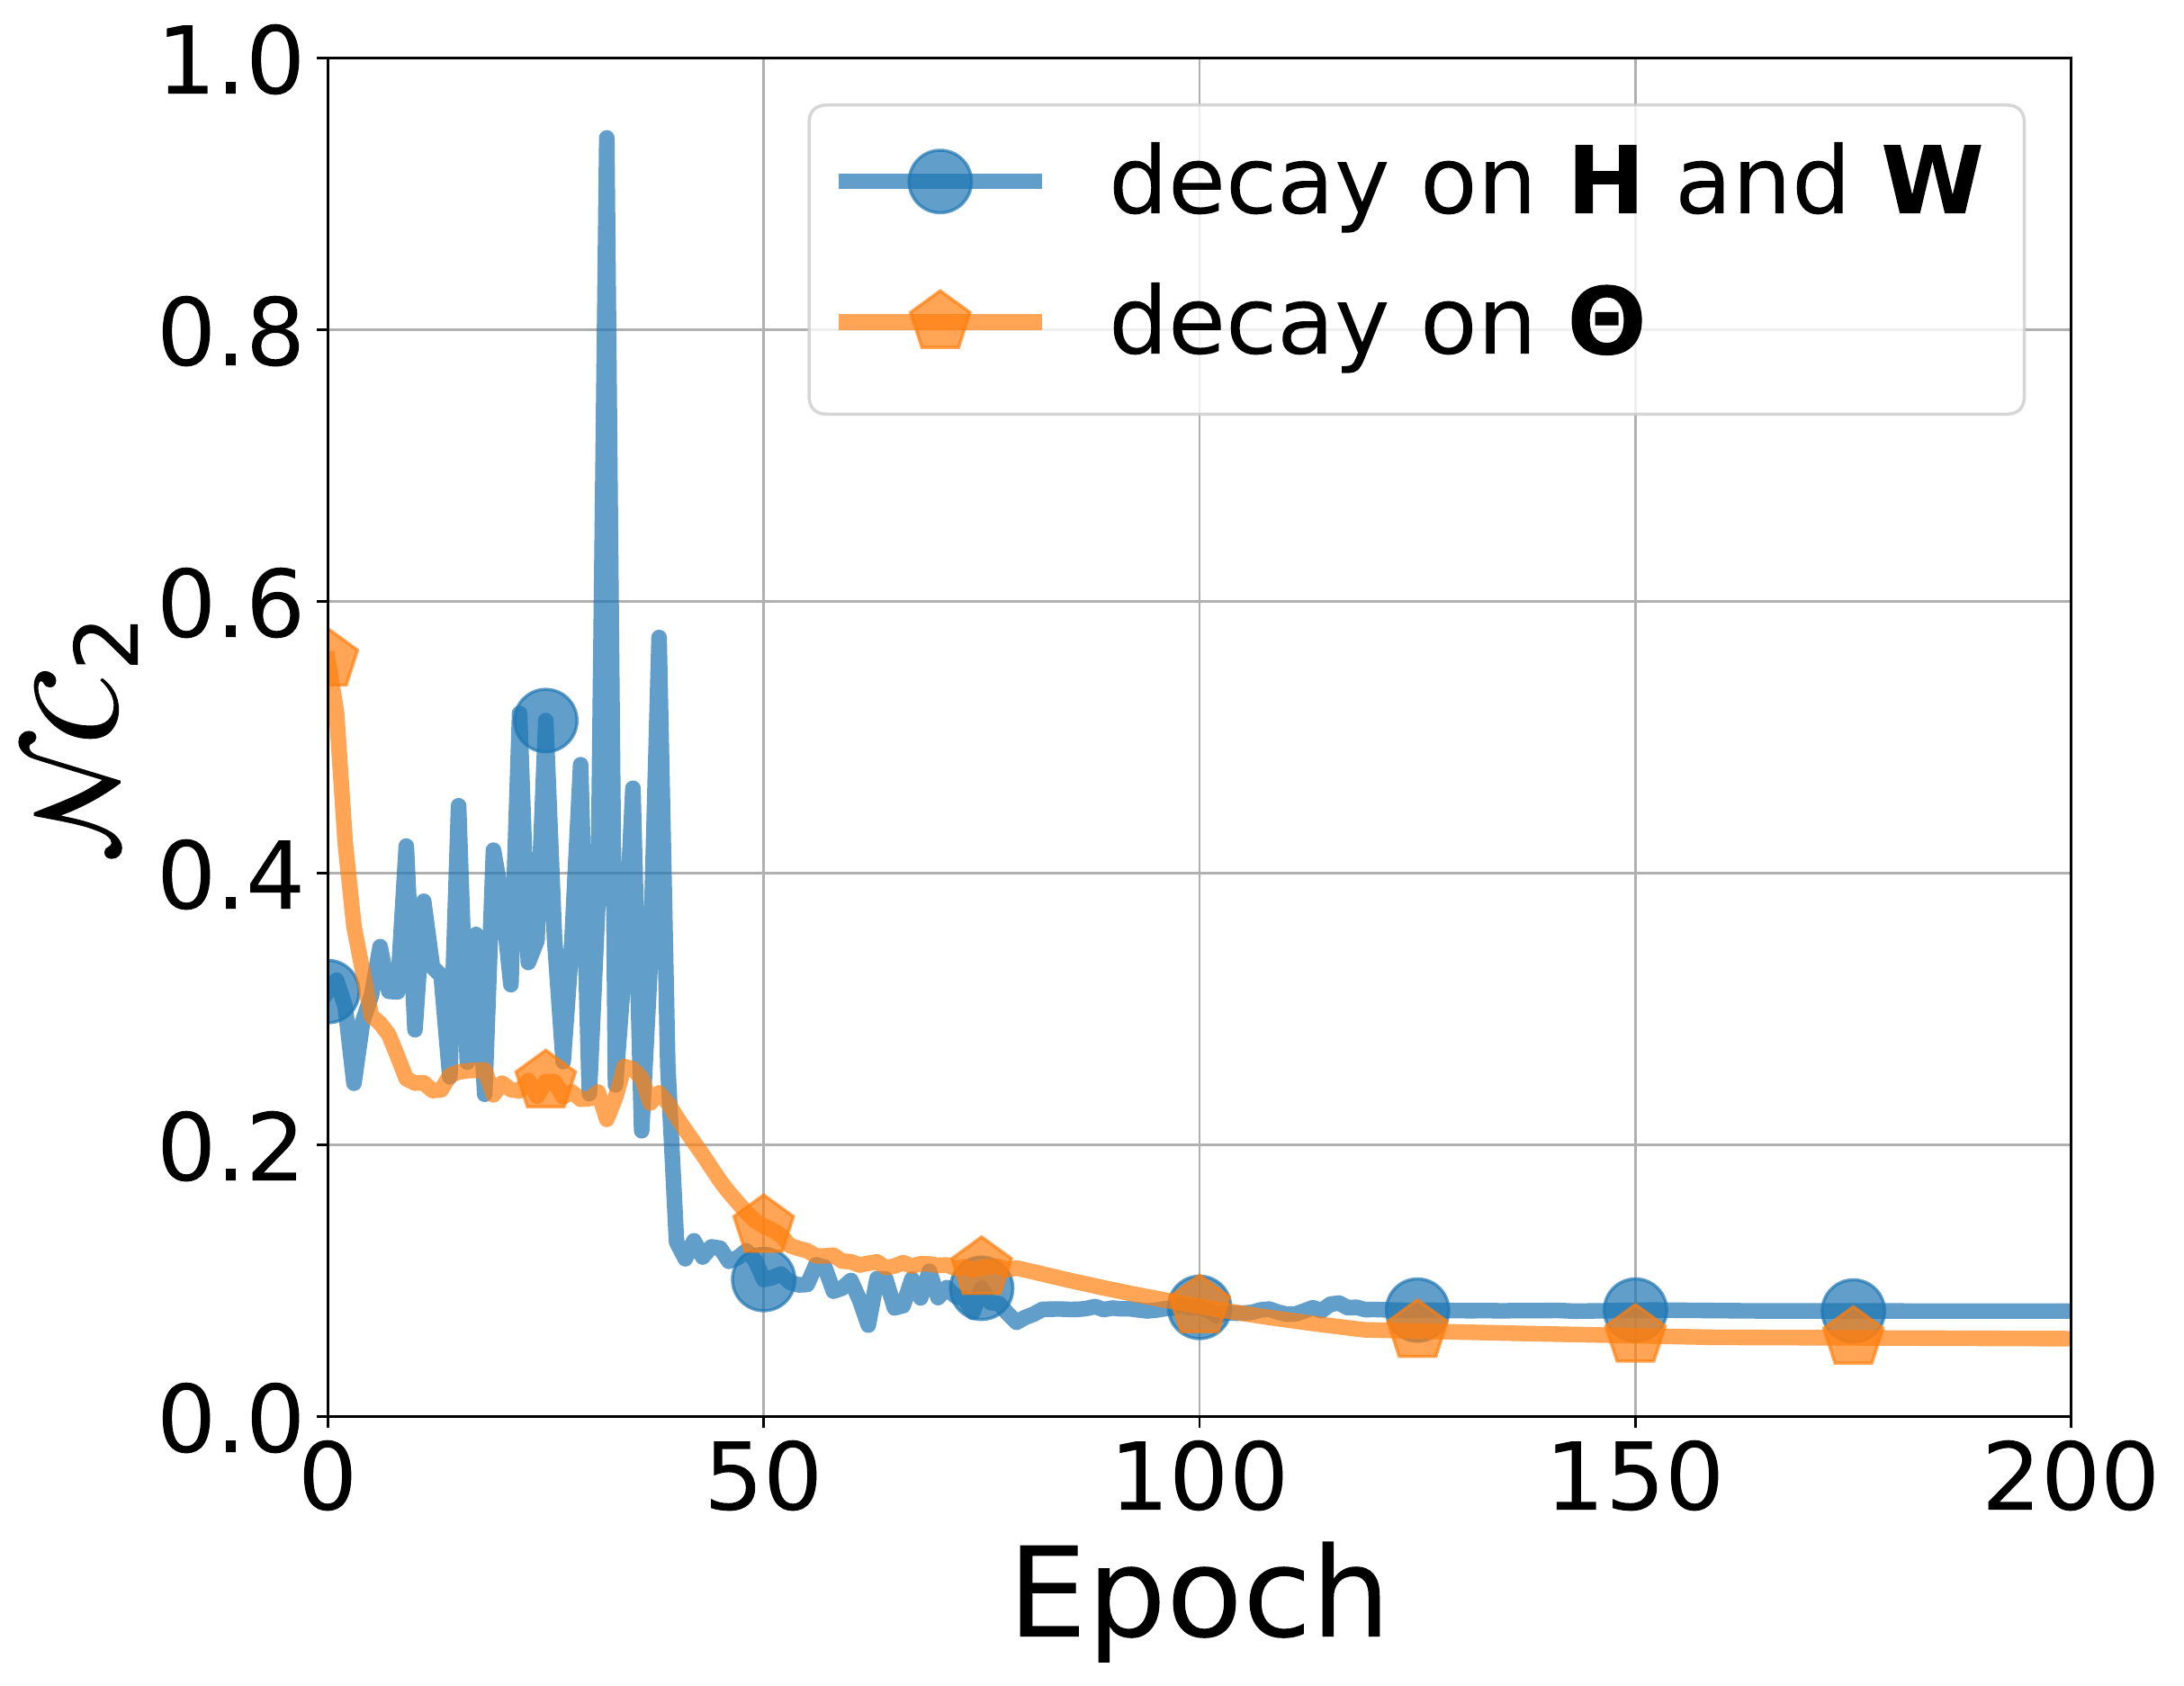}} \
    \subfloat[$\mc {NC}_3$ (MNIST)]{\includegraphics[width=0.24\textwidth]{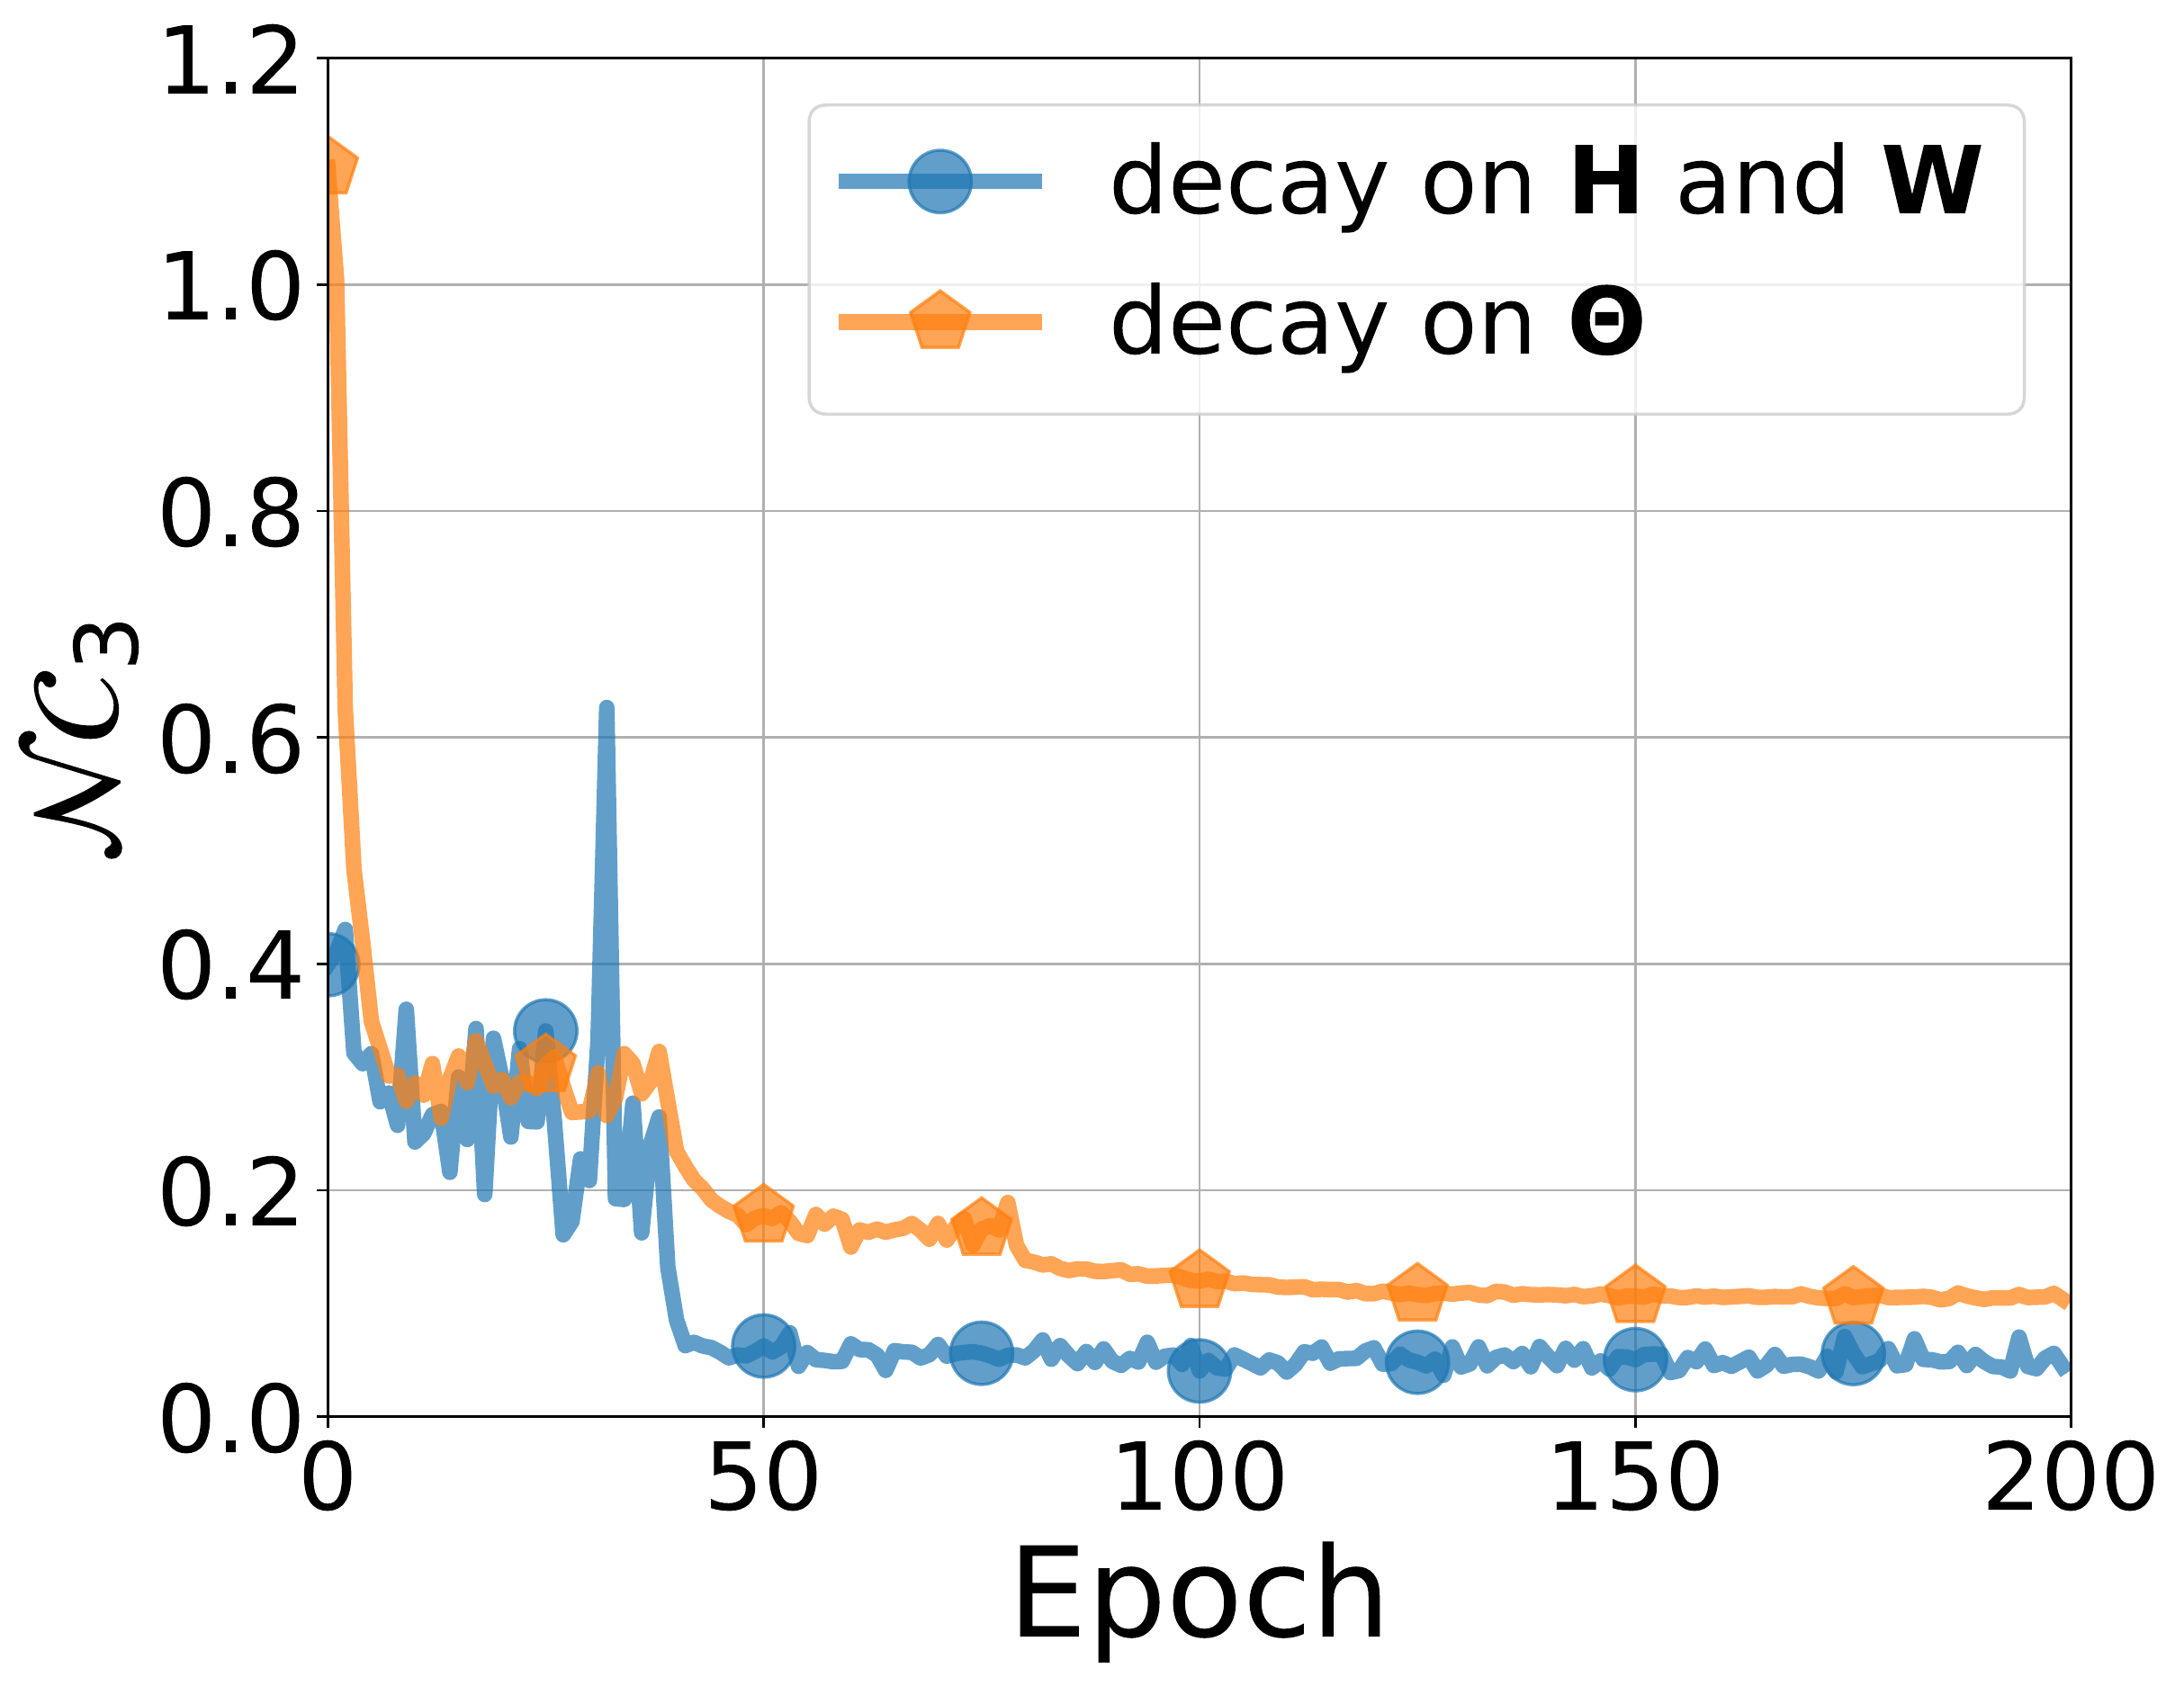}} \
    \subfloat[$\mc {NC}_4$ (MNIST)]{\includegraphics[width=0.23\textwidth]{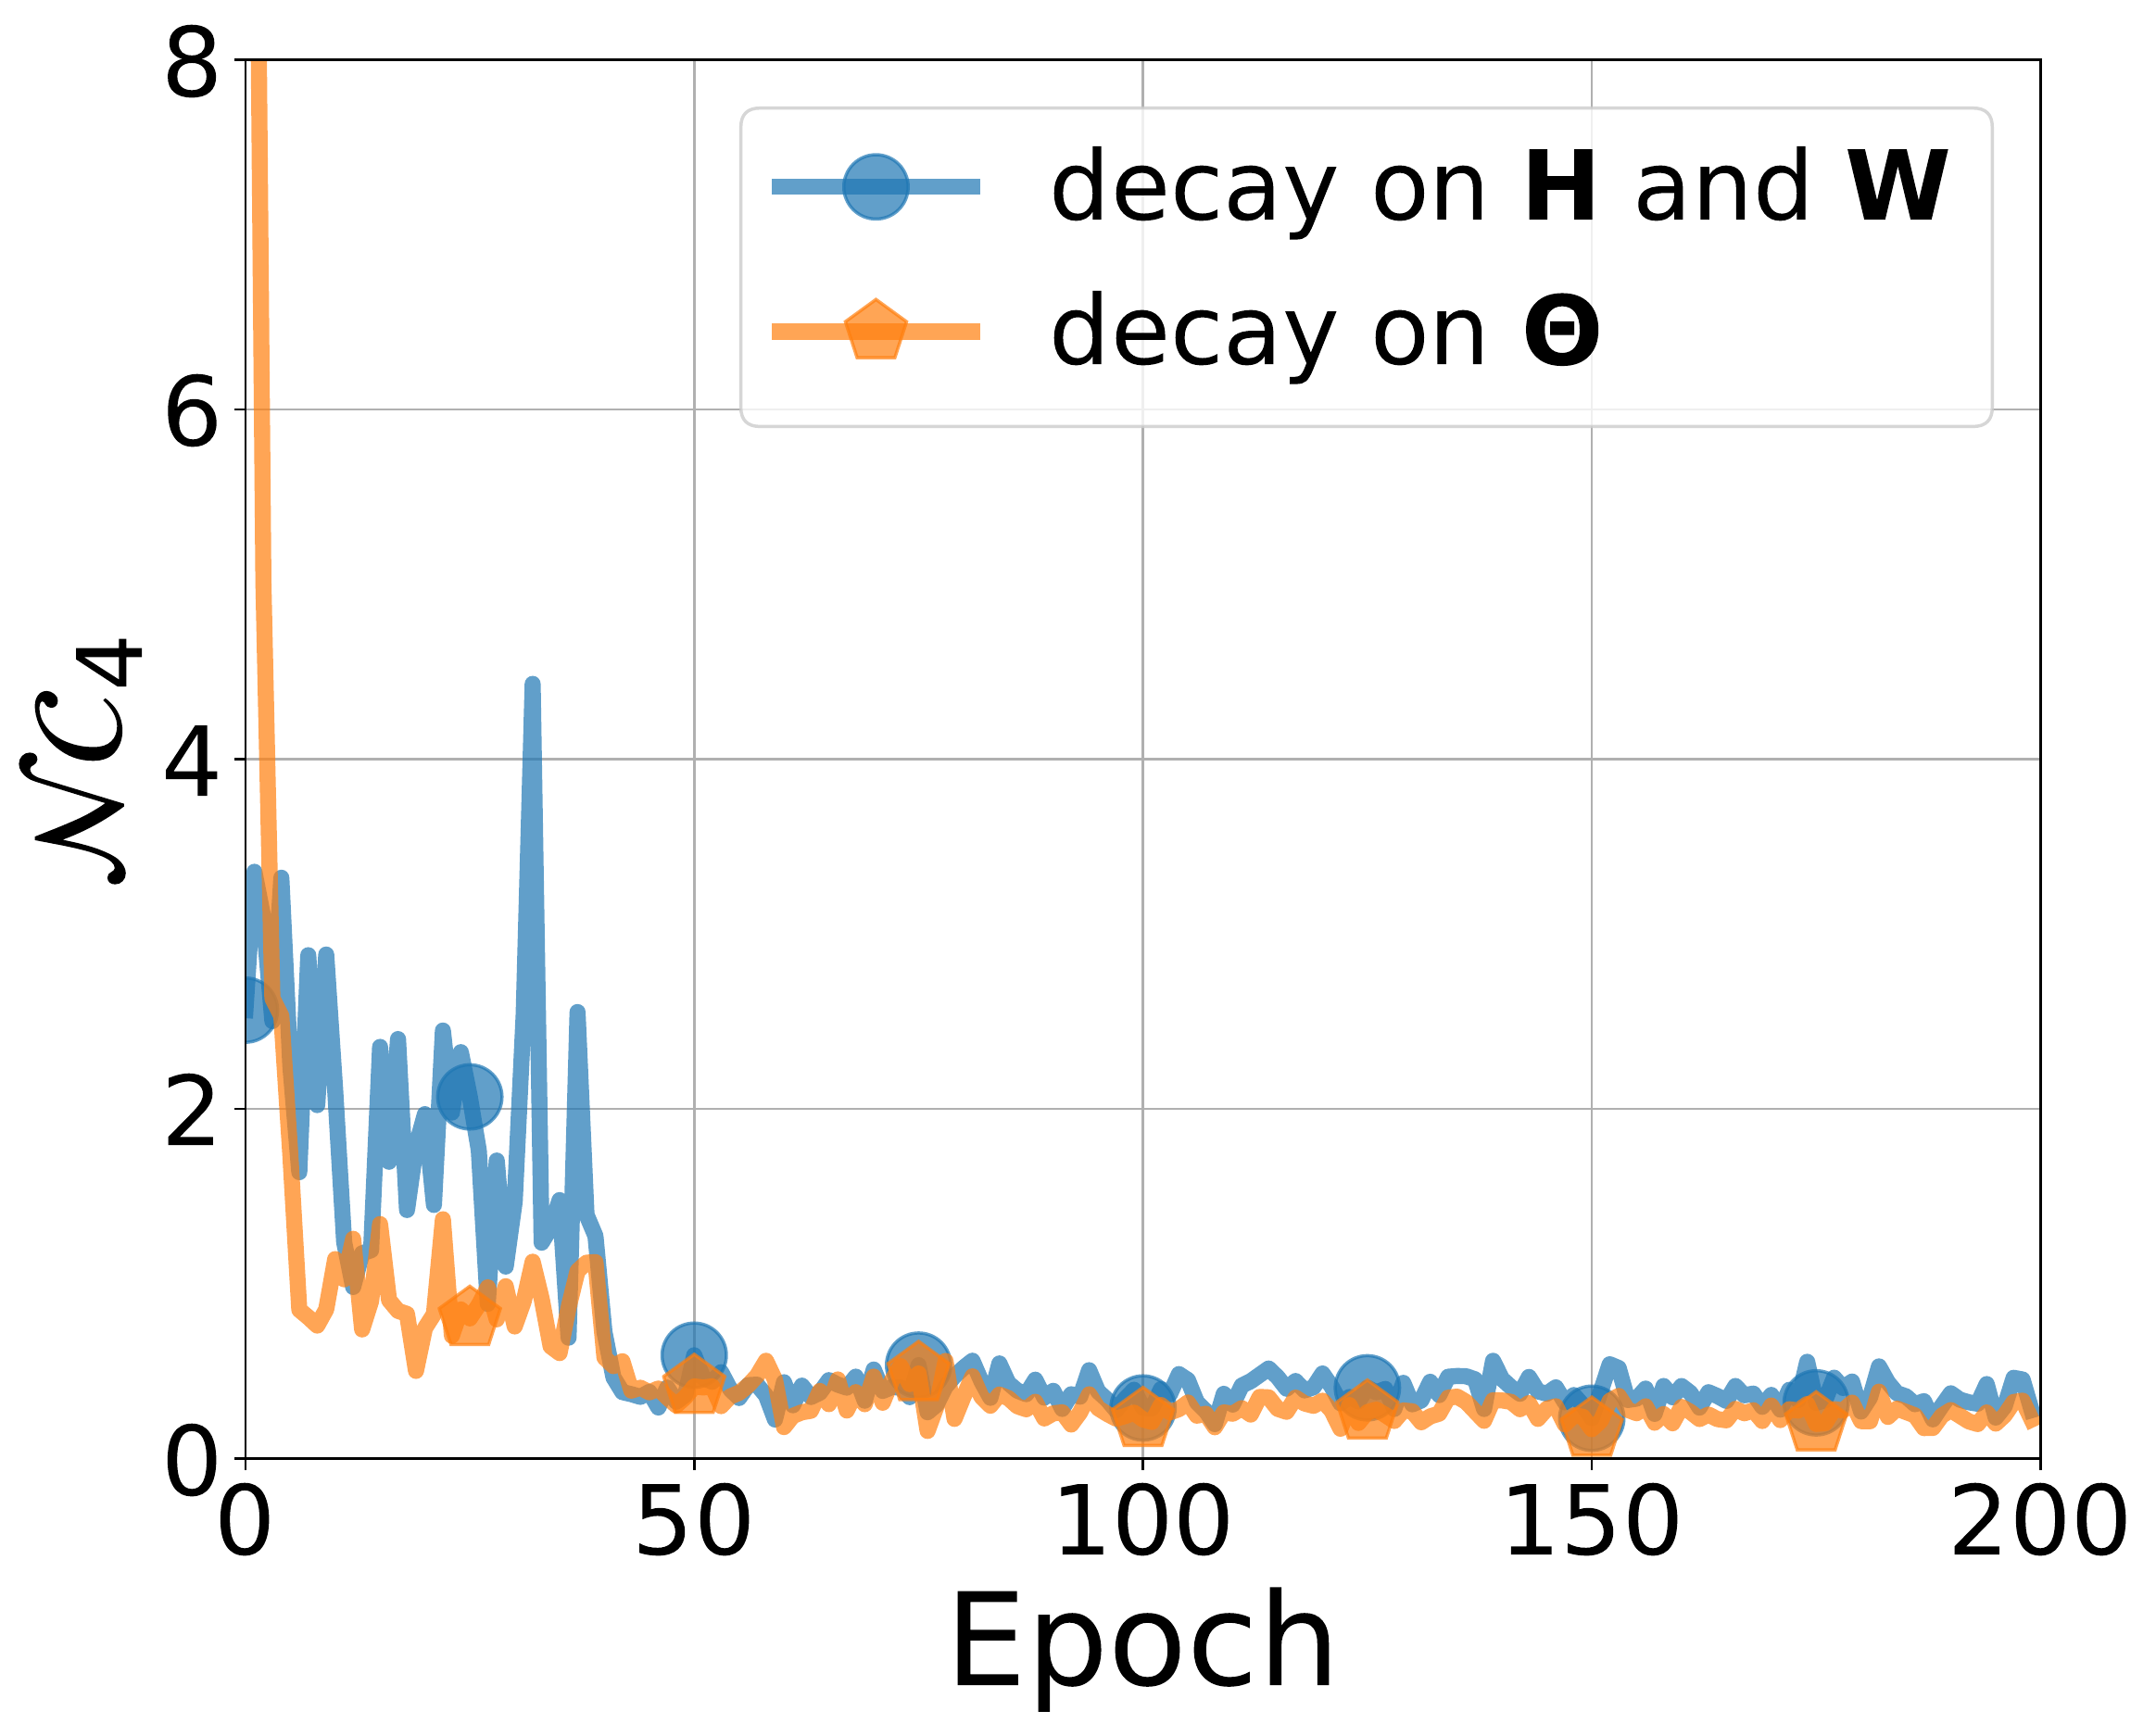}} \\
    
    \subfloat[$\mc {NC}_1$ (CIFAR10)]{\includegraphics[width=0.24\textwidth]{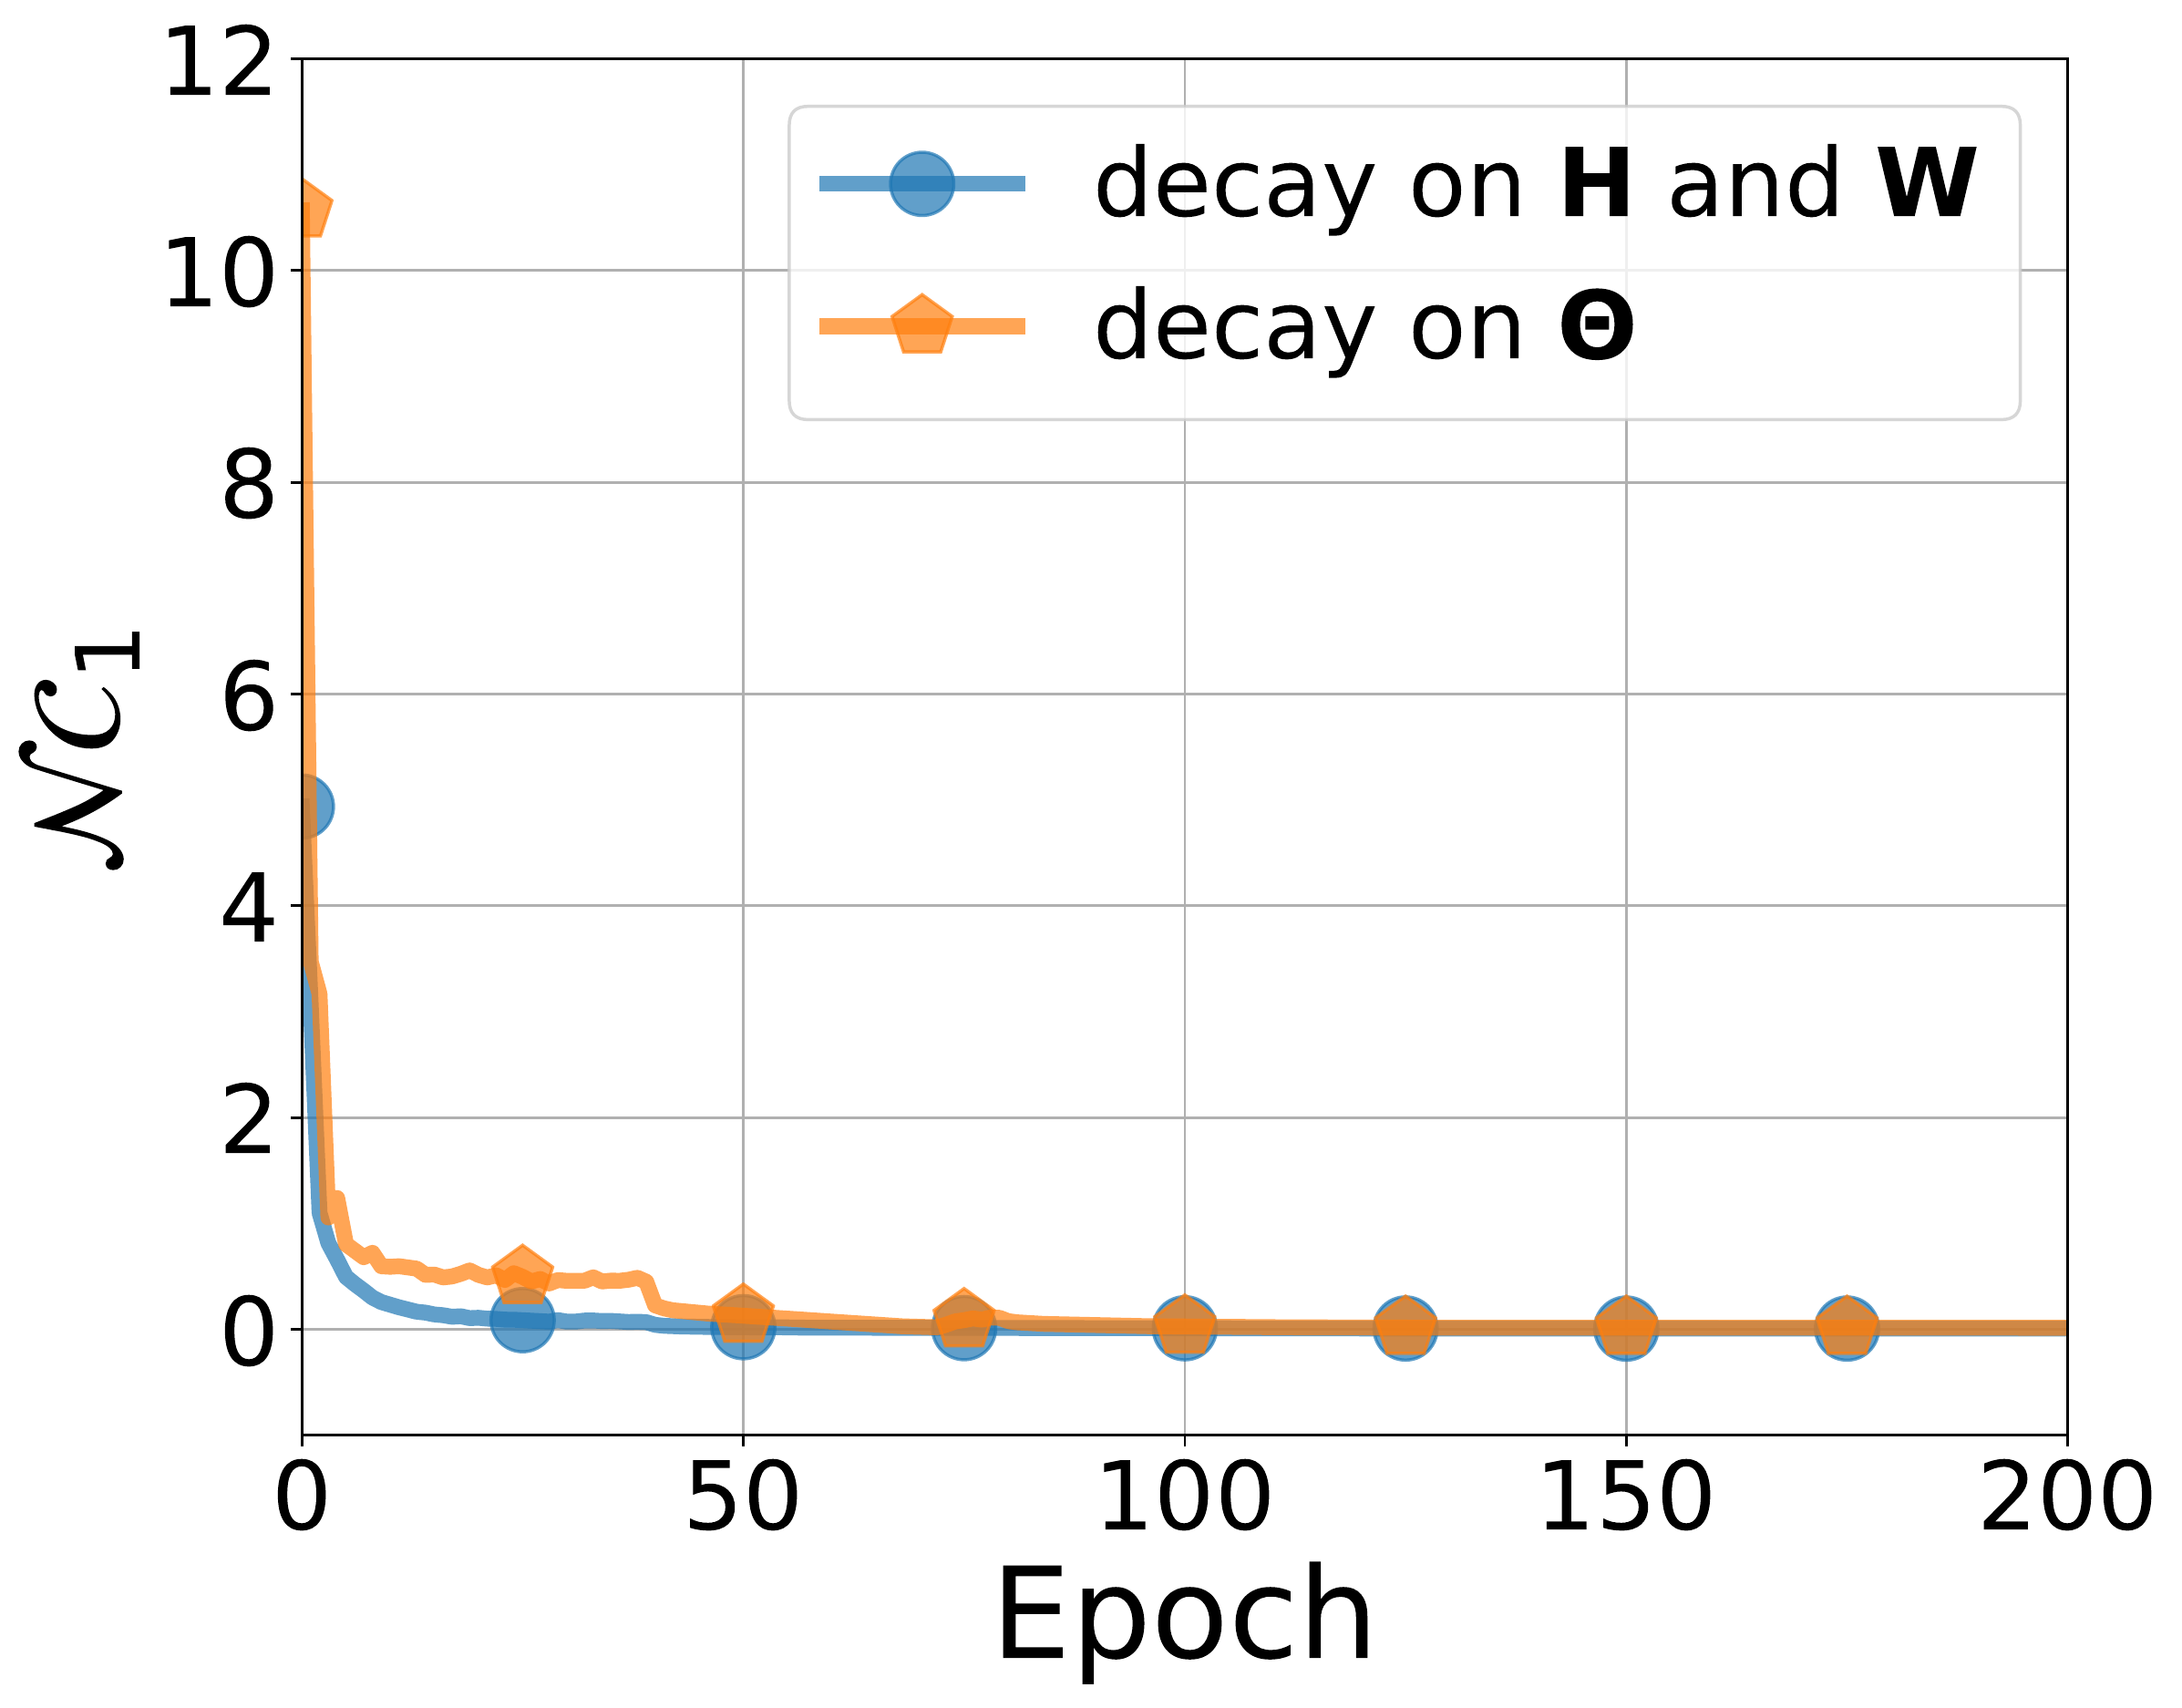}} \
    \subfloat[$\mc {NC}_2$ (CIFAR10)]{\includegraphics[width=0.24\textwidth]{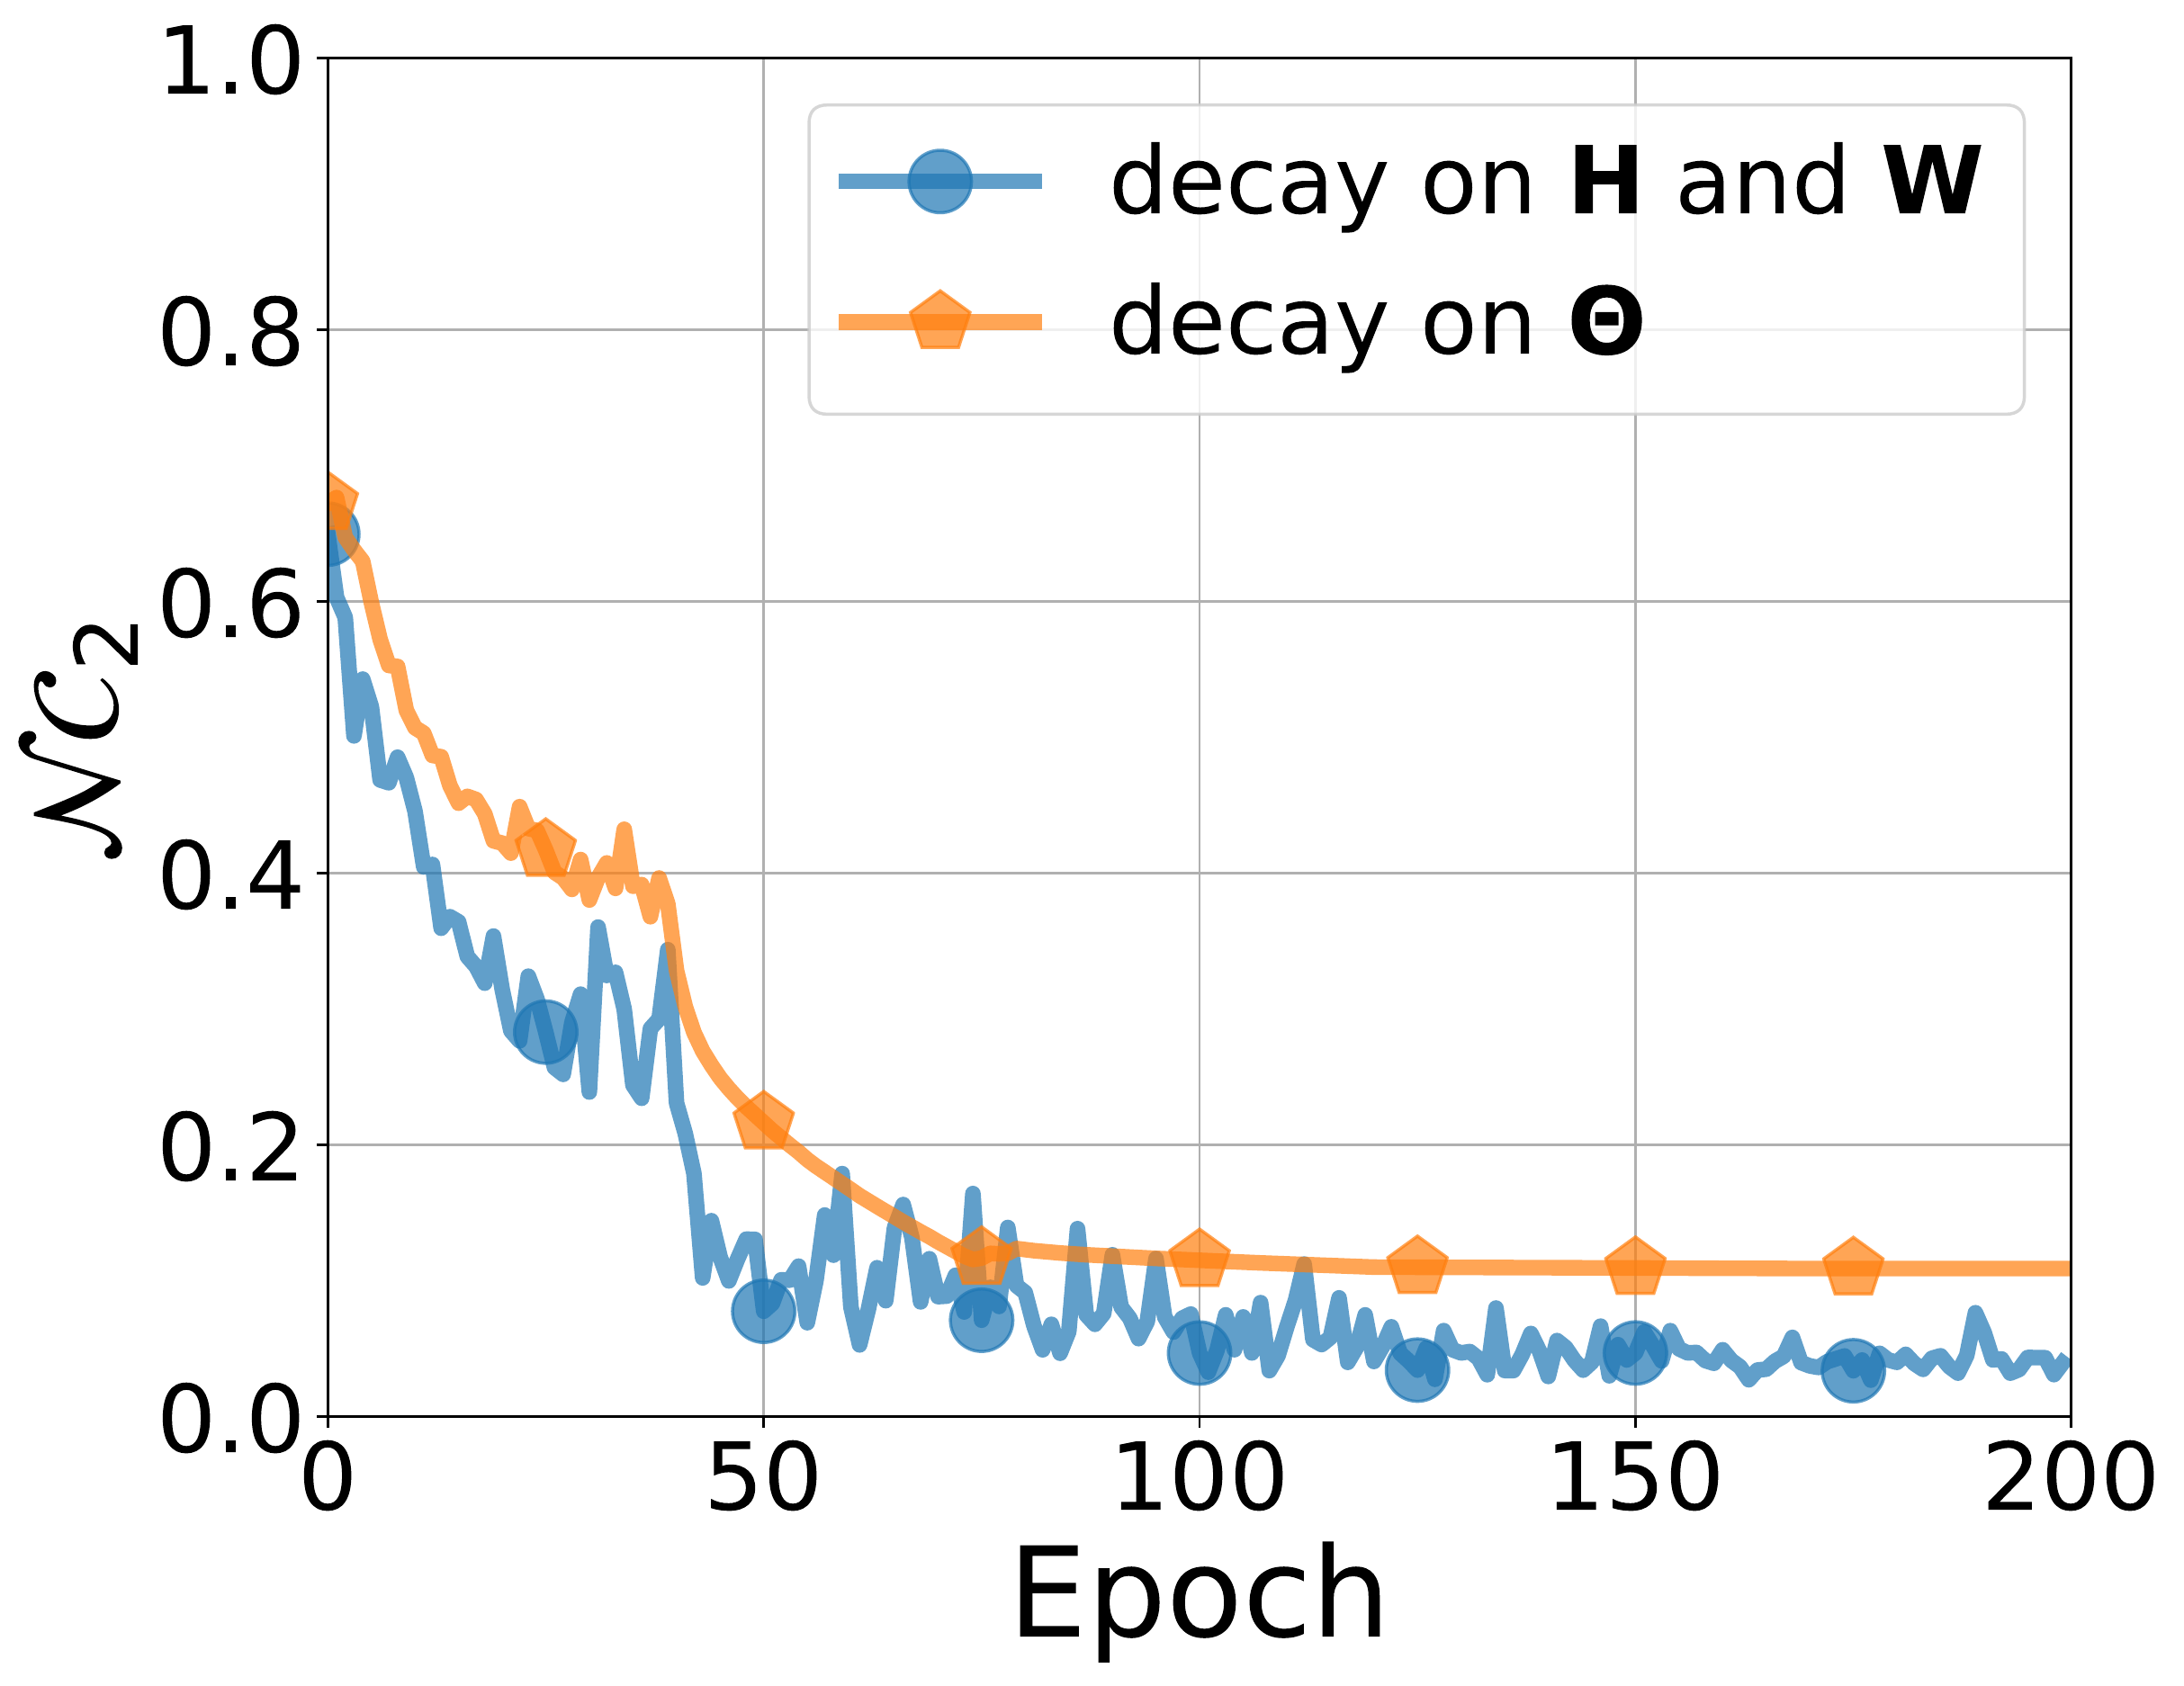}} \
    \subfloat[$\mc {NC}_3$ (CIFAR10)]{\includegraphics[width=0.24\textwidth]{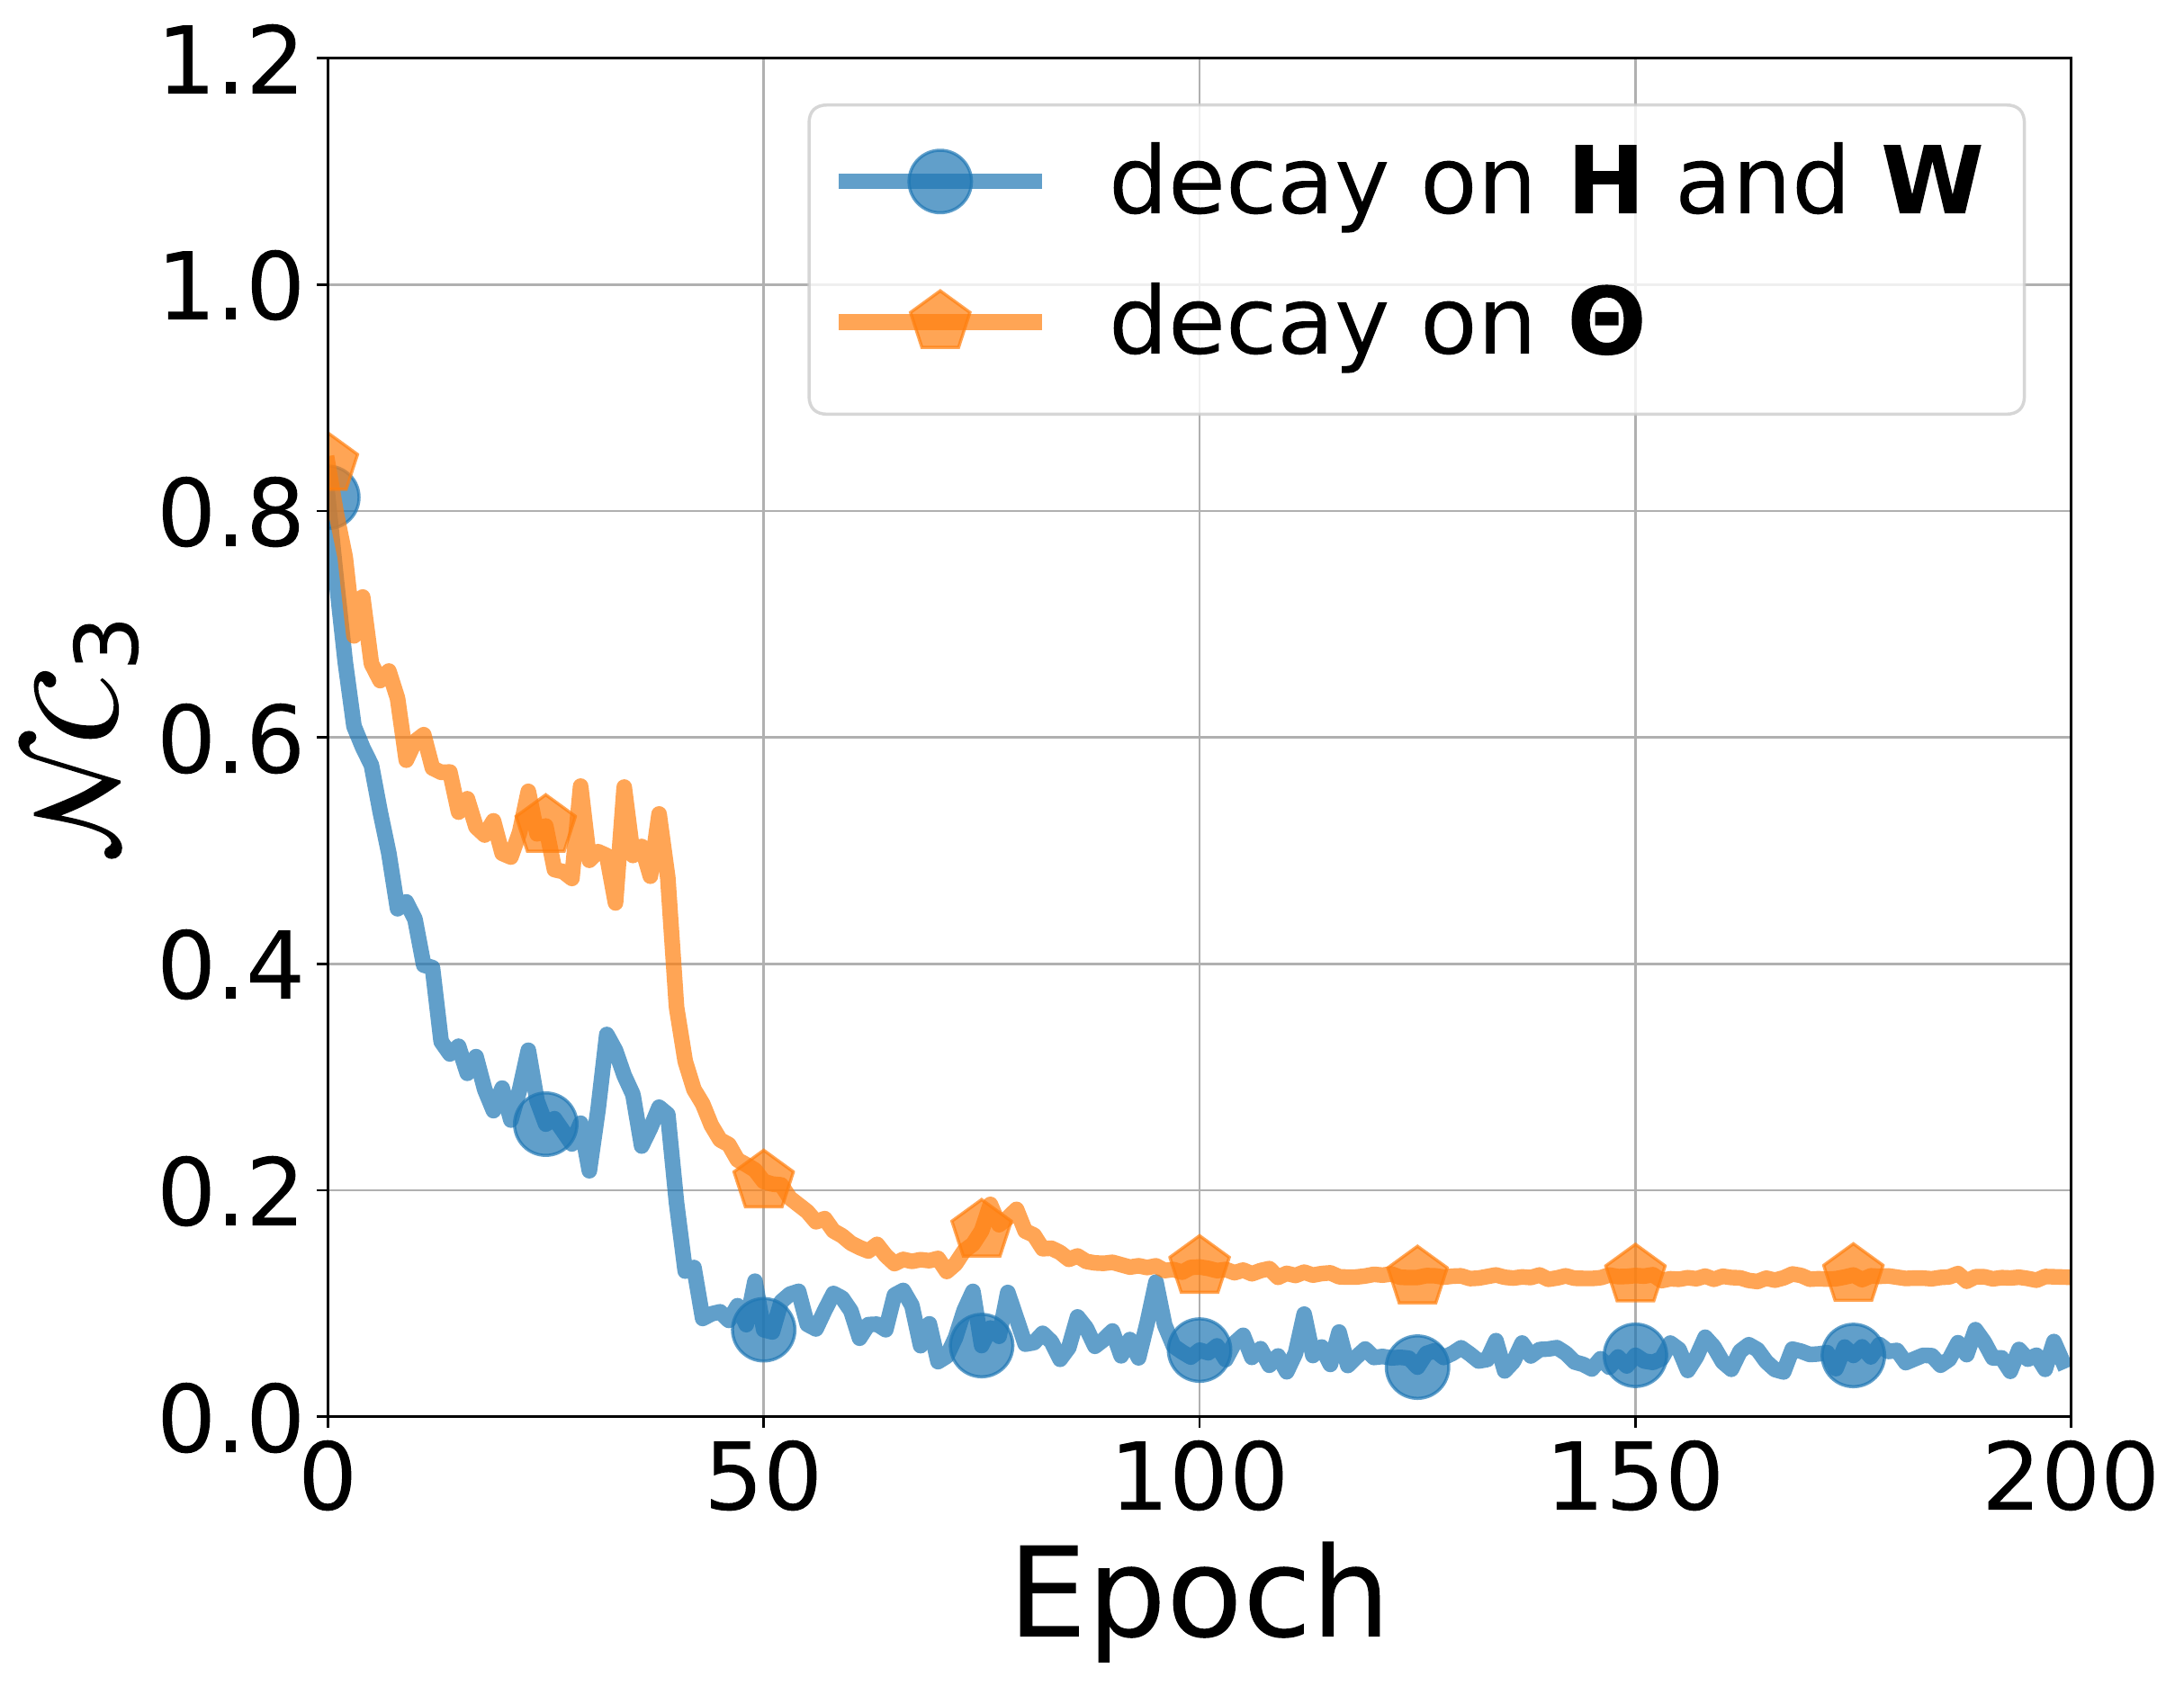}} \
    \subfloat[$\mc {NC}_4$ (CIFAR10)]{\includegraphics[width=0.23\textwidth]{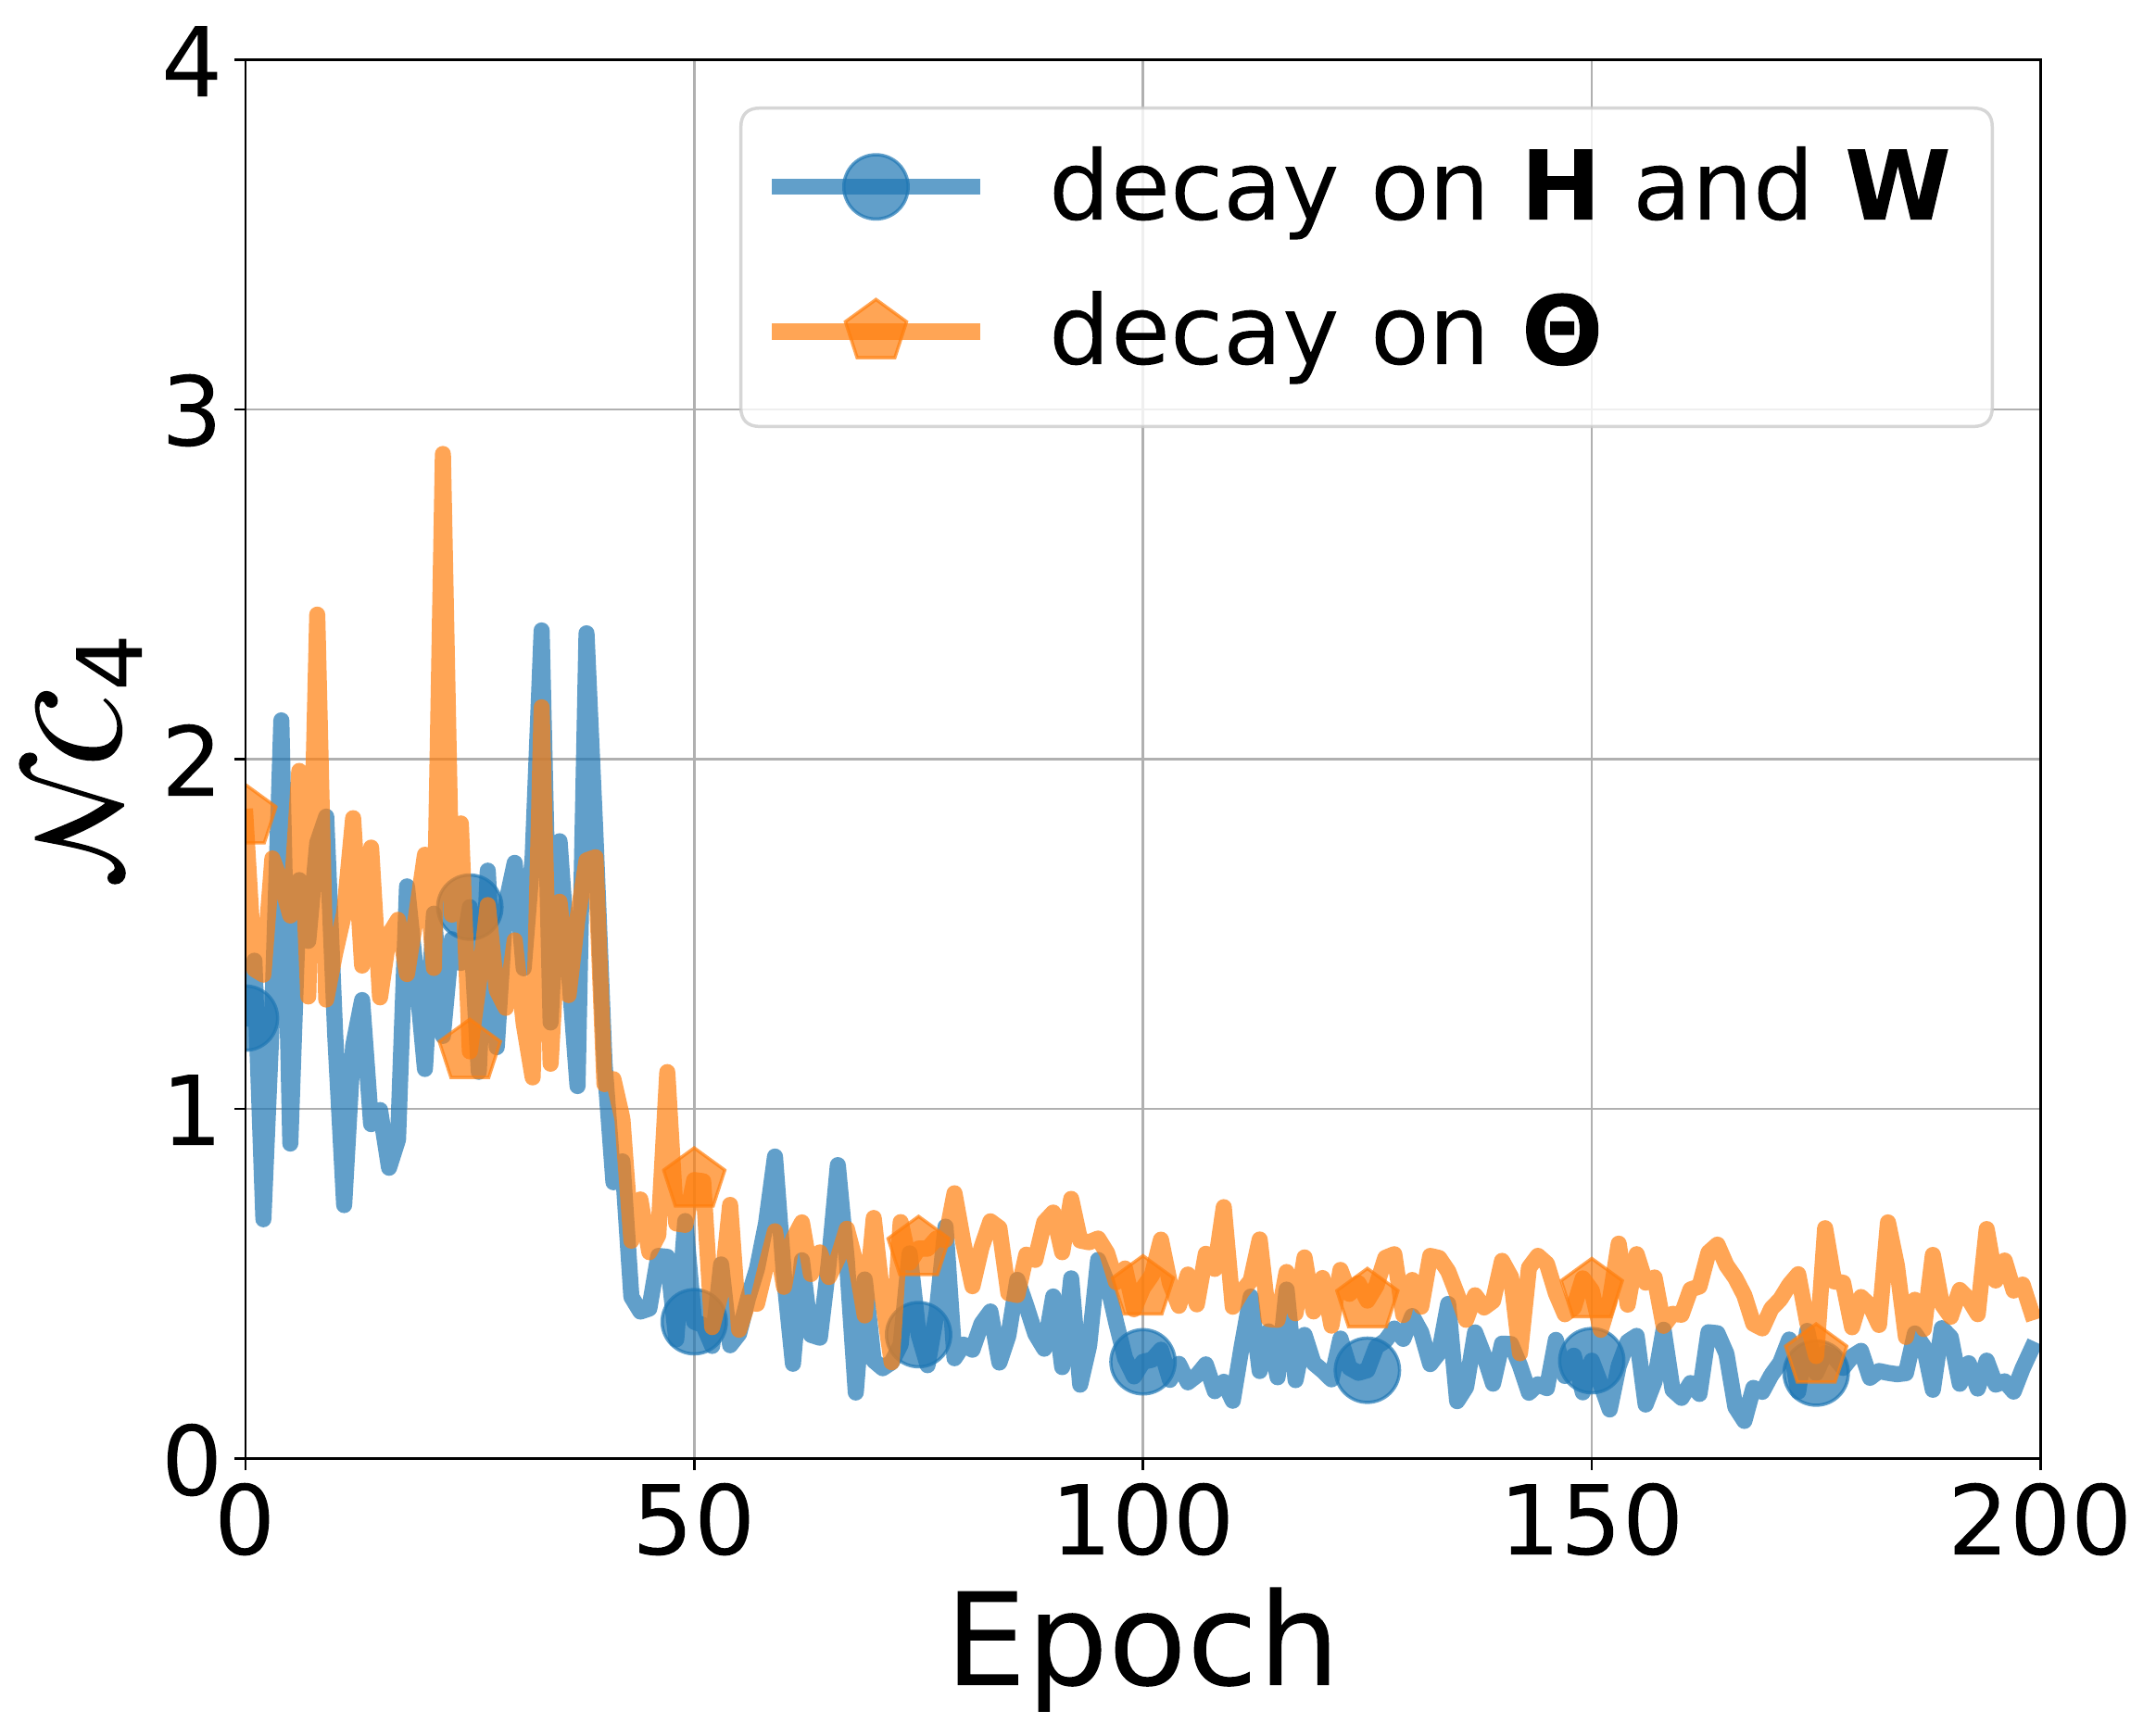}}
    \caption{\textbf{Comparison of \NC\;behavior for weight decay on $\mb \Theta$ vs. on $(\mb H,\mb W)$.}  For the latter set up, we choose $\lambda_{\mb W} = \lambda_{\mb b} = 0.01$ and $\lambda_{\mb H} = 0.00001$.
    }
    \label{fig:NC-WD}
\end{figure}

\subsection{Insights from \NC\ for Improving Network Designs}
%\label{sec:exp-fix-classifier}

Similar to \Cref{fig:fxied-classifier}, we train a ResNet18 and fix the weights in the last layer as a Simplex ETF throughout training for MNIST and CIFAR10 datasets, but without any data augmentation. \Cref{fig:fxied-classifier-appendix} presents a comparison of learned and fixed classifiers in terms of within-class variation collapse ($\mc {NC}_1$), self-duality ($\mc {NC}_3$), training accuracy, and test accuracy. The results in \Cref{fig:fxied-classifier-appendix} are consistent with those in \Cref{fig:fxied-classifier}, implying that the fixed classifier and setting $d = K$ exhibits the same within-class variation collapse for the feature $\mb H$, and achieves the same classification accuracy as the \emph{fully-trained} classifier with $d>K$.

\begin{figure}[t]
   \centering
    % \subfloat[$\mc {NC}_1$ (MNIST)]{\includegraphics[width=0.24\textwidth]{figs/resnet18/mnist-SGD-ETF-fixdim/mnist-resnet18-NC1.pdf}} \
    % % \subfloat[$\mc {NC}_2$ (MNIST)]{\includegraphics[width=0.32\textwidth]{figs/resnet18/mnist-SGD-ETF-fixdim/mnist-resnet18-NC2.pdf}} \
    % \subfloat[$\mc {NC}_3$ (MNIST)]{\includegraphics[width=0.24\textwidth]{figs/resnet18/mnist-SGD-ETF-fixdim/mnist-resnet18-NC3.pdf}} \
    % % \subfloat[$\mc {NC}_4$ (MNIST)]{\includegraphics[width=0.32\textwidth]{figs/resnet18/mnist-SGD-ETF-fixdim/mnist-resnet18-NC4.pdf}} \
    % \subfloat[Training Error]{\includegraphics[width=0.24\textwidth]{figs/resnet18/mnist-SGD-ETF-fixdim/mnist-resnet18-train-acc.pdf}} \
    % \subfloat[Test Error]{\includegraphics[width=0.24\textwidth]{figs/resnet18/mnist-SGD-ETF-fixdim/mnist-resnet18-test-acc.pdf}} \\
        \subfloat[MNIST-ResNet18 (from left to right): $\mc {NC}_1$, $\mc {NC}_3$, Training Accuracy, Testing Accuracy]{\includegraphics[width=0.24\textwidth]{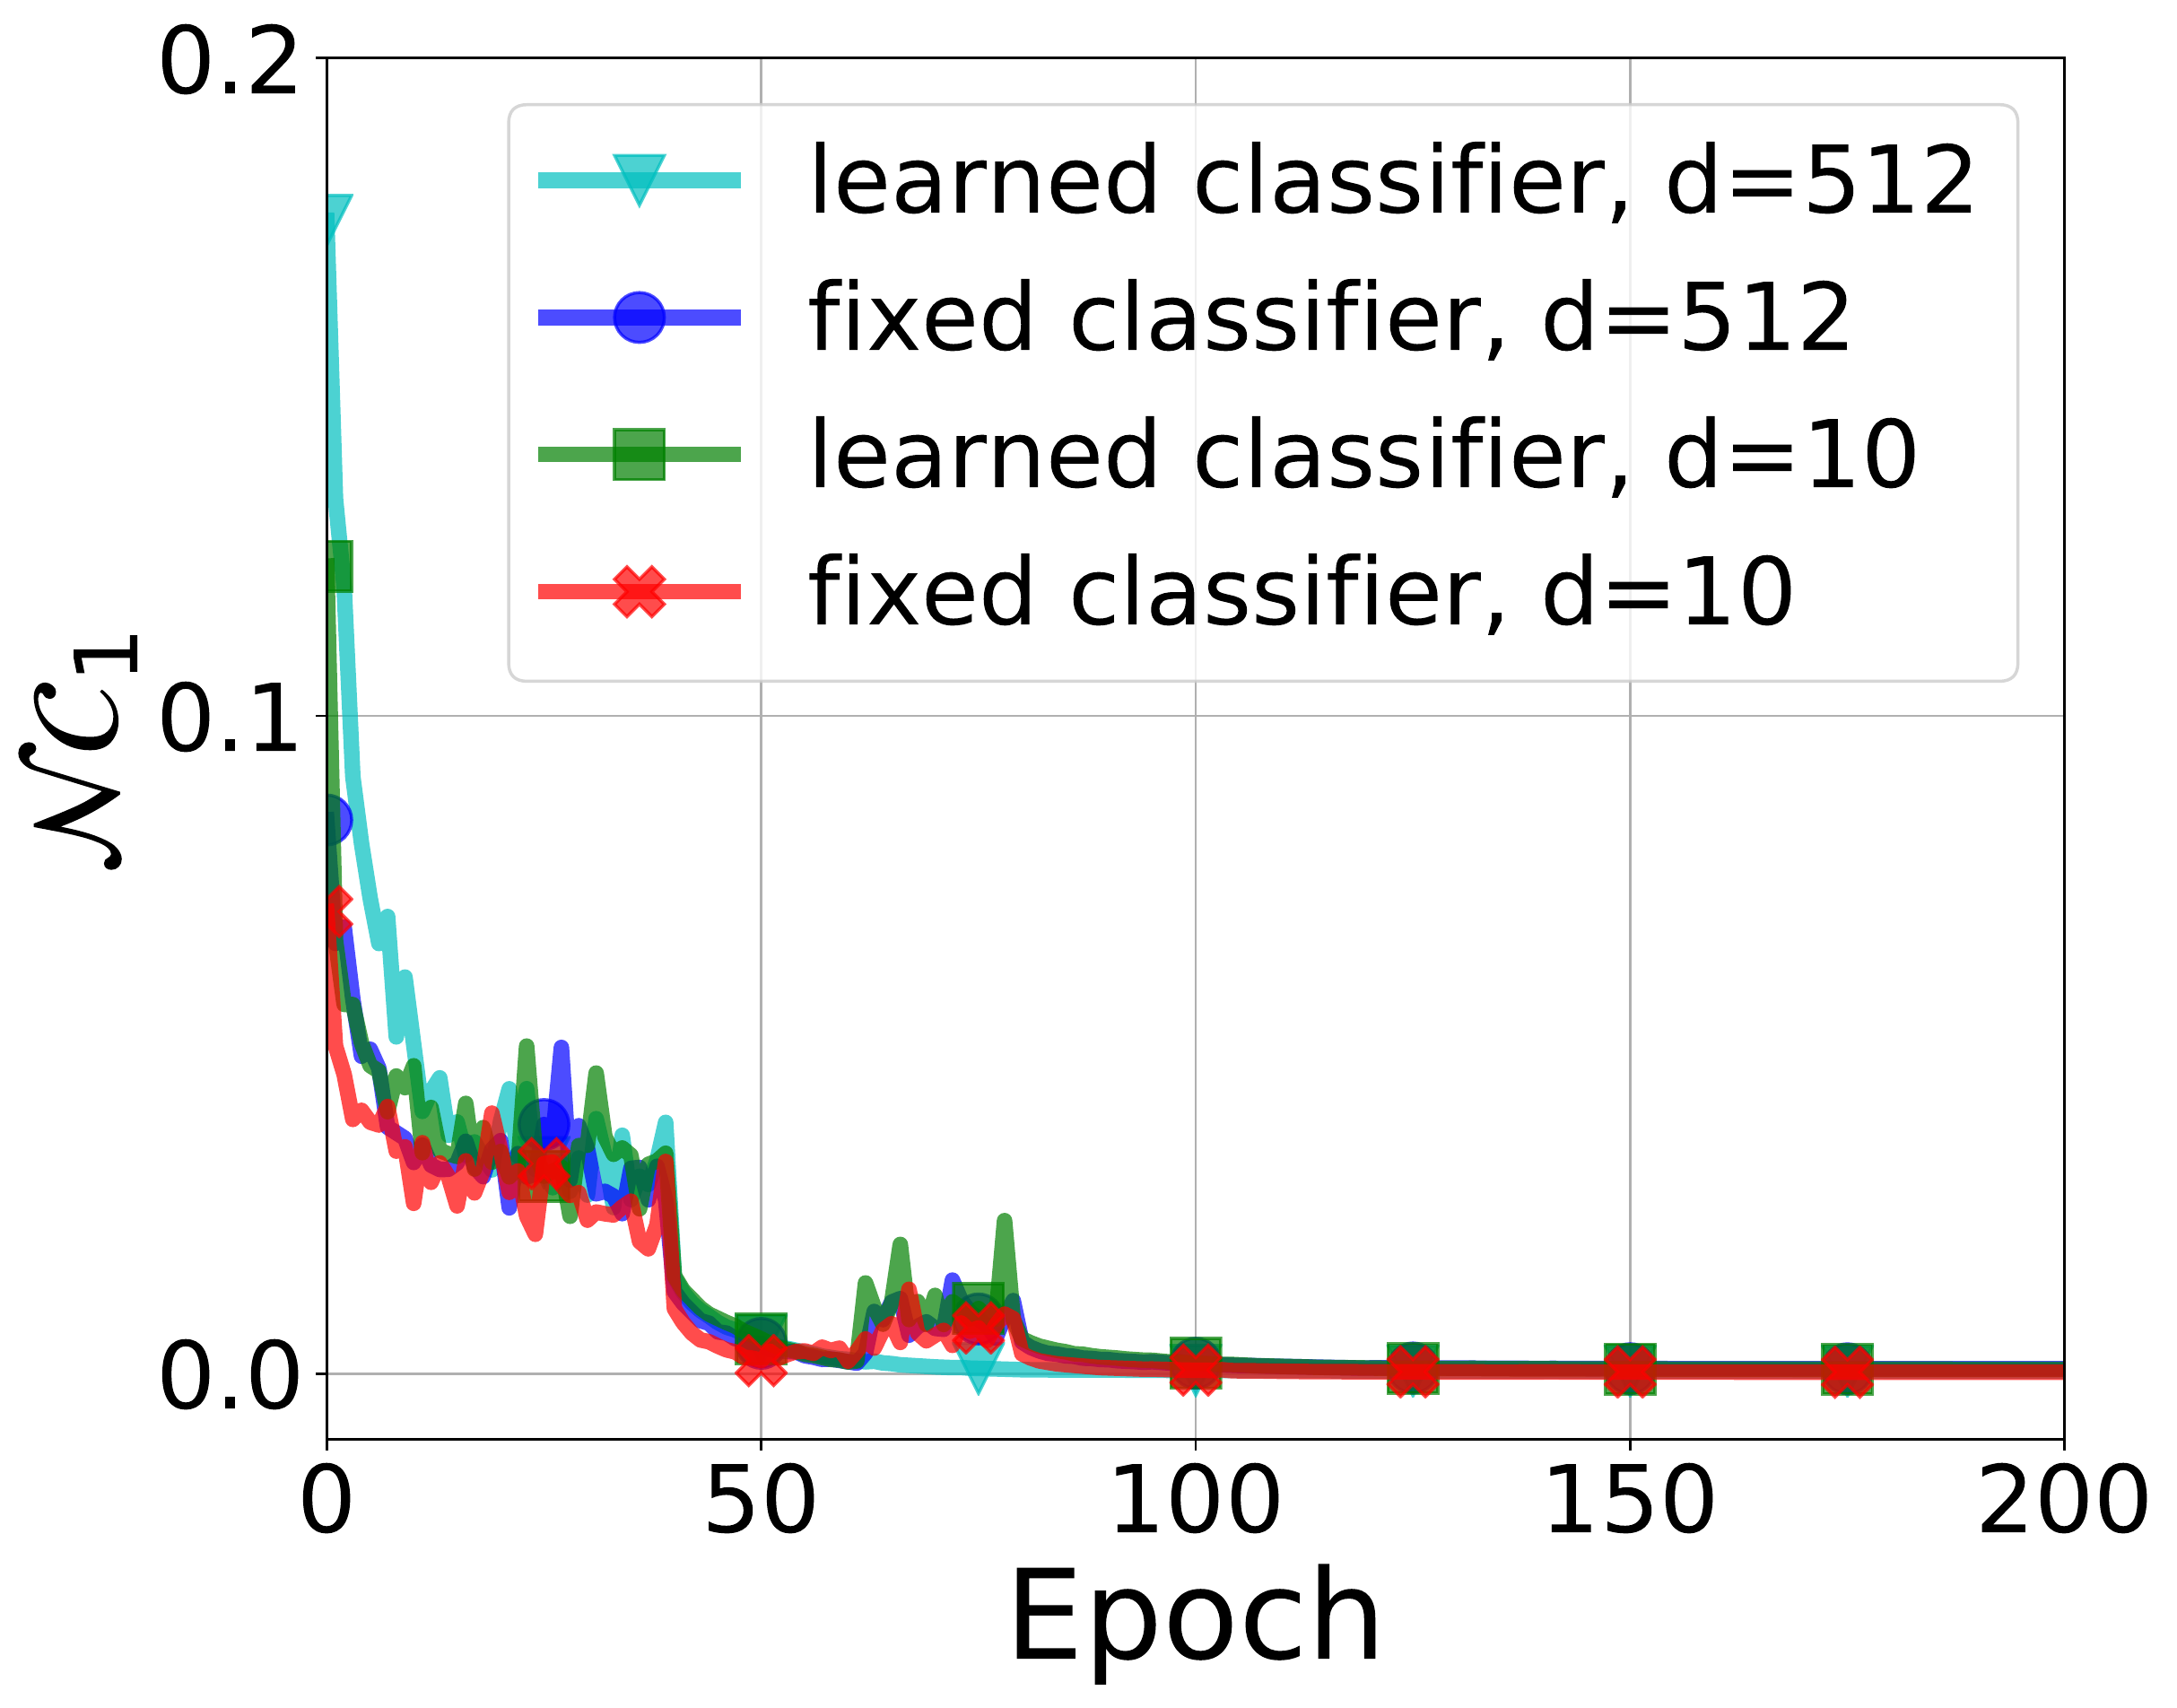} 
    % \subfloat[$\mc {NC}_2$ (MNIST)]{\includegraphics[width=0.32\textwidth]{figs/resnet18/mnist-SGD-ETF-fixdim/mnist-resnet18-NC2.pdf}} \
    \includegraphics[width=0.24\textwidth]{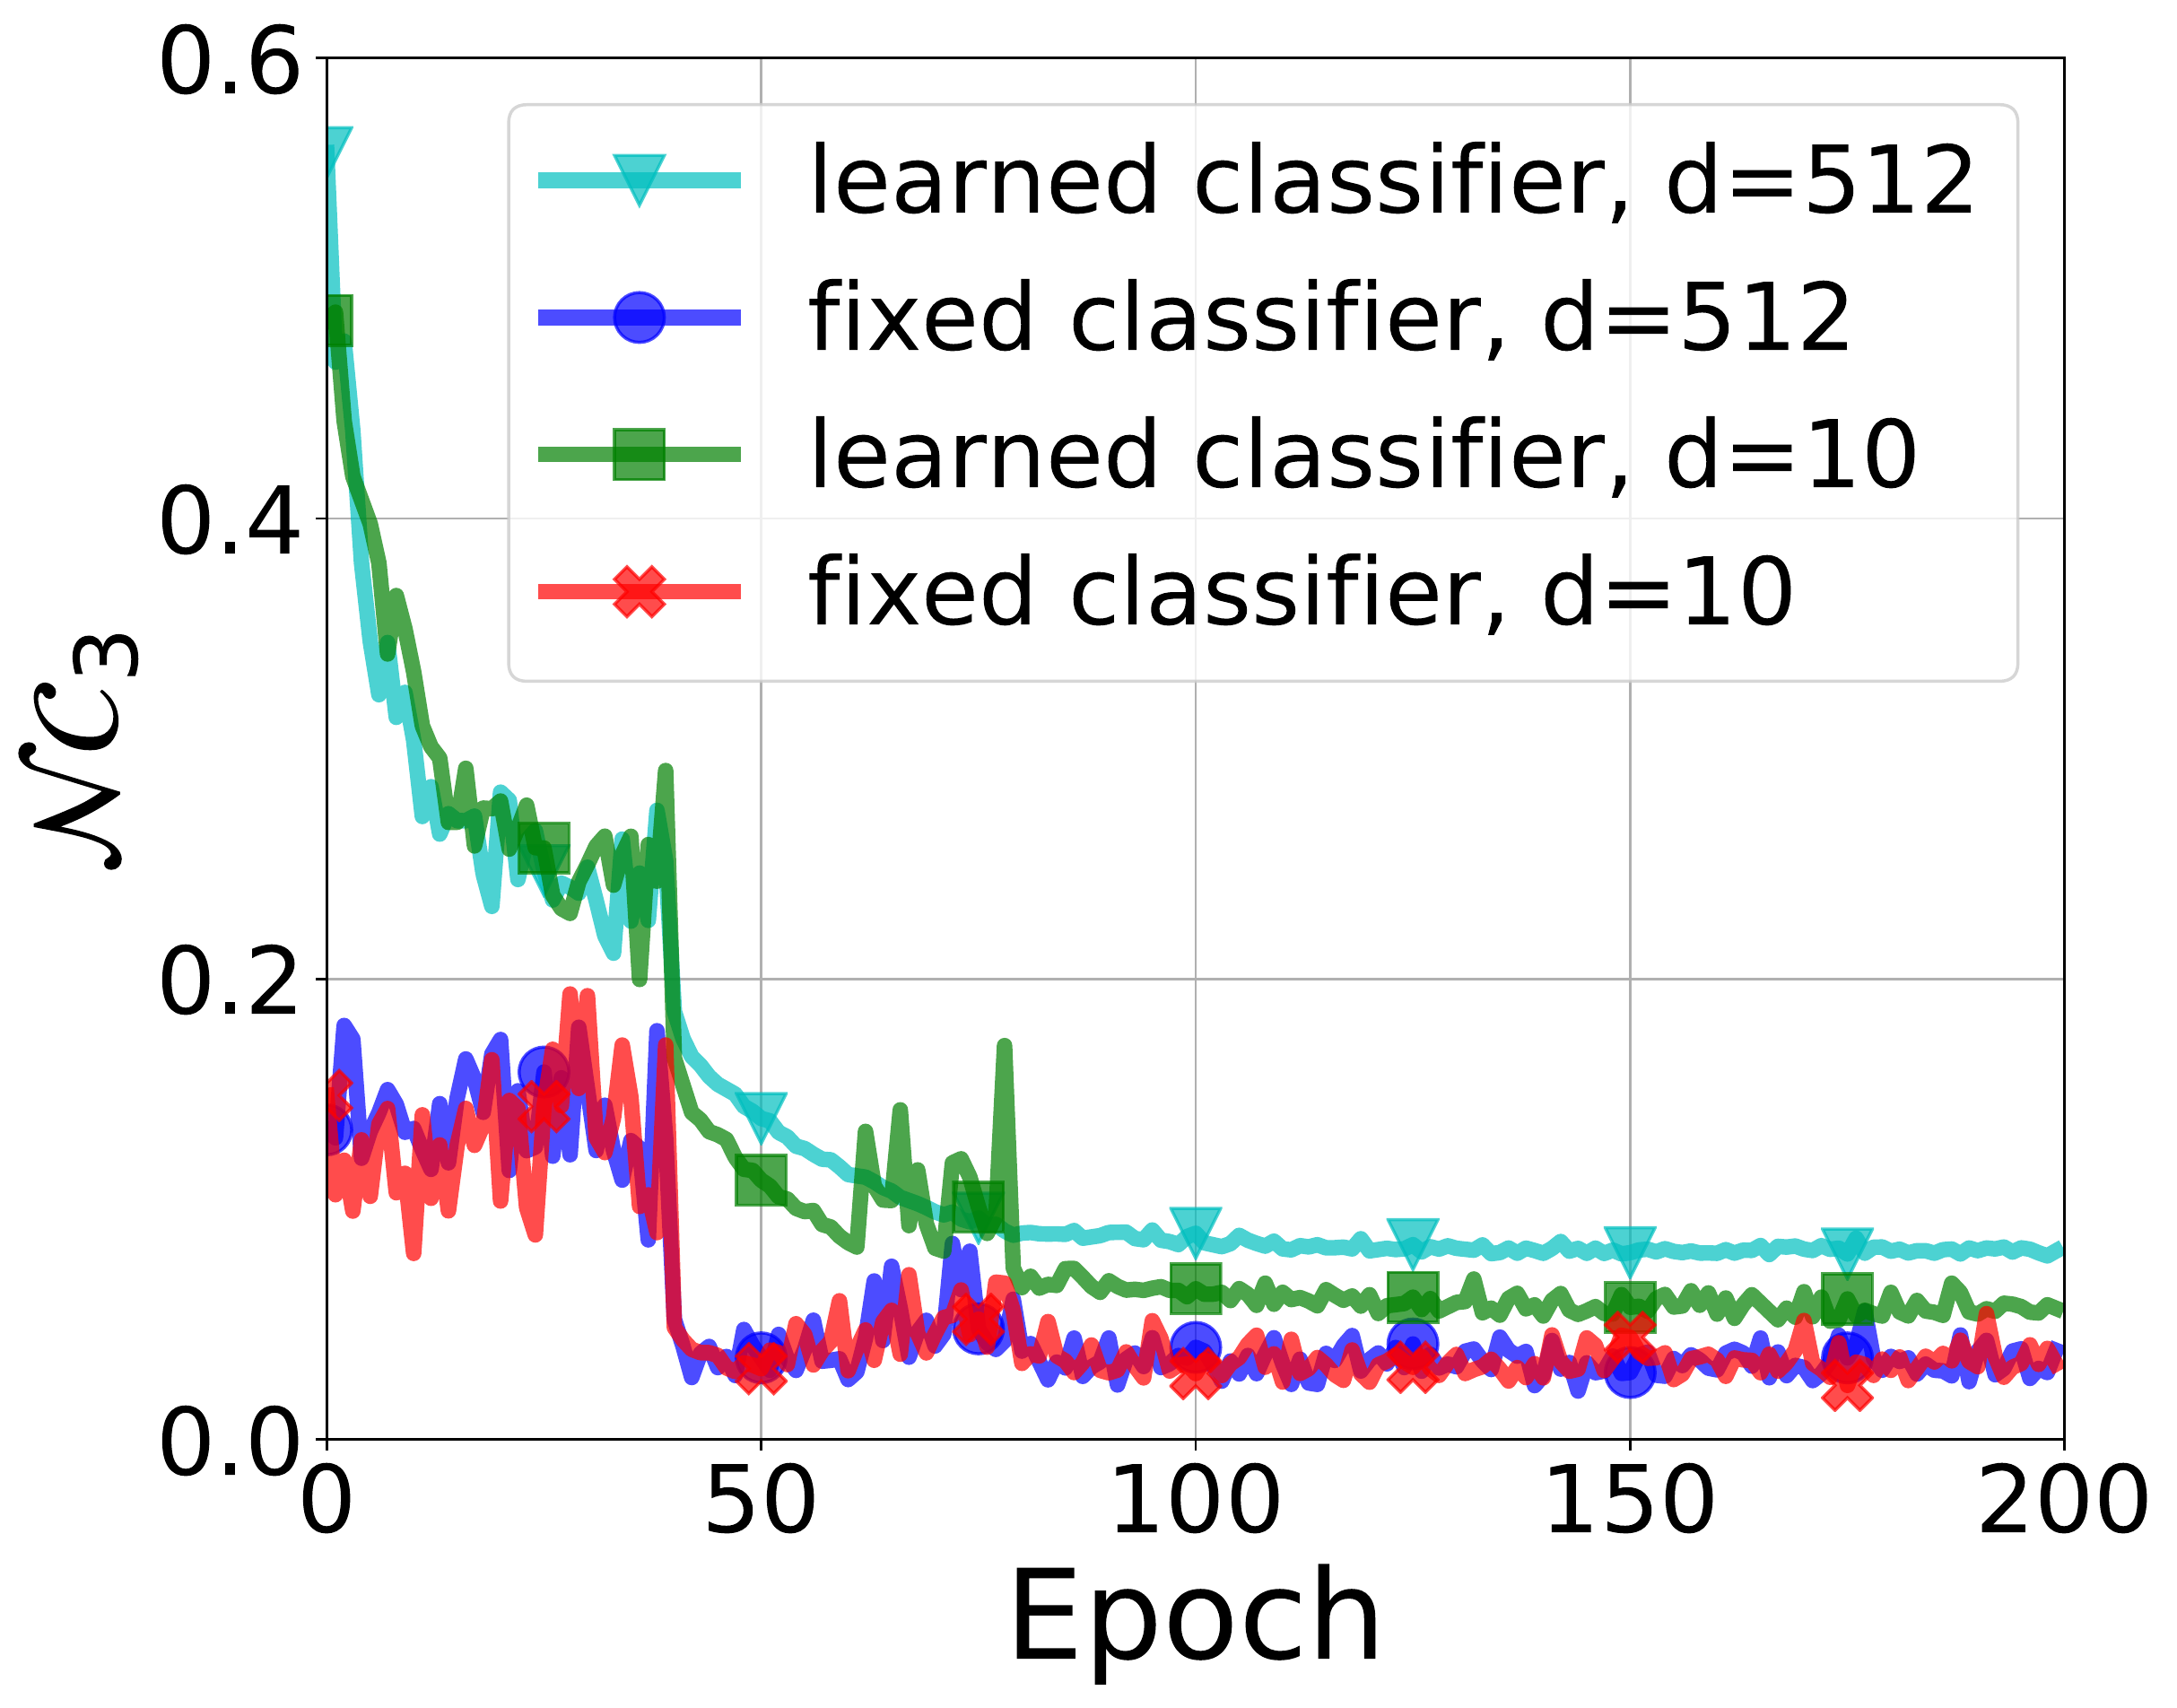} \
    % \subfloat[$\mc {NC}_4$ (MNIST)]{\includegraphics[width=0.32\textwidth]{figs/resnet18/mnist-SGD-ETF-fixdim/mnist-resnet18-NC4.pdf}} \
    \includegraphics[width=0.24\textwidth]{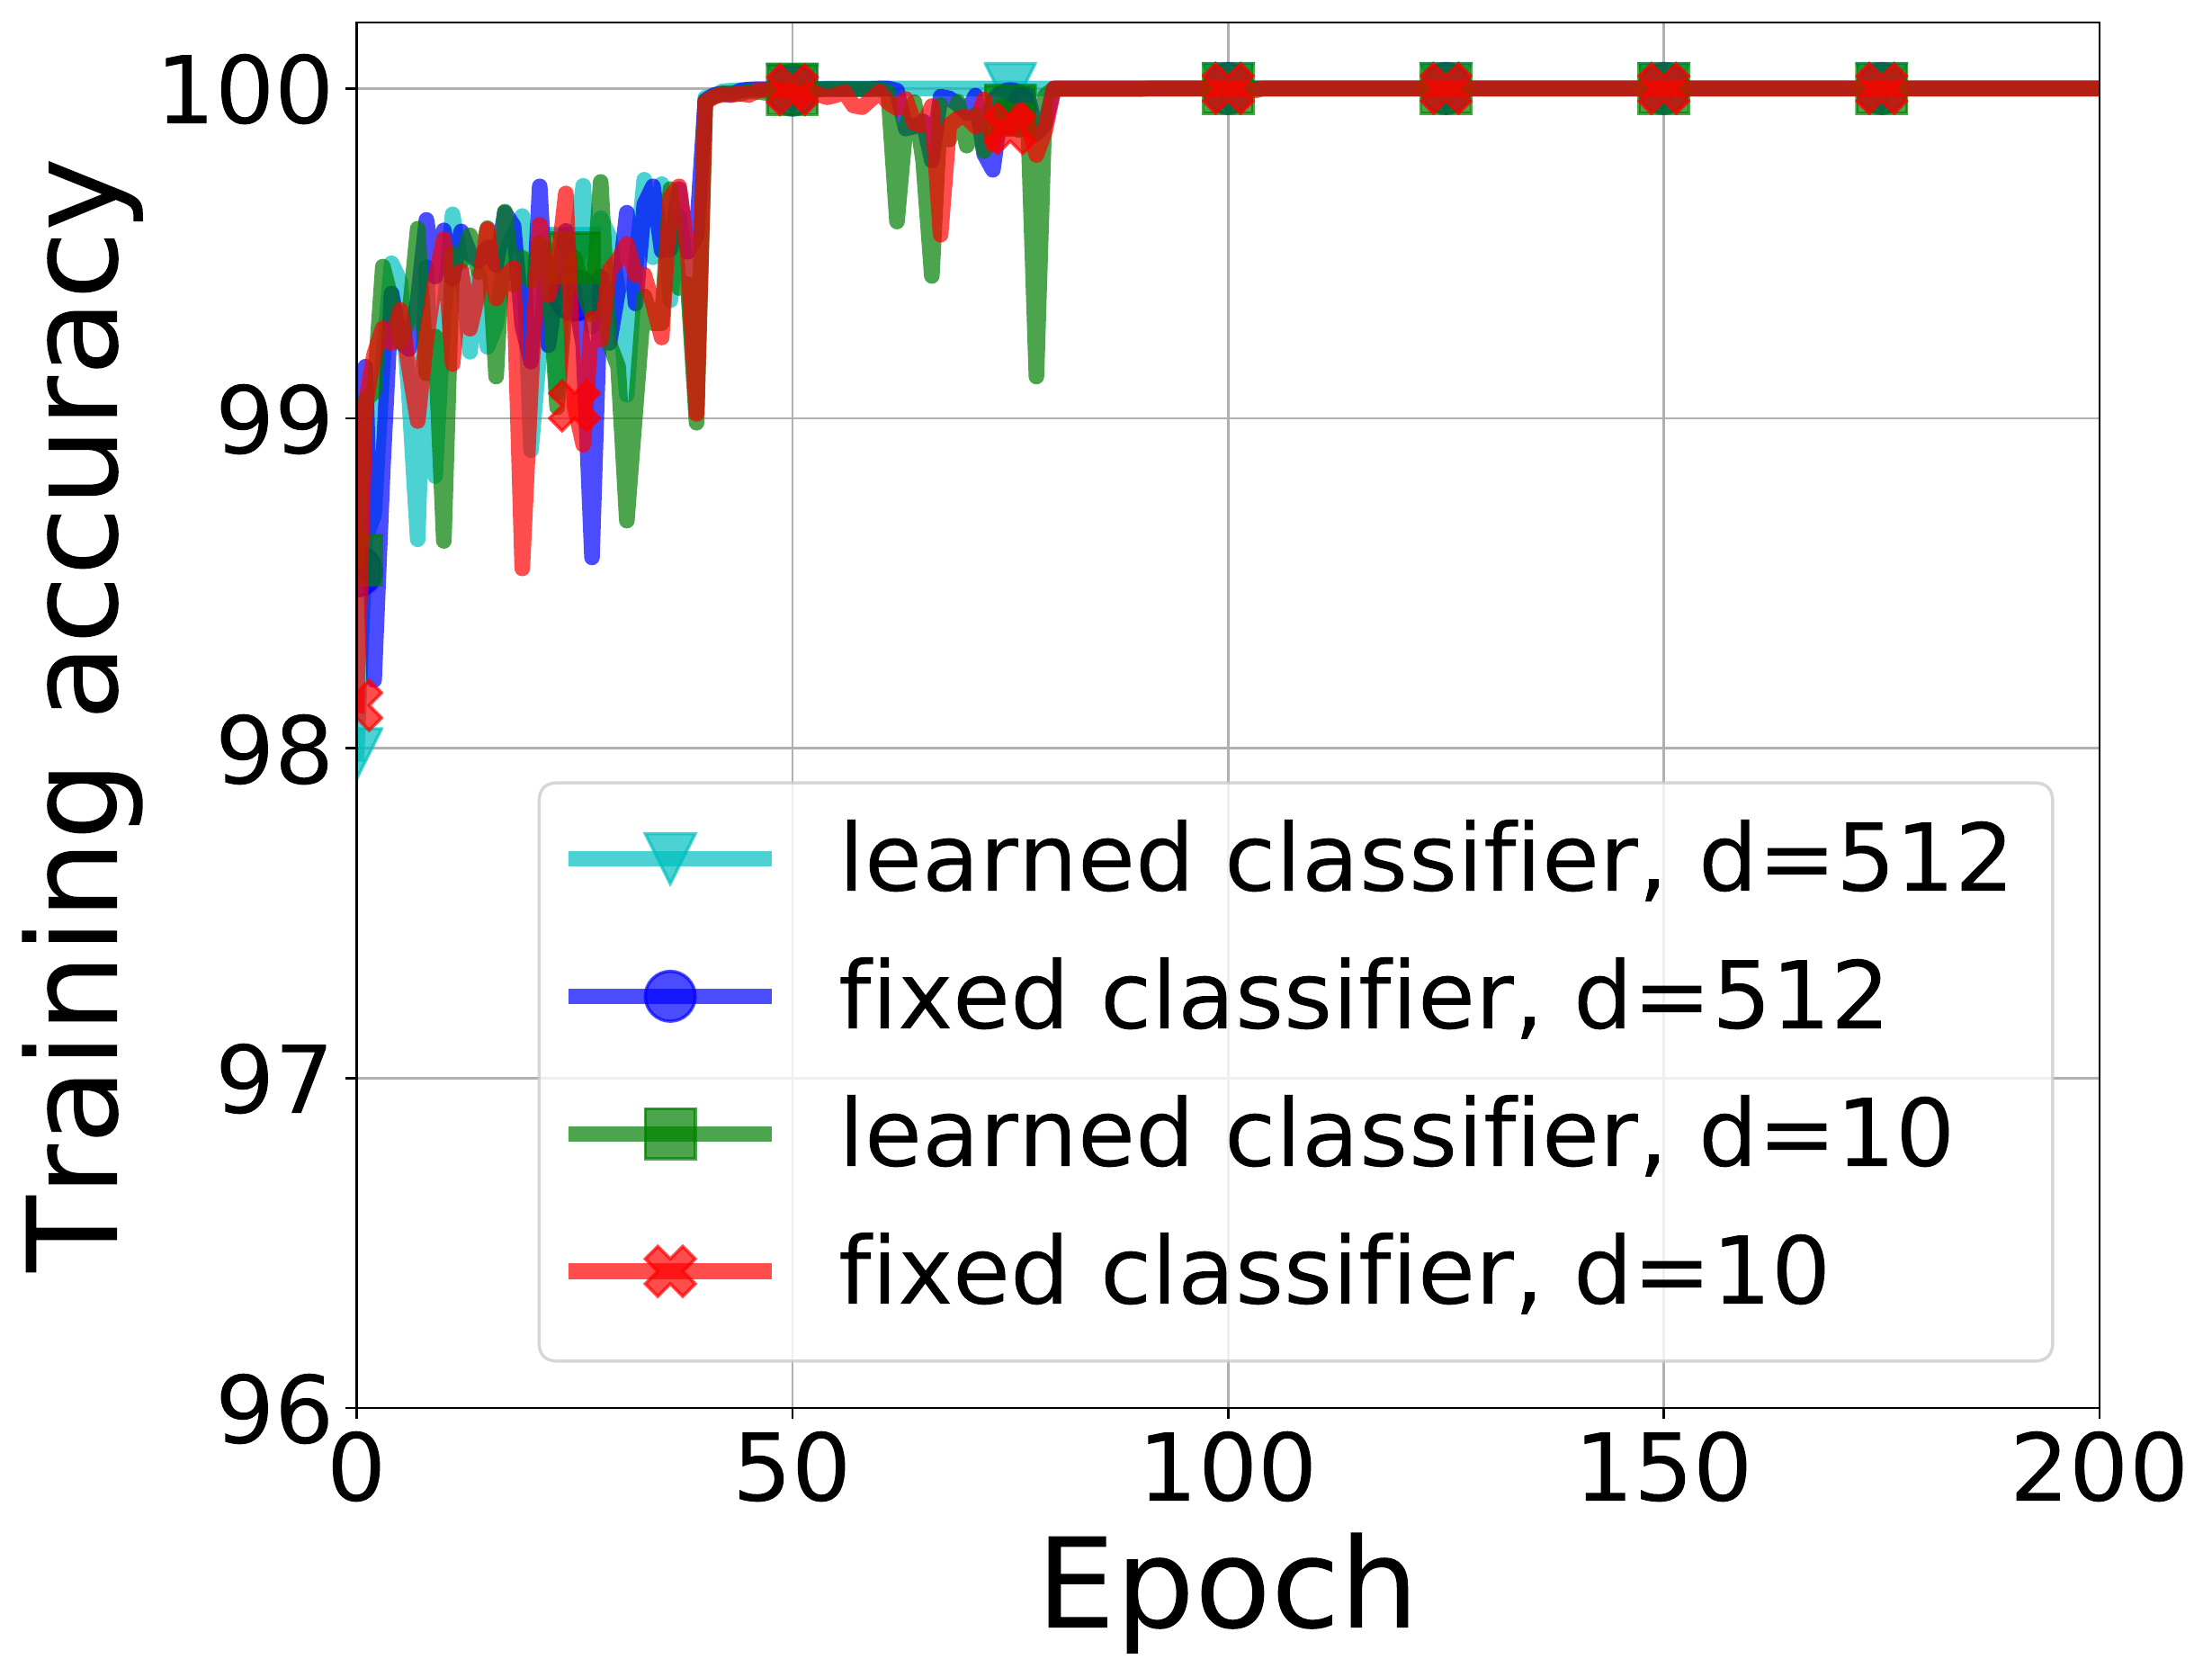} \
   \includegraphics[width=0.24\textwidth]{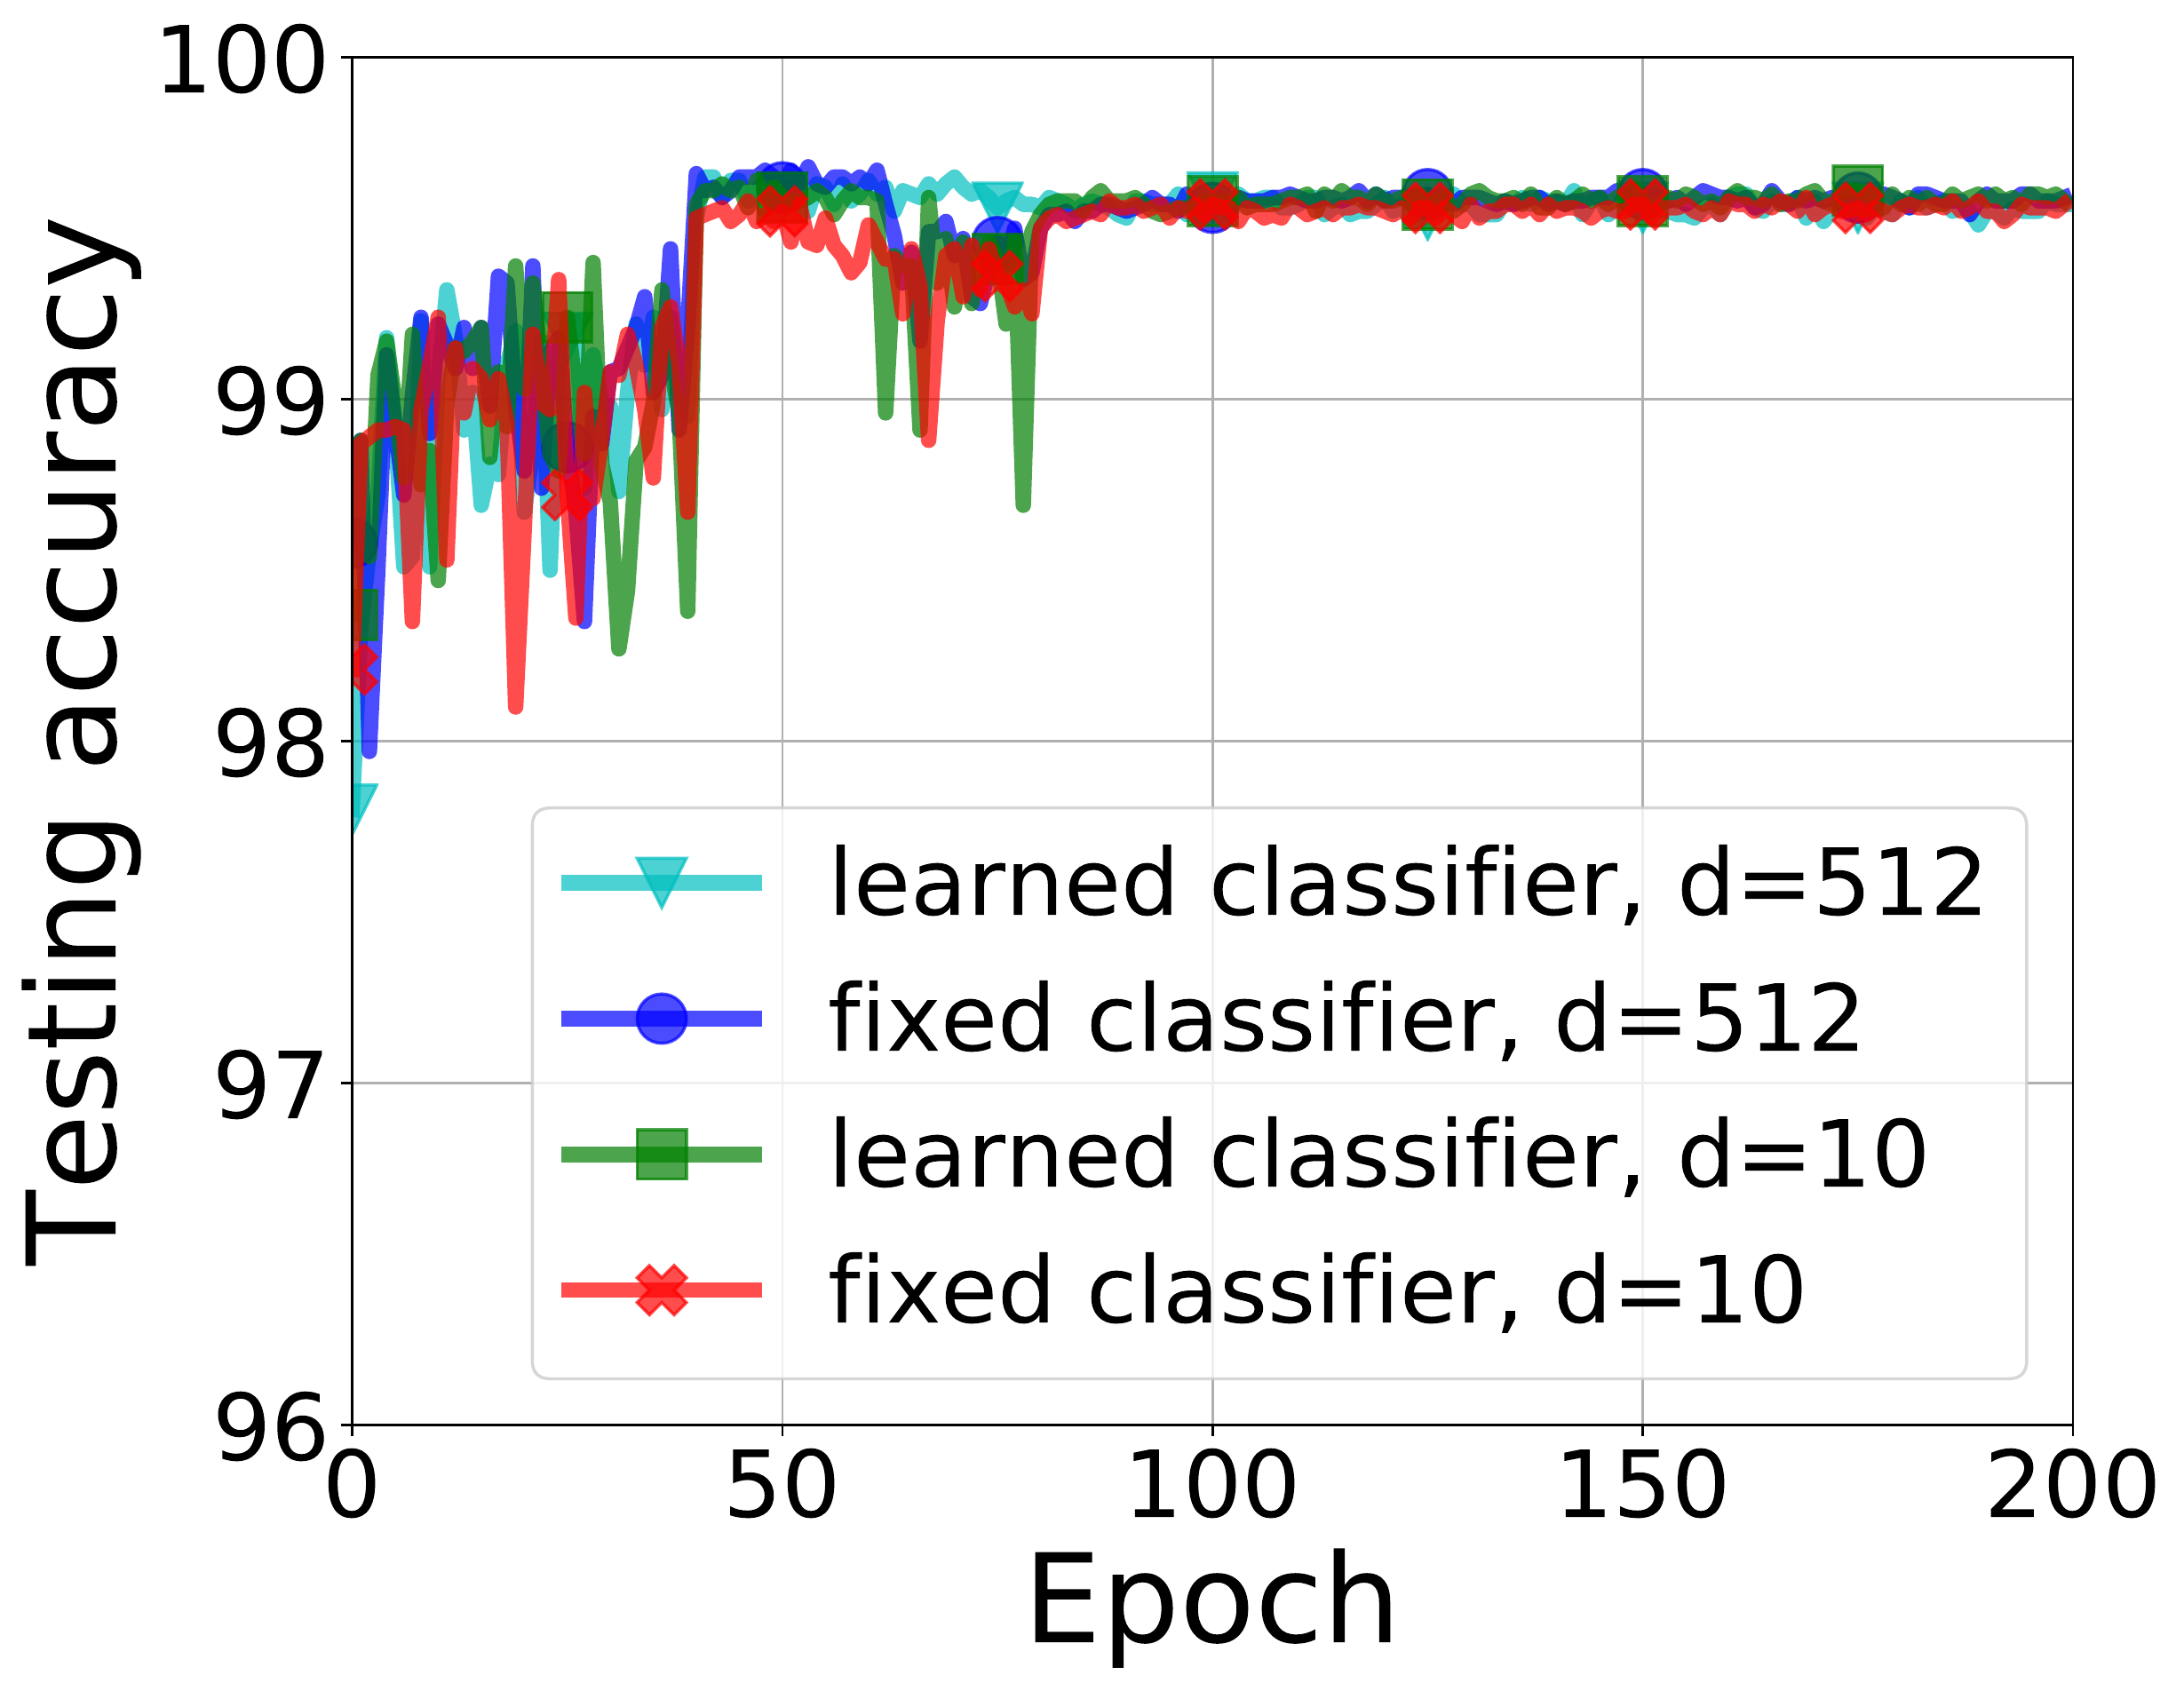}} \\
    \subfloat[CIFAR10-ResNet18 (from left to right): $\mc {NC}_1$, $\mc {NC}_3$, Training Accuracy, Testing Accuracy]{\includegraphics[width=0.24\textwidth]{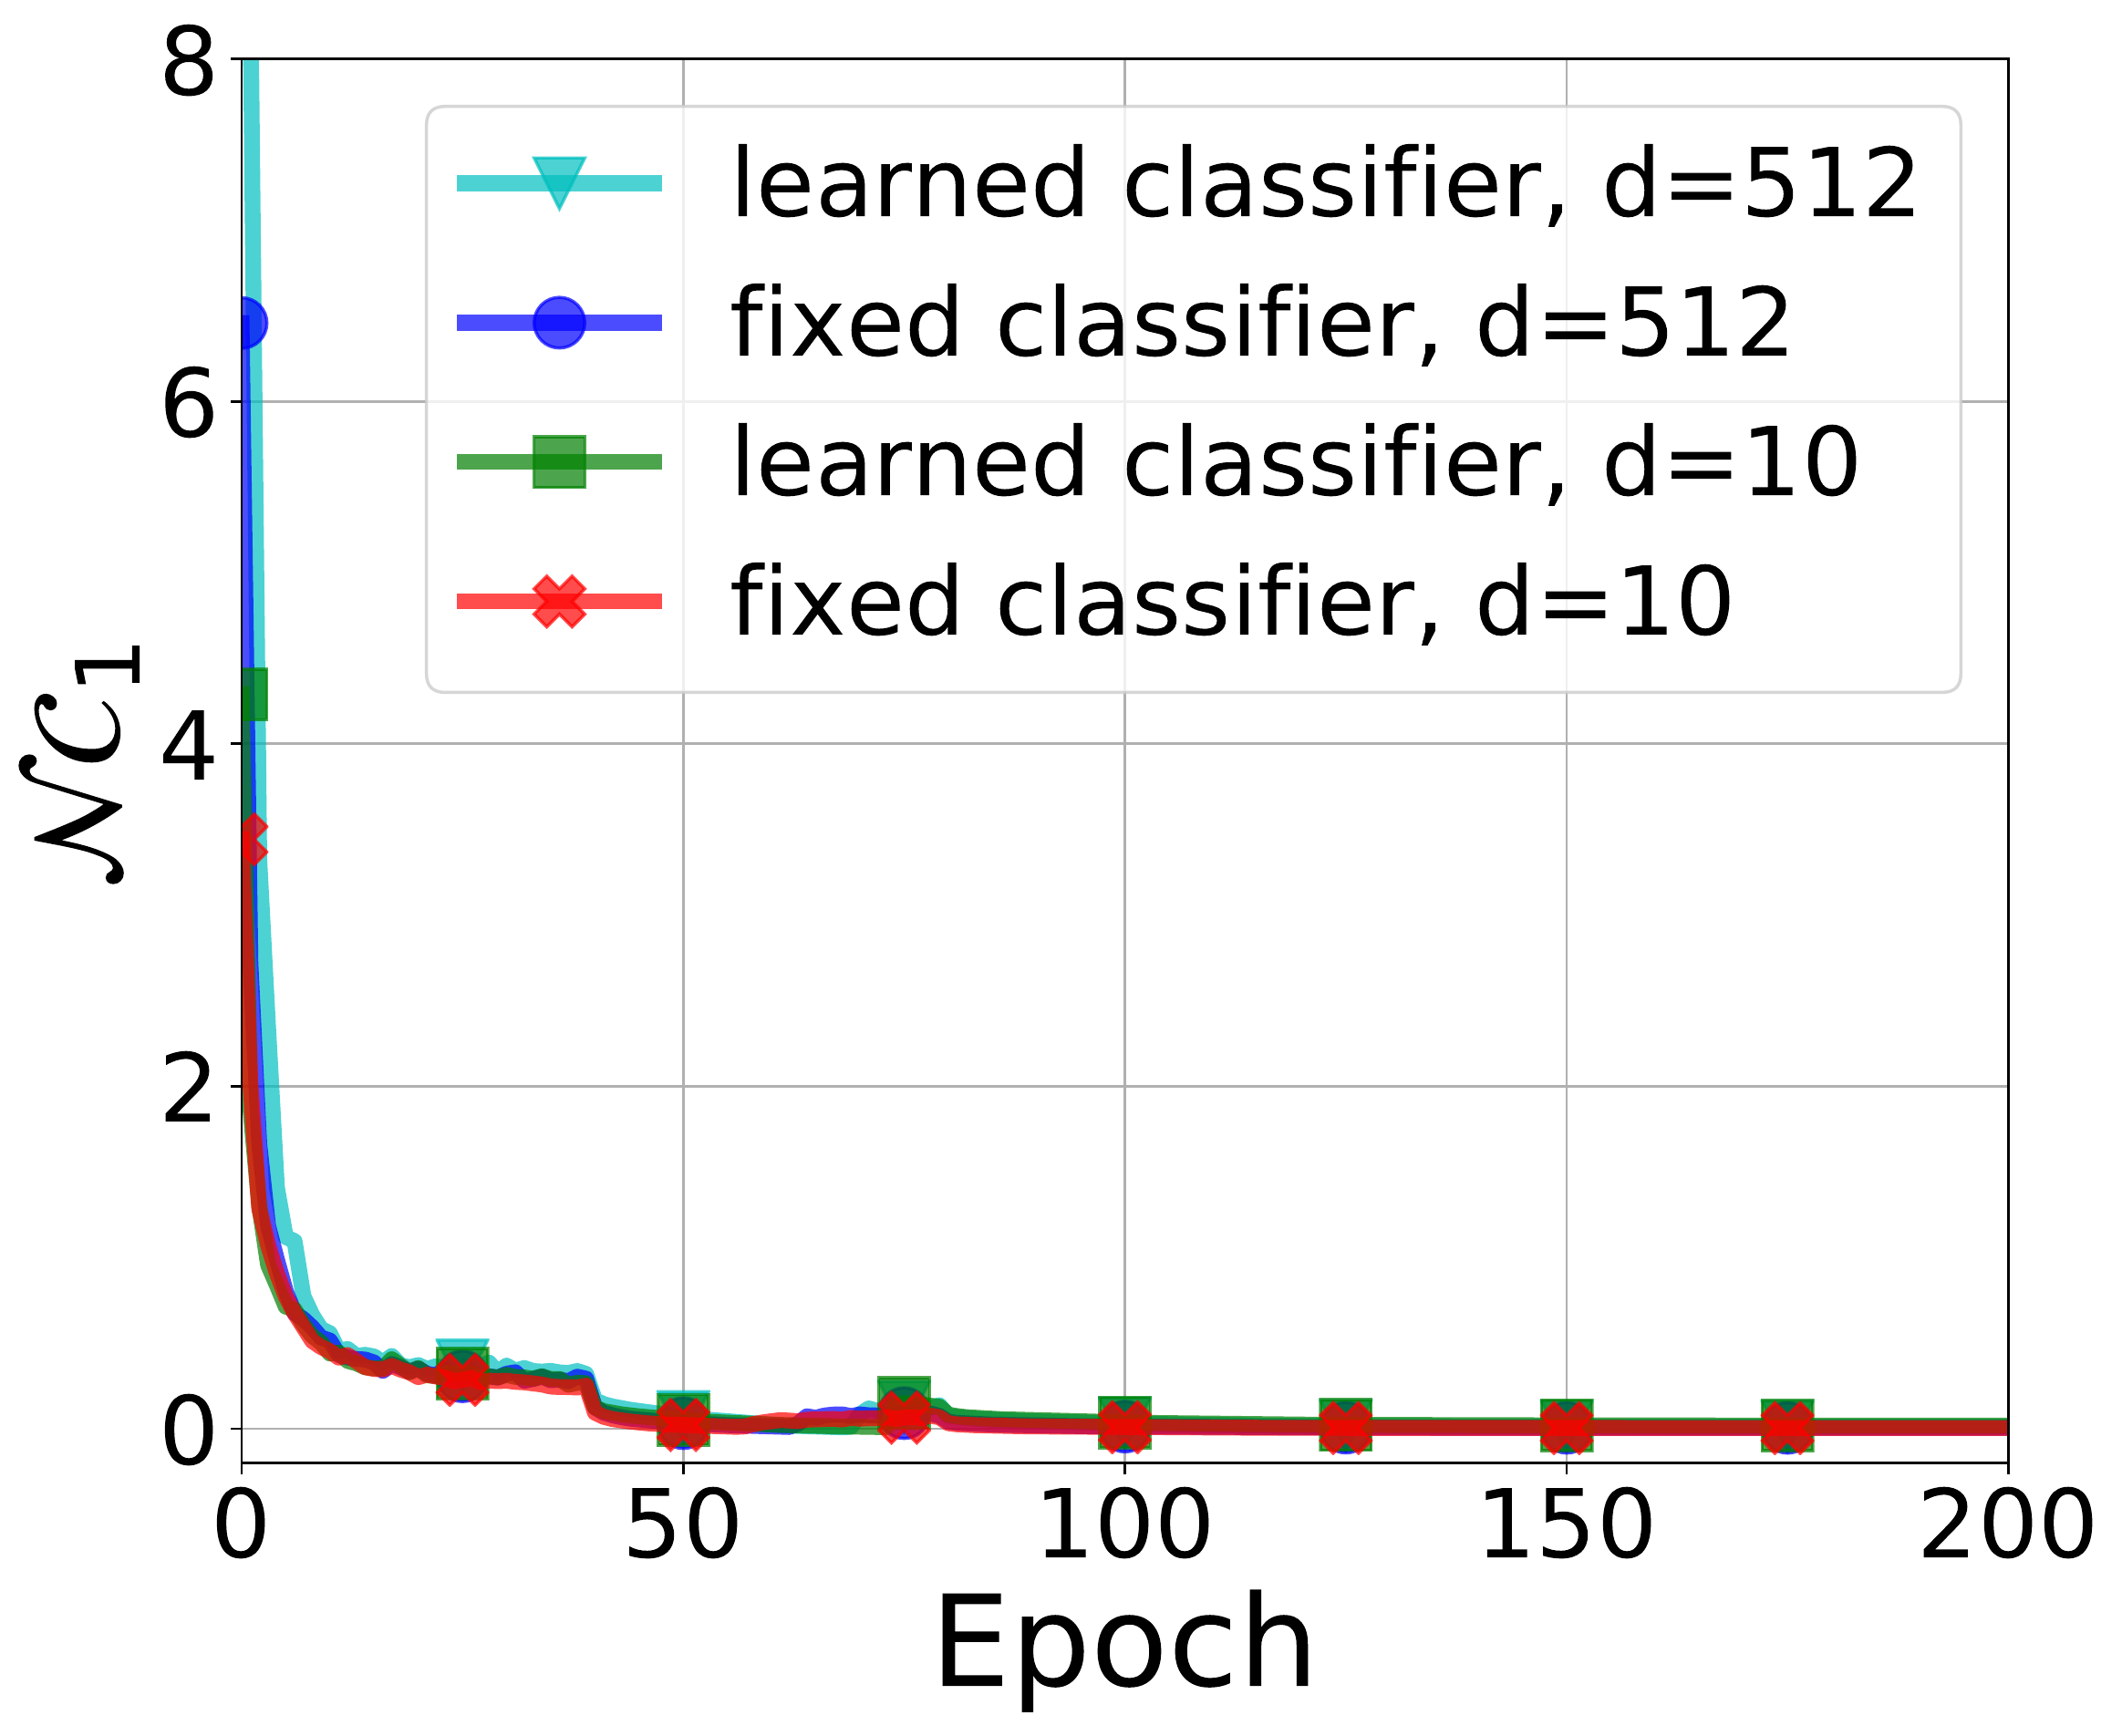} 
    % \subfloat[$\mc {NC}_2$ (MNIST)]{\includegraphics[width=0.32\textwidth]{figs/resnet18/mnist-SGD-ETF-fixdim/mnist-resnet18-NC2.pdf}} \
    \includegraphics[width=0.24\textwidth]{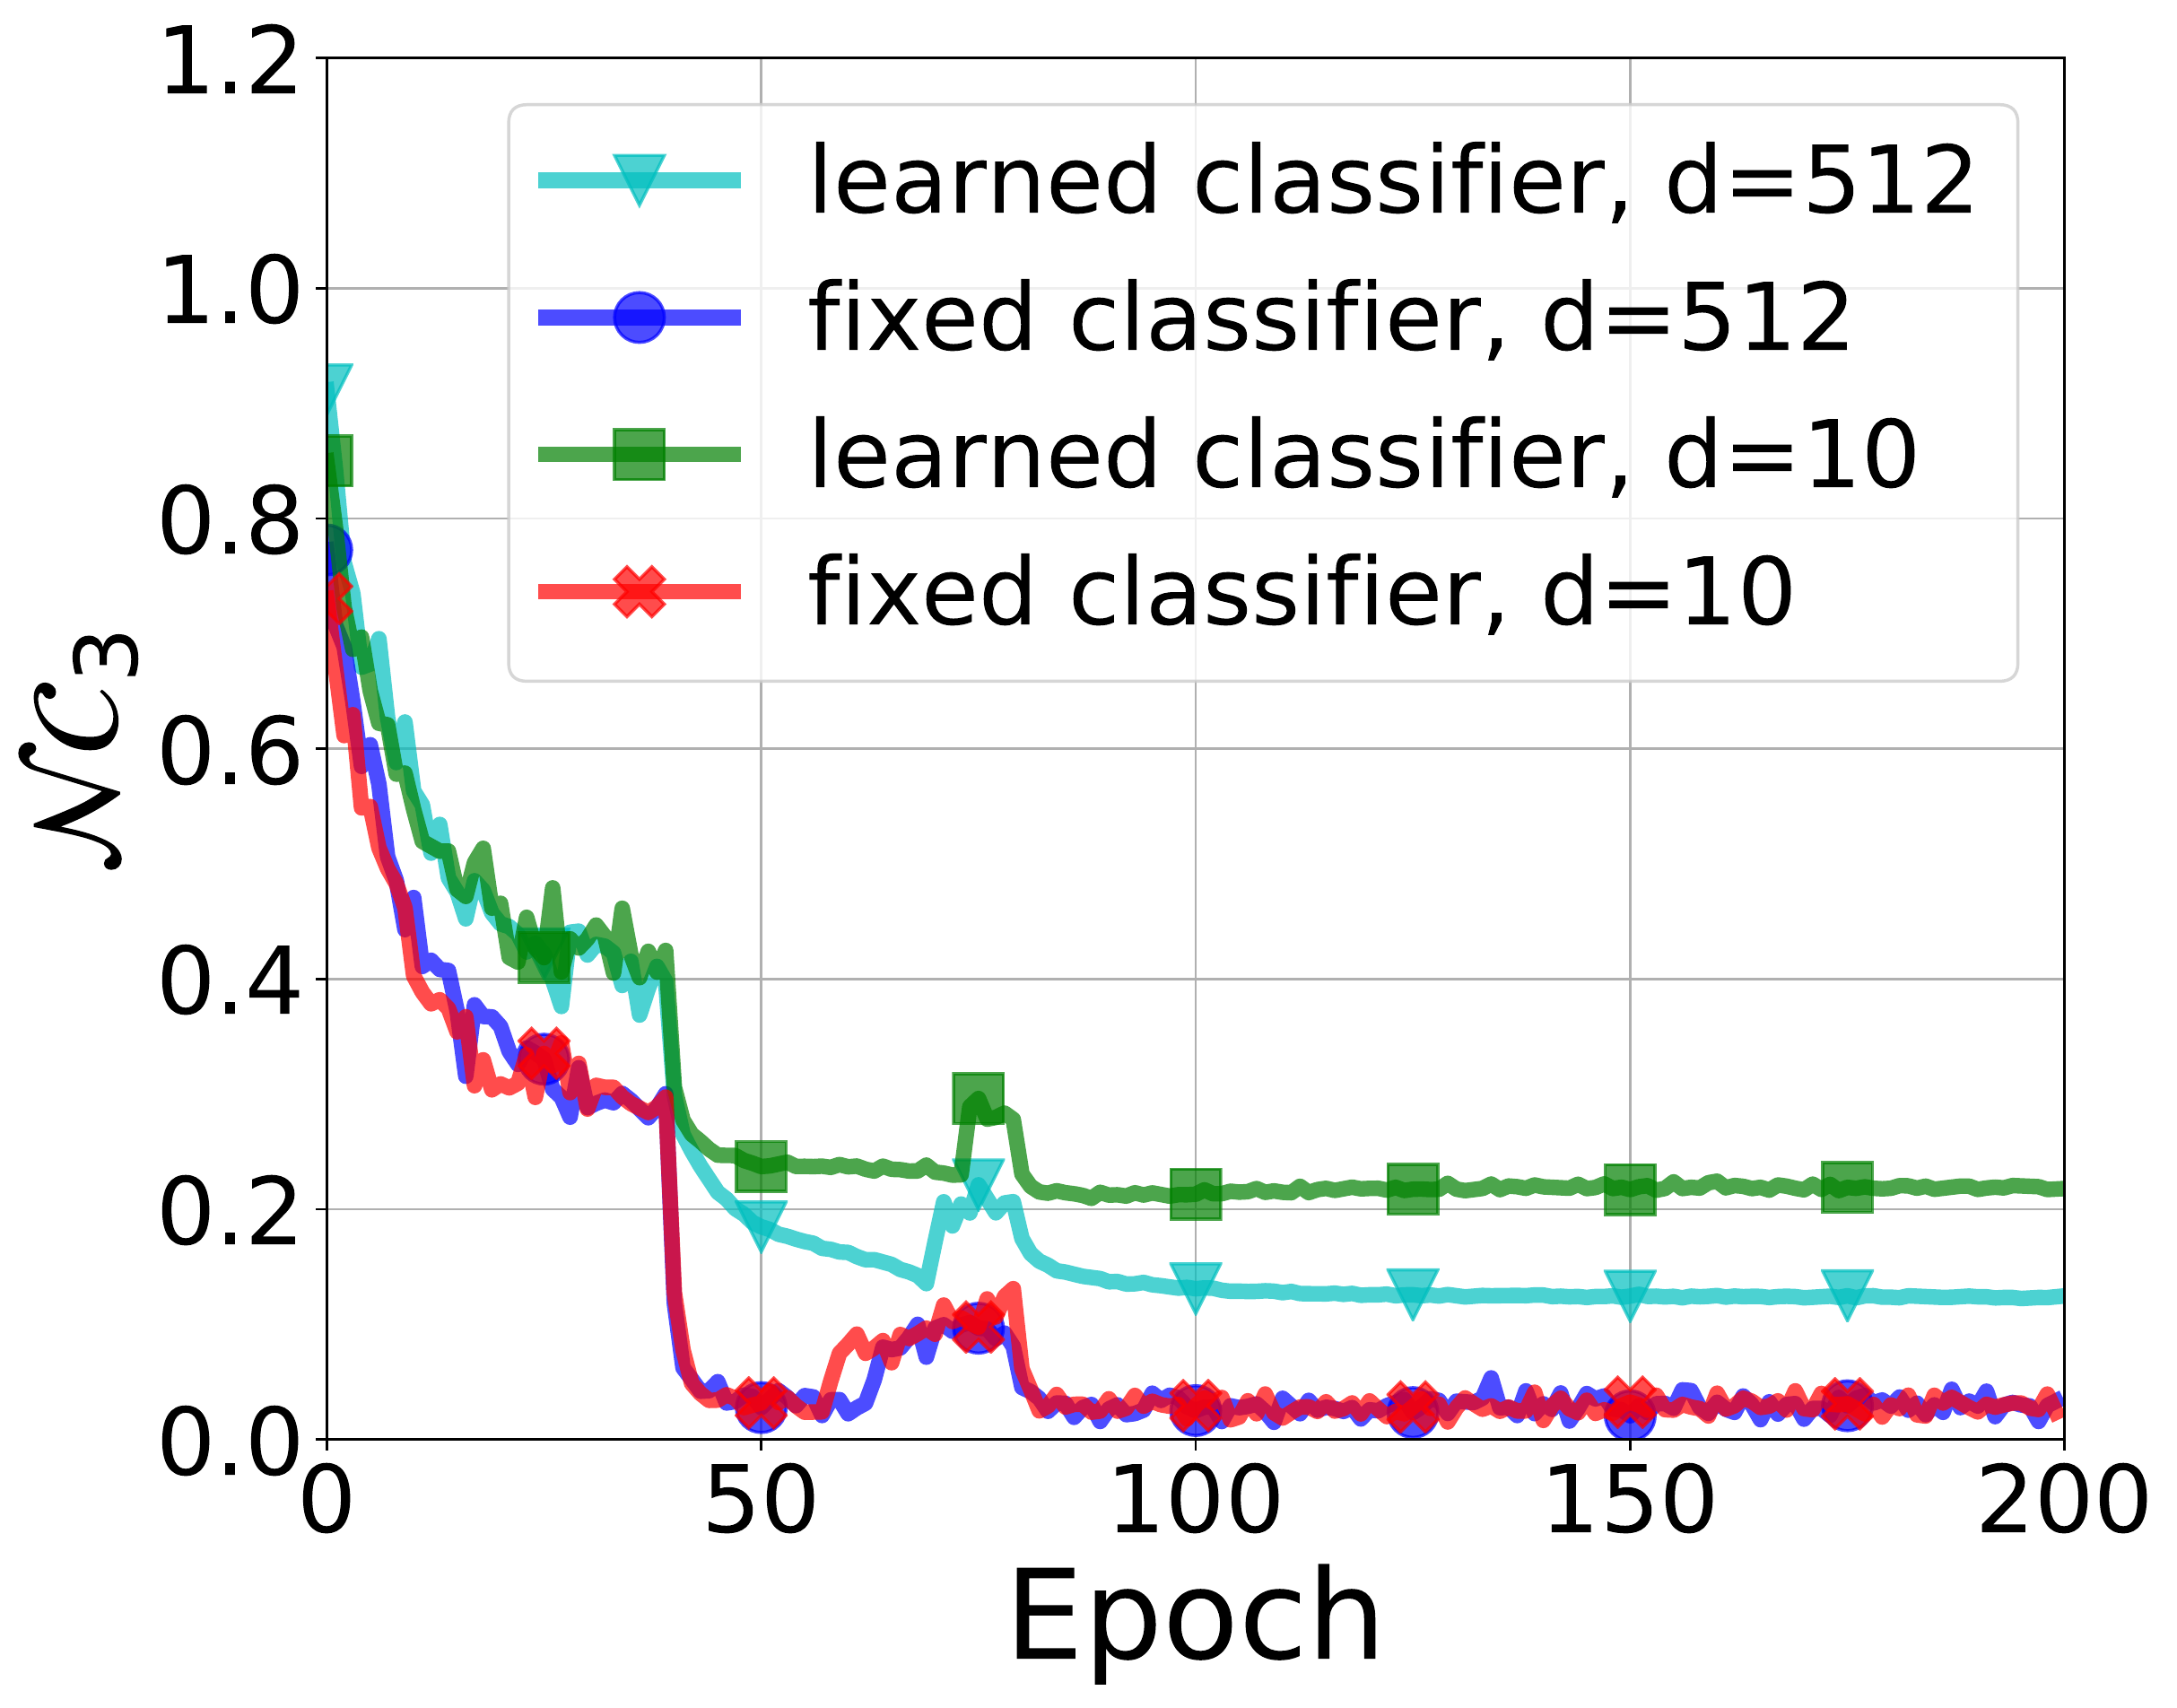} \
    % \subfloat[$\mc {NC}_4$ (MNIST)]{\includegraphics[width=0.32\textwidth]{figs/resnet18/cifar10-SGD-ETF-fixdim/cifar10-resnet18-NC4.pdf}} \
    \includegraphics[width=0.24\textwidth]{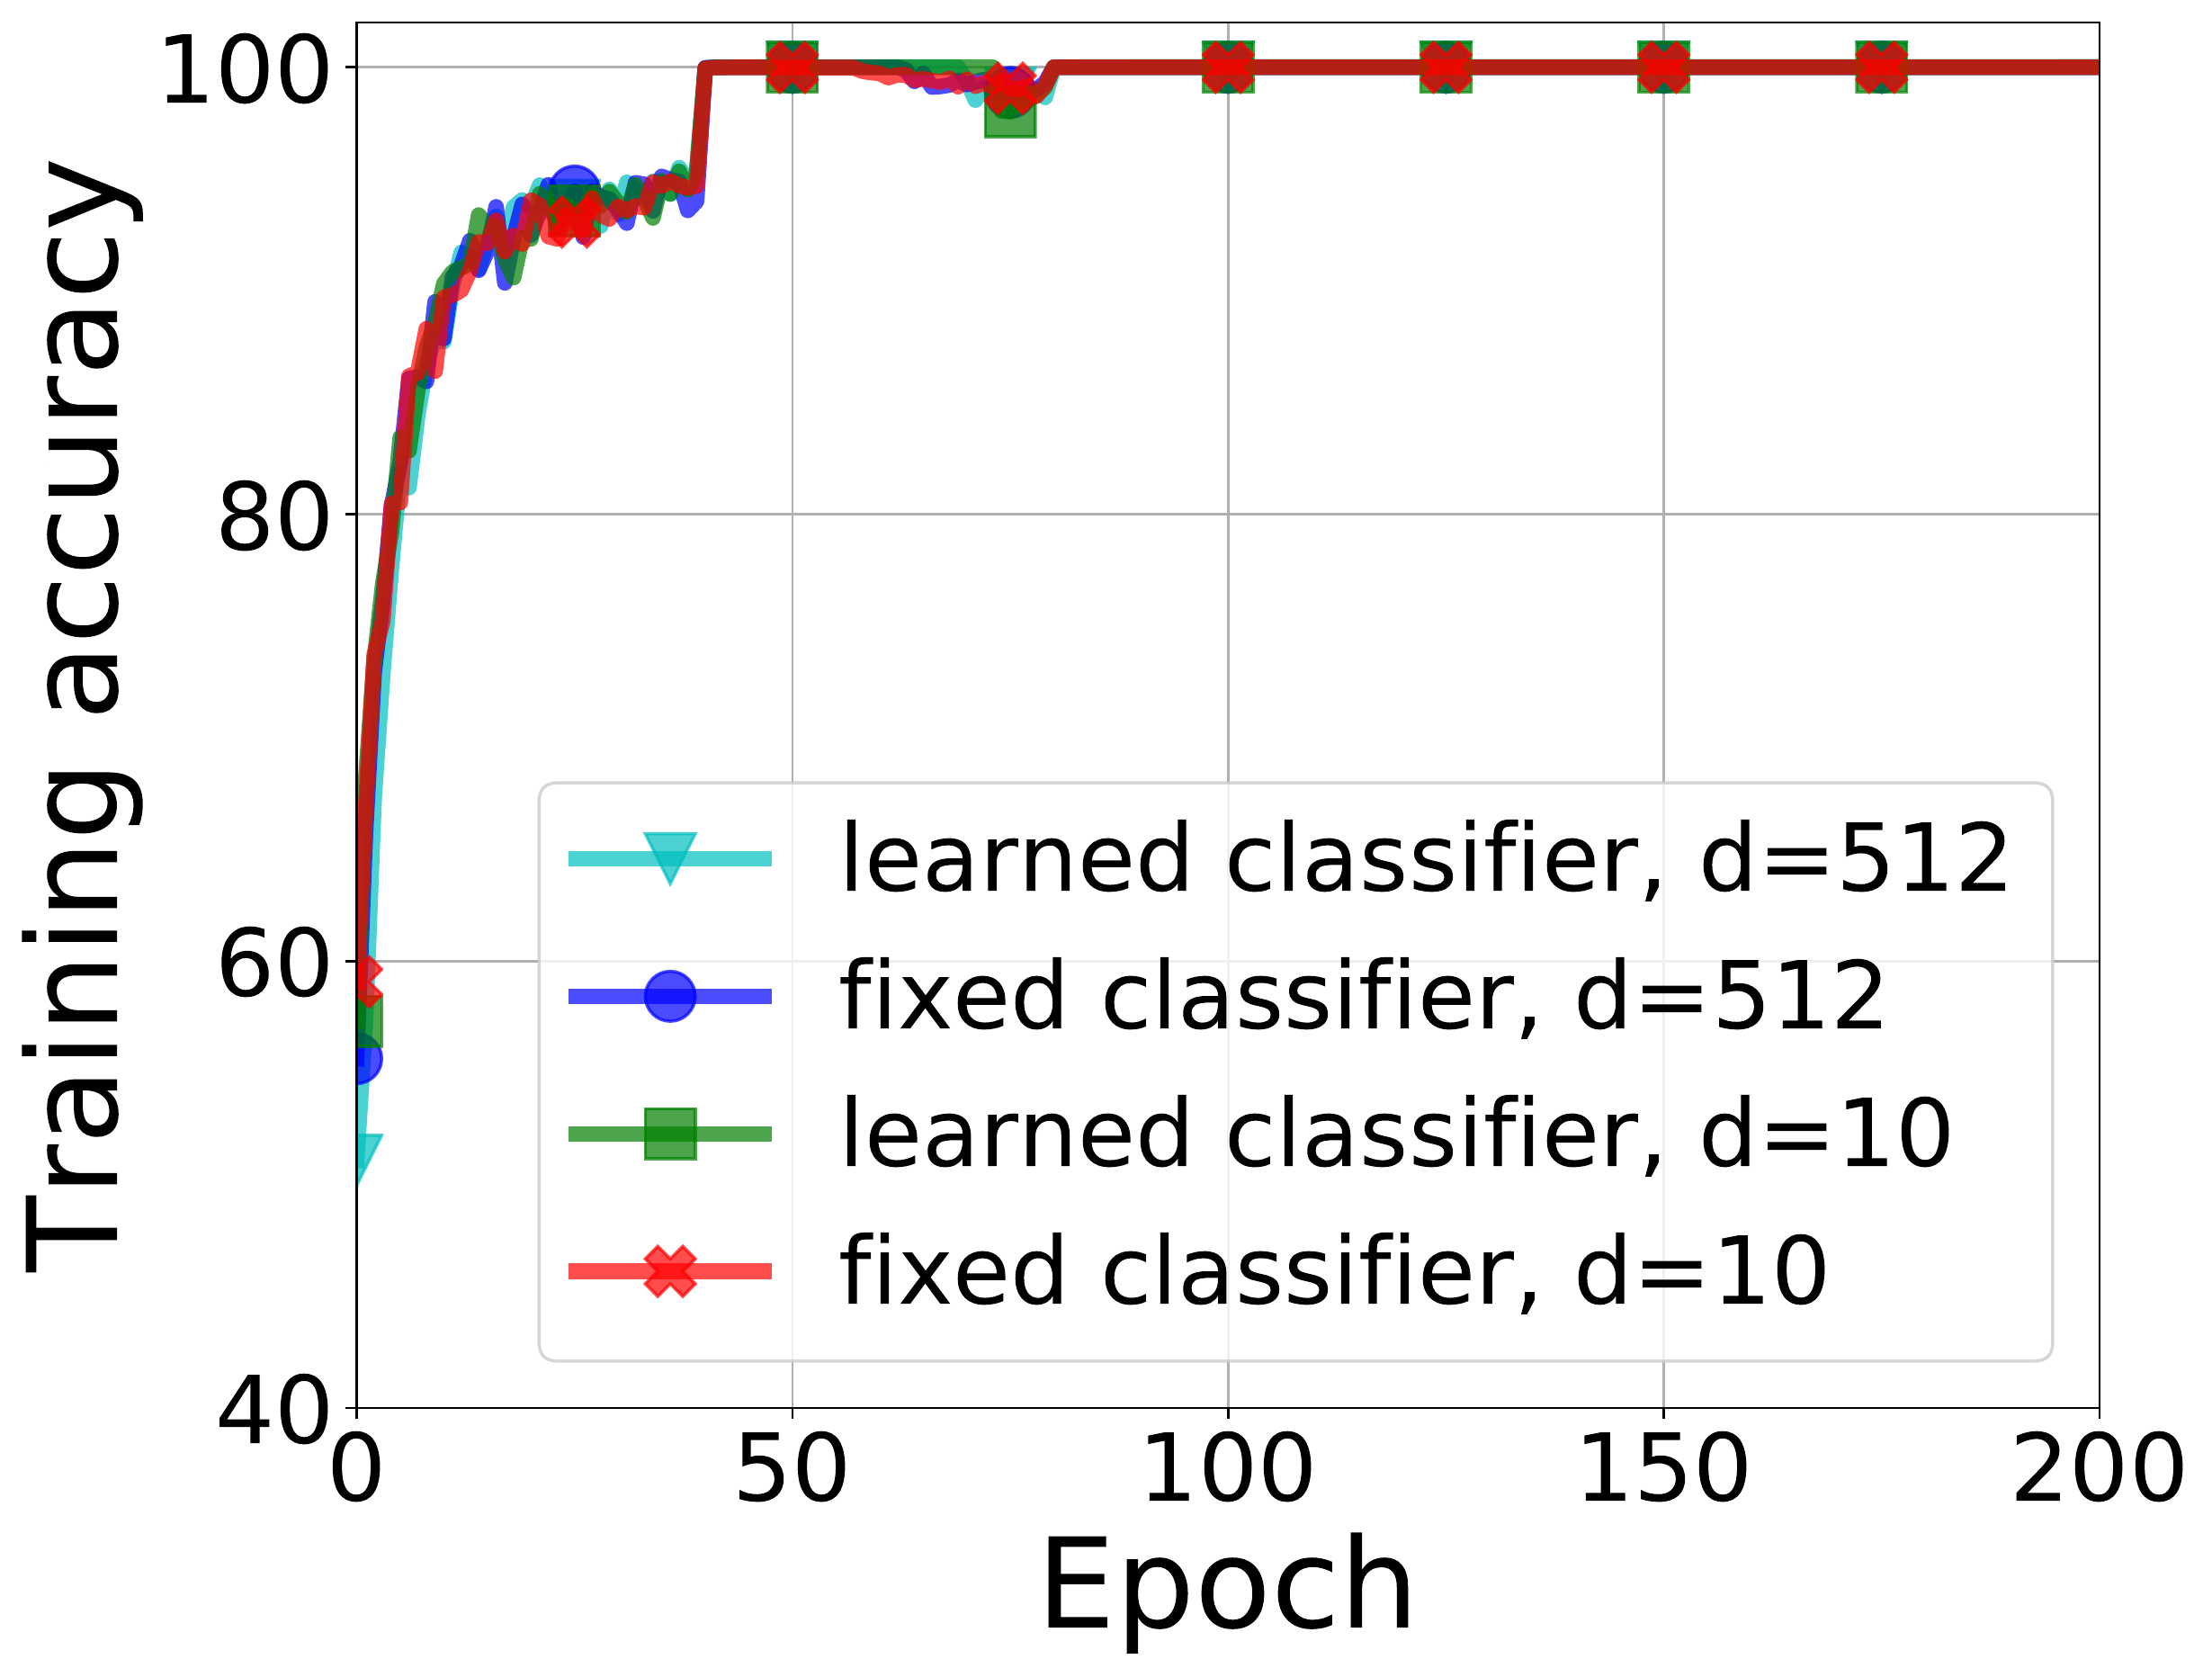} \
   \includegraphics[width=0.24\textwidth]{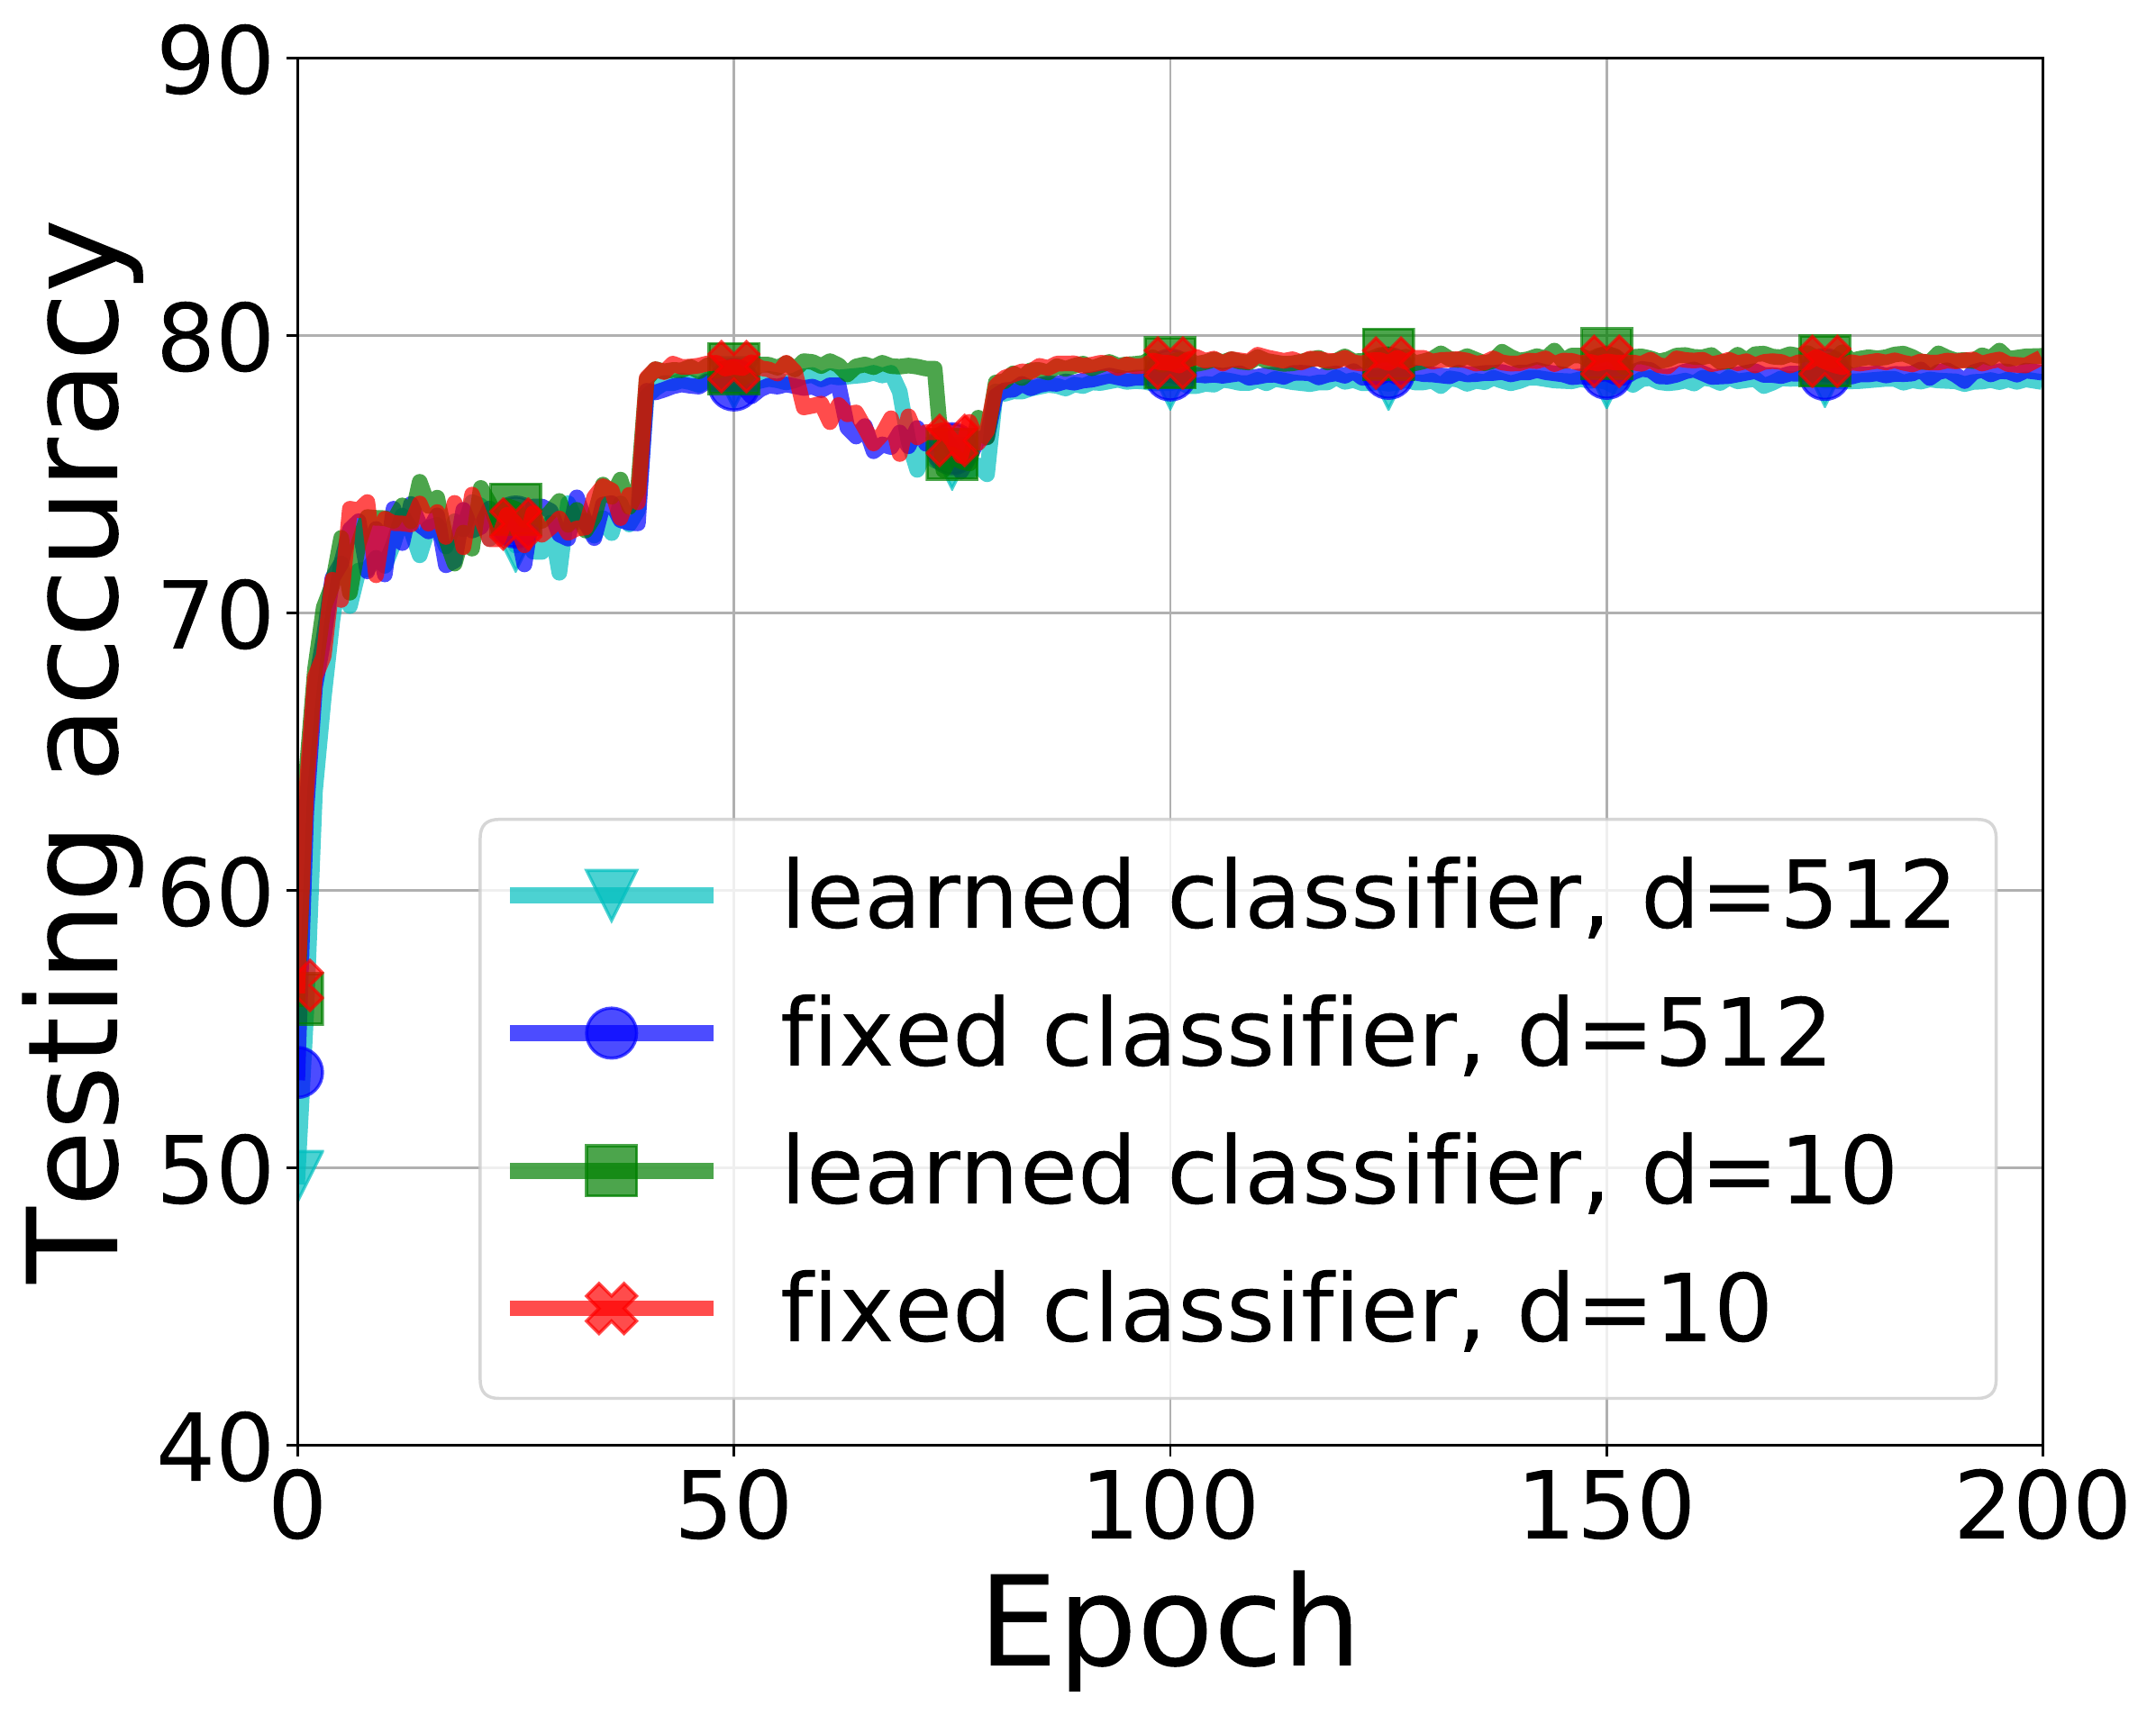}}
    \caption{\textbf{Comparison of the performances on learned vs. fixed last-layer classifiers.} We compare within-class variation collapse $\mc {NC}_1$, self-duality $\mc {NC}_3$, training accuracy, and test accuracy, on fixed and learned classifier on MNIST-ResNet18 (Top) and CIFAR10-ResNet18 (Middle). All networks are trained by SGD optimizer. 
    }
    \label{fig:fxied-classifier-appendix}
\end{figure}
