# Supplementary material for: Are All Losses Created Equal: A Neural Collapse Perspective
Source: arXiv:2210.02192 source file (2022-10-08)
Supplement: Supplementary file 10 [file prior.tex]

Our work highly relates to recent advances on studying the optimization landscape in neural network training; see \cite{sun2020optimization,sun2020global} for a contemporary survey. Most of the existing work \cite{haeffele2015global,baldi1989neural,kawaguchi2016deep,safran2018spurious,yun2018small,laurent2018deep,nouiehed2018learning,liang2018adding,zhu2019global,yun2018global,zhou2021local} analyzes the problem based on a \emph{bottom-up} approach -- from the input to the output of neural networks -- ranging from two-layer linear network \cite{baldi1989neural,nouiehed2018learning,kunin2019loss,zhu2019global}, deep linear network \cite{kawaguchi2016deep,nouiehed2018learning,yun2018global,laurent2018deep}, to nonlinear network \cite{safran2018spurious,nouiehed2018learning,yun2018small,liang2018adding}. More specifically, the line of work \cite{baldi1989neural,kawaguchi2016deep,nouiehed2018learning,zhu2019global,yun2018global} studied the optimization landscape for linear two-layer networks and proved that the associated training loss is a strict saddle function. For deeper linear networks, it can be shown that flat saddle points exist at the origin, but there are no spurious local minima \cite{kawaguchi2016deep,laurent2018deep}. For nonlinear neural networks, it has been proved that there do exist spurious local minima \cite{safran2018spurious,yun2018small}, but such local minima may be eliminated, or the number can be significantly reduced, in the over-parameterization regime \cite{safran2018spurious,liang2018adding}. Additionally, the work \cite{haeffele2015global} proved that certain local minima (having an all-zero ``slice'') are also global solutions, but the analysis is crucially dependent on the sufficient condition of an all-zero slice in the weights, which is insufficient to characterize the landscape properties. At a high level, the differences between these results and ours can be summarized as follows.
\begin{itemize}[leftmargin=*]
 %   \item \textbf{\emph{Optimization vs. Learning Perspectives.}} Most of these results based on the bottom-up approach only focus on the optimization perspective of deep learning, explaining why the training loss can be efficiently minimized to optimality. However, they provided limited insights into the empirical success of learning in terms of learned representations, generalization, and robustness. In contrast, we take a \emph{top-down} approach to look at the network starting from the very last layer. The slight difference in the models can lead to a dramatic difference in the interpretability for deep learning. As we will show in this work, by starting from the last layer, our results not only provide valid reasons on why the training loss can be efficiently optimized, but also provide new insights on the learning perspective through the last-layer classifiers and features learned from the network. \js{I'm not super sure about this point on ``optimization vs learning''. There are works that look at optimization and can show max-min solutions, which naturally lead to learning (generalization) guarantees (see eg [Wei, Lee, Liu \& Ma, 2018]).} \zz{Agree with JS. We need to be careful about ``learning". I thinking ``learning perspective" is mainly referred to generalization and other learning issues, but this paper focuses more on the optimization part. What this paragraph expresses is that here our optimization problem looks at the representation or feature, while most of the others look at the loss function.}\cy{Agreed \& how about the following:}

    \item \textbf{\emph{A Feature Learning Perspective.}} While most of these results based on the bottom-up approach explain optimization and generalization of certain types of deep neural networks, they provided limited insights into the practice of deep learning. In contrast, we take a \emph{top-down} approach to look at the network starting from the very last layer. The slight difference in the models can lead to a dramatic difference in the interpretability for deep learning. By starting from the last layer, our results not only provide valid reasons on why the training loss can be efficiently optimized, but also provide a precise characterization of the last-layer features as well as the classifiers learned from the network. As we will show, such a feature learning perspective not only helps with network design (see \Cref{sec:exp-fix-classifier}), but may bear broadly on generalization and robustness of deep learning as well as the recent development of contrastive learning (see \Cref{sec:conclusion}).% \cy{Best I can come up with to replace the previous one. Hopefully this is better}

    \item \textbf{\emph{Connections to Empirical Phenomena.}} Moreover, most existing theoretical results on landscape analysis \cite{allen2019convergence,du2019gradient} are somewhat disconnected from practice due to unrealistic assumptions, providing limited guiding principles for modern network training or design. In contrast, our assumption on the last-layer features as optimization variables is naturally based on model overparameterization. Moreover, our results provide explanations for \NC, an empirical phenomenon that has been widely observed on convincing numerical evidence across many different practical network architectures and a variety of standard image datasets.
\end{itemize}
%\qq{cite Sam's work and discuss relationship to NTK?}

Our work also broadly relates to the recent theoretical study for deep learning based on Neural Tangent Kernels (NTKs) \cite{jacot2018neural}, where a neural network behaves like a \emph{linear} model on random features hence has a benign optimization landscape. 
However, the ``kernel regime'' that NTKs work in requires neural networks that are infinitely wide -- or at least so wide that is beyond the regime that practical neural networks work in \cite{zou2020gradient,montanari2020interpolation,buchanan2020deep,chizat2019lazy}. 
% Consequently, there has been controversy on whether NTKs provides insights for understanding the practice of deep learning at all. 
In contrast, we adopt the unconstrained feature model which does not directly impose requirements on the width of the neural network and, as shown in our experiments, well captures the behavior of practical neural networks. 
Hence, our result can provide a more practical understanding for deep learning. 

Moreover, from a boarder perspective our work is rooted in recent advances on global nonconvex optimization theory for signal processing and machine learning problems \cite{chi2019nonconvex,danilova2020recent,zhang2020symmetry,qu2020finding,10.1145/3418526}. In a sequence of works \cite{zhao2015nonconvex,sun2016complete1,sun2015complete,li2016,qu2017convolutional,sun2018geometric,zhu2018global,li2019symmetry,zhu2018distributed,chi2019nonconvex,qu2020geometric,qu2020finding,qu2020exact,lau2020short,kuo2019geometry,zhang2019structured}, the authors showed that many problems exhibit ``equivalently good'' global minimizers due to symmetries and intrinsic low-dimensional structures, and the loss functions are usually strict saddles \cite{ge2015escaping,sun2015nonconvex,zhang2020symmetry}. These problems include, but are not limited to, phase retrieval \cite{sun2018geometric,qu2017convolutional}, low-rank matrix recovery \cite{zhao2015nonconvex,li2016,zhu2018global,chi2019nonconvex,zhu2018distributed}, dictionary learning \cite{qu2014finding,sun2016complete1,sun2015complete,qu2020geometric,qu2020finding}, and sparse blind deconvolution \cite{kuo2019geometry,qu2020exact,lau2020short,zhang2019structured}. As we shall see, the global minimizers (i.e., simplex ETFs) of our problem here also exhibit a similar rotational symmetry, compared to low-rank matrix recovery. In fact, our proof techniques are inspired by recent results on low-rank matrix recovery \cite{zhu2018global,chi2019nonconvex}. Thus, our work establishes a new connection between recent advances on nonconvex optimization theory and deep learning.
