# Supplementary material for: Are All Losses Created Equal: A Neural Collapse Perspective
Source: arXiv:2210.02192 source file (2022-10-08)
Supplement: Supplementary file 12 [file thm_landscape.tex]

In this part of appendices, we prove \Cref{thm:global-geometry} in \Cref{sec:main}. In particular, we analyze the global optimization landscape of 
\begin{align*}
     \min_{\mb W , \mb H,\mb b  } \;f(\mb W,\mb H,\mb b) \;=\;  \frac{1}{Kn} \sum_{k=1}^K \sum_{i=1}^{n} \Lce \paren{ \mb W \mb h_{k,i} + \mb b, \mb y_k } \;+\; \frac{\lambda_{\mb W} }{2} \norm{\mb W}{F}^2 + \frac{\lambda_{\mb H} }{2} \norm{\mb H}{F}^2 + \frac{\lambda_{\mb b} }{2} \norm{\mb b}{2}^2 ,
\end{align*}
with respect to $\mb W \in \bb R^{K \times d}$, $\mb H = \begin{bmatrix}\vh_{1,1} \cdots \vh_{K,n} \end{bmatrix} \in \bb R^{d \times N} $, and $\mb b \in \bb R^K$.
We show that the function is a strict saddle function \cite{ge2015escaping,sun2015nonconvex,zhang2020symmetry} in the Euclidean space, that there is no spurious local minimizer and all global minima are corresponding to the form showed in \Cref{thm:global-minima-app}.

\begin{theorem}[No Spurious Local Minima and Strict Saddle Property]\label{thm:global-geometry-app}
	Assume that the feature dimension $d$ is larger than the number of classes $K$, i.e., $d> K$. Then the function $f(\mb W,\mb H,\mb b)$ in \eqref{eq:obj-app} is a strict saddle function with no spurious local minimum:
	\begin{itemize}
	    \item Any local minimizer of \eqref{eq:obj-app} is a global minimum of the form shown in \Cref{thm:global-minima-app}.
	    \item Any critical point of \eqref{eq:obj-app} that is not a local minimum has at least one negative curvature direction, i.e., the Hessian $\nabla^2 f(\mb W,\mb H,\mb b)$ at this point has at least one negative eigenvalue 
	    \begin{align*}
	        \lambda_i\paren{\nabla^2 f(\mb W,\mb H,\mb b)}\;<\;0.
	    \end{align*}
	\end{itemize}
\end{theorem}

\subsection{Main Proof}

\begin{proof}[Proof of \Cref{thm:global-geometry-app}]
The main idea of proving \Cref{thm:global-geometry} is to first connect the problem \eqref{eq:obj-app} to its corresponding convex counterpart,
so that we can obtain the global optimality conditions for the original problem \eqref{eq:obj-app} based on the convex counterpart. Finally, we characterize the properties of all the critical points based on the optimality condition. We describe this in more detail as follows.

\paragraph{Connection of \eqref{eq:obj-app} to a Convex Program.} Let $\mb Z = \mb H \mb W \in \bb R^{K \times N}$ with $N=nK$ and $\alpha = \frac{\lambda_{\mH}}{\lambda_{\mW}}$. By Lemma \ref{lem:nuclear-norm}, we know that
\begin{align*}
   \min_{\mb H\mb W = \mb Z} \; \frac{ \lambda_{\mb W} }{2} \norm{\mb W}{F}^2 + \frac{ \lambda_{\mb H} }{2} \norm{\mb H}{F}^2 \;&=\; \sqrt{\lambda_{\mb W} \lambda_{\mb H} }  \min_{\mb H\mb W = \mb Z}  \;\frac{1}{2\sqrt{\alpha} } \paren{ \norm{\mb W}{F}^2 + \alpha \norm{\mb H}{F}^2 } \\
   \;&=\; \sqrt{\lambda_{\mb W} \lambda_{\mb H} }  \norm{\mb Z}{*}.
\end{align*}
Thus, we can relate the bilinear factorized problem \eqref{eq:obj-app} to a convex problem in terms of $\mb Z$ and $\mb b$ as follows
\begin{align}\label{eq:convex-prob}
    \min_{\mb Z \in \bb R^{K \times N},\; \mb b \in \bb R^{K}}\; \wt{f}(\mb Z,\mb b) \;:=\; g\paren{\mb Z + \mb b \mb 1^\top} +  \sqrt{\lambda_{\mb W} \lambda_{\mb H} }  \norm{\mb Z}{*} + \frac{\lambda_{\mb b}}{2} \norm{\mb b}{2}^2.
\end{align}
Similar to the idea in \cite{haeffele2015global,ciliberto2017reexamining,zhu2018global,li2019non}, we will characeterize the critical points of \eqref{eq:obj-app} by establishing a connection to the optimality condition of the convex problem \eqref{eq:convex-prob}. Towards this goal, we first show the global minimum of the convex program \eqref{eq:convex-prob} provides a lower bound for the original problem \eqref{eq:obj}. More specifically, in Lemma \ref{lem:equivalence} we can show that for any global minimizer $(\mb Z_\star, \mb b_\star)$ of $\wt{f}$ satisfies 
\begin{align}\label{eqn:convex-lower-bound}
    \wt{f}(\mZ^\star,\vb^\star) \;\leq\; f(\mW,\mH,\vb),\quad \forall \; \mW\in\R^{K\times d},\;\mH\in\R^{d\times N},\;\vb\in\R^K.
\end{align}

\paragraph{Characterizing the Optimality Condition of \eqref{eq:obj-app} Based on the Convex Program \eqref{eq:convex-prob}.}
Next, we characterize the optimality condition of our nonconvex problem \eqref{eq:obj-app}, based on the relationship to its convex counterpart
\eqref{eq:convex-prob}. Specifically, Lemma \ref{lem:conv-global-cond} showed that any critical point $(\mZ,\vb)$ of \eqref{eq:convex-prob} is characterized by the following necessary and sufficient condition
\e\begin{split}
    &\nabla g(\mZ + \vb\vone^\top) \;\in\; - \sqrt{\lambdaW\lambdaH}\partial\norm{ \mZ}{*},\\
    &\sum_{i=1}^N [\nabla g(\mZ + \vb\vone^\top)]_i + \lambdab\vb\; =\; \vzero,
\end{split}
\label{eq:KKT-convex-app}\ee
where $[\nabla g(\mZ + \vb\vone^\top)]_i$ represents the $i$-th column in $\nabla g(\mZ + \vb\vone^\top)$. By Lemma \ref{lem:global-optimality-nonconvex}, we can transfer the optimality condition from convex to the nonconvex problem \eqref{eq:obj-app}. More specifically, any critical point $(\mW,\mH,\vb)$ of \eqref{eq:obj-app} satisfies
\begin{align*} 
    \norm{ \nabla g(\mb W \mb H + \mb b \mb 1^\top) }{} \;\leq \; \sqrt{ \lambda_{\mb W} \lambda_{\mb H} },
\end{align*}
then $(\mb Z,\mb b)$ with $\mb Z = \mb W\mb H$ satisfies all the conditions in \eqref{eq:KKT-convex-app}. Combining with \eqref{eqn:convex-lower-bound}, Lemma \ref{lem:global-optimality-nonconvex} showed that $(\mW,\mH,\vb)$ is a global solution of the nonconvex problem \eqref{eq:obj-app}.

\paragraph{Proving No Spurious Local Minima and Strict Saddle Property.} Now we turn to prove the strict saddle property and that there are no spurious local minima by characterizing the properties for all the critical points of \eqref{eq:obj-app}. Denote the set of critical points of $f(\mW,\mH,\vb)$ by
\begin{align*}
    \calC \;:=\; \Brac{ \; \mW\in\R^{K\times d},\mH\in\R^{d\times N}, \vb\in\R^K \;\mid\;  \nabla f(\mW,\mH,\vb) \;=\; \vzero\; }.
\end{align*}
To proceed, we separate the set $\calC$ into two disjoint subsets
\begin{align*}
    \calC_1 \;&:=\;  \calC\cap \Brac{\; \mW\in\R^{K\times d},\mH\in\R^{d\times N}, \vb\in\R^K\;\mid\; \norm{\nabla g(\mW\mH + \vb\vone^\top)}{} \;\leq\; \sqrt{\lambdaW\lambdaH} \;} ,\\
       \calC_2 \;&:=\; \calC\cap \Brac{\; \mW\in\R^{K\times d},\mH\in\R^{d\times N}, \vb\in\R^K\;\mid\; \norm{\nabla g(\mW\mH + \vb\vone^\top)}{}  \;>\; \sqrt{\lambdaW\lambdaH} \;},
\end{align*}
satisfying $\calC = \calC_1\cup\calC_2$. By Lemma \ref{lem:global-optimality-nonconvex}, we already know that any $(\mW,\mH,\vb)\in \calC_1$ is a global optimal solution of $f(\mb W,\mb H,\mb b)$ in \eqref{eq:obj-app}. If we can show that any critical point in $\calC_2$ possesses negative curvatures (i.e., the Hessian at $(\mb W,\mb H,\mb b)$ has at least one negative eigenvalue), then we prove that there is no spurious local minima as well as strict saddle property.

%If we show that $\calC_2$ is the set of strict saddles, then we prove that there is no spurious local minima as well as strict saddle property. By Lemma \ref{lem:global-optimality-nonconvex}, we conclude that $(\mW,\mH,\vb)$ is the globally optimal solution of \eqref{eq:obj} for any $(\mW,\mH,\vb)\in \calC_1$. If we show that $\calC_2$ is the set of strict saddles, then we prove that there is no spurious local minima as well as strict saddle property. 
Thus, the remaining part is to show any point in $\calC_2$ possesses negative curvatures. We will find a direction $\mDelta$ along which the Hessian has a strictly negative curvature for this point. Towards that goal, for any $\mDelta = (\mDelta_{\mW},\mDelta_{\mH},\mDelta_{\vb})$, we first compute the Hessian bilinear form of $f(\mb W,\mb H,\mb b)$ along the direction $\mDelta$ by
\begin{align}\label{eqn:hessian-f}
\begin{split}
        &\nabla^2 f(\mW,\mH,\vb)[\mDelta,\mDelta] \\
    \;=\;& \nabla^2g(\mW\mH + \vb\vone^\top) \brac{  \mW\mDelta_{\mH} + \mDelta_{\mW}\mH + \mDelta_{\vb}\vone^\top,\mW\mDelta_{\mH} + \mDelta_{\mW}\mH + \mDelta_{\vb}\vone^\top } \\
    &+ 2\innerprod{\nabla g(\mW\mH+ \vb\vone^\top)}{\mDelta_{\mW}\mDelta_{\mH}} +\lambdaW\norm{\mDelta_{\mW}}{F}^2 + \lambdaH \norm{\mDelta_{\mH}}{F}^2 + \lambdab\norm{\mDelta_{\vb}}{2}^2.
\end{split}
\end{align}
We now utilize the property that $\norm{ \nabla g(\mW\mH + \vb\vone^\top)}{} > \sqrt{\lambdaW\lambdaH}$ for any $(\mW,\mH,\vb)\in \calC_2$ to construct a negative curvature direction. Let $\mb u$ and $\mb v$ be the left and right singular vectors corresponding to the largest singular value $\sigma_1(\nabla^2 g(\mW\mH + \vb\vone^\top))$ of $\nabla^2 g(\mW\mH + \vb\vone^\top)$, which is larger than $\sqrt{\lambdaW\lambdaH}$ by our assumption.

Since $d>K$ and $\mW \in \bb R^{K \times d}$, there exists a nonzero $\va\in\R^{d}$ in the null space of $\mW$, i.e., $\mW\va = \vzero$.
%$\mathrm{row}(\mW)= \mathrm{span}\Brac{\mb w_1, \cdots, \mb w_K}$, i.e., $\mW\va = \vzero$. 
%\zz{I think it is more common to simply say the null space of the matrix $\mW$. Not common to say the null space of a subspace.} 
Furthermore, by Lemma  \ref{lem:critical-balance}, we know that 
\begin{align*}
    \mW^\top\mW = \sqrt{ \frac{ \lambda_{\mb H} }{ \lambda_{\mb W} }  } \mH\mH^\top \quad \Longrightarrow\quad \mH^\top\va = \vzero.
\end{align*}
We now construct the negative curvature direction as 
 \begin{align*}
   \mb \Delta \;=\;  \paren{ \mb \Delta_{\mb W},\mDelta_{\mH}, \mDelta_{\vb}  } \;=\; \paren{  \paren{ \frac{ \lambda_{\mb H} }{ \lambda_{\mb W} } }^{1/4} \mb u \mb a^\top ,  - \paren{ \frac{ \lambda_{\mb H} }{ \lambda_{\mb W} } }^{-1/4} \mb a \mb v^\top, \mb 0 }
 \end{align*}
so that the term $\innerprod{\nabla g(\mW\mH+ \vb\vone^\top)}{\mDelta_{\mW}\mDelta_{\mH}}$ is small enough to create a negative curvature. Since $\mW\va = \vzero$, $\va^\top \mH = \vzero$, and $\mDelta_{\vb} = \mb 0$, we have
\begin{align*}
    \mW\mDelta_{\mH} + \mDelta_{\mW}\mH + \mDelta_{\vb}\vone^\top \;=\; - \paren{ \frac{ \lambda_{\mb H} }{ \lambda_{\mb W} } }^{-1/4}  \mW  \va \mb v^\top +  \paren{ \frac{ \lambda_{\mb H} }{ \lambda_{\mb W} } }^{1/4} \mb u \mb a^\top \mH \;=\; \vzero,
\end{align*}
so that $\nabla^2g(\mW\mH + \vb\vone^\top) \brac{  \mW\mDelta_{\mH} + \mDelta_{\mW}\mH + \mDelta_{\vb}\vone^\top,\mW\mDelta_{\mH} + \mDelta_{\mW}\mH + \mDelta_{\vb}\vone^\top } = 0$. Thus, combining the results above with \eqref{eqn:hessian-f}, we obtain the following
\begin{align*}
&\nabla^2 f(\mW,\mH,\vb)[\mDelta,\mDelta] \\
\;=\;& 2\innerprod{\nabla g(\mW\mH + \vb\vone^\top)}{\mDelta_{\mW}\mDelta_{\mH}} \;+\; \lambdaW\norm{\mDelta_{\mW}}{F}^2 + \lambdaH\norm{\mDelta_{\mH}}{F}^2 \\
\;=\;& -2\norm{\va}{2}^2\innerprod{\nabla g(\mW\mH + \vb\vone^\top)}{\mb u \mb v^\top} + 2 \sqrt{ \lambda_{\mb W} \lambda_{\mb H} }  \norm{\va}{2}^2 \\
\;=\;& -2\norm{\va}{2}^2 \paren{\norm{\nabla g(\mW\mH+ \vb\vone^\top)}{} - \sqrt{\lambdaW\lambdaH}} \;<\;0,
\end{align*}
where the last inequality is based on the fact that $(\mb W,\mb H,\mb b) \in \mc C_2 $ so that $\norm{ \nabla g(\mW\mH + \vb\vone^\top) }{} > \sqrt{\lambdaW\lambdaH}$. Therefore, any $(\mW,\mH,\vb)\in \calC_2$ possesses at least one negative curvature direction. This completes our proof of \Cref{thm:global-geometry-app}.
\end{proof}

\subsection{Supporting Lemmas}

\begin{lemma} \label{lem:equivalence}
If $(\mZ^\star,\vb^\star)$ is a global minimizer of
\begin{align*} 
    \min_{\mb Z \in \bb R^{K \times N},\; \mb b \in \bb R^{K}}\; \wt{f}(\mb Z,\mb b) \;:=\; g\paren{\mb Z + \mb b \mb 1^\top} +  \sqrt{\lambda_{\mb W} \lambda_{\mb H} }  \norm{\mb Z}{*} + \frac{\lambda_{\mb b}}{2} \norm{\mb b}{2}^2.
\end{align*}
introduced in \eqref{eq:convex-prob}, then $\wt{f}(\mZ^\star,\vb^\star) \le f(\mW,\mH,\vb)$ for all $\mW\in\R^{K\times d},\mH\in\R^{d\times N}, \vb\in\R^K$.
\end{lemma}

\begin{proof}[Proof of Lemma \ref{lem:equivalence}] Suppose $(\mZ^\star,\vb^\star)$ is a global minimum of $\wt{f}(\mb Z,\mb b)$. Then by \Cref{lem:nuclear-norm}, we have %\xiao{mark}
\begin{align*}
    \wt{f}(\mZ^\star,\vb^\star) \;&= \; \min_{\mZ,\vb} \; g(\mZ + \vb\vone^\top) + \sqrt{\lambdaW\lambdaH} \norm{\mZ}{*} + \frac{\lambda_{\mb b} }{2}\norm{\vb}{2}^2\\
    \;&= \; \min_{\mZ,\vb} \; g(\mb Z + \vb\vone^\top)+ \min_{\mW\mH=\mZ}  \paren{ \frac{\lambdaW}{2}\norm{\mW}{F}^2 + \frac{\lambdaH}{2}\norm{\mH}{F}^2 } + \frac{\lambdab}{2}\norm{\vb}{2}^2 \\
    \;&\leq\;\min_{\mb W,\mb H, \mb Z,\vb, \mb Z = \mb W\mb H} \; g(\mb W \mb H + \vb\vone^\top)+  \frac{\lambdaW}{2}\norm{\mW}{F}^2 + \frac{\lambdaH}{2}\norm{\mH}{F}^2  + \frac{\lambdab}{2}\norm{\vb}{2}^2.
\end{align*}
Thus, we have 
\begin{align*}
    \wt{f}(\mZ^\star,\vb^\star)  \;\leq\; \min_{\mW\in\R^{K\times d},\mH\in\R^{d\times N}, \vb\in\R^K} \; f(\mW,\mH,\vb)
\end{align*}
as desired.
\end{proof}

\begin{lemma}[Optimality Condition for the Convex Program \eqref{eq:convex-prob}]\label{lem:conv-global-cond}
Consider the following convex program in \eqref{eq:convex-prob} that we rewrite as follows
\begin{align*} 
    \min_{\mb Z \in \bb R^{K \times N},\; \mb b \in \bb R^{K}}\; \wt{f}(\mb Z,\mb b) \;:=\; g\paren{\mb Z + \mb b \mb 1^\top} +  \sqrt{\lambda_{\mb W} \lambda_{\mb H} }  \norm{\mb Z}{*} + \frac{\lambda_{\mb b}}{2} \norm{\mb b}{2}^2.
\end{align*}
Then the necessary and sufficient condition for $(\mb Z,\mb b)$ being the global solution of \eqref{eq:convex-prob} is 
\e\begin{split}
    &\nabla g(\mZ + \vb\vone^\top)\mV \;=\; - \sqrt{\lambdaW\lambdaH} \mU,\quad \nabla g(\mZ + \vb\vone^\top)^\top\mU \;=\; - \sqrt{\lambdaW\lambdaH} \mV,\\
     & \norm{\nabla g(\mZ + \vb\vone^\top)}{} \;\leq\;  \sqrt{\lambdaW\lambdaH}, \quad \text{and}\quad \sum_{i=1}^N [\nabla g(\mZ + \vb\vone^\top)]_i + \lambdab\vb\; =\; \vzero,
\end{split}
\label{eq:KKT-convex-equivalence}\ee
where $\mb U$ and $\mb V$ are the left and right singular value matrices of $\mb Z$, i.e., $\mb Z = \mb U \mb \Sigma \mb V^\top$.
\end{lemma}

\begin{proof}[Proof of Lemma \ref{lem:conv-global-cond}] 
Standard convex optimization theory asserts that any critical point $(\mZ,\vb)$ of \eqref{eq:convex-prob} is global, where the optimality is characterized by the following necessary and sufficient condition
\e\begin{split}
    &\nabla g(\mZ + \vb\vone^\top) \;\in\; - \sqrt{\lambdaW\lambdaH}\partial\norm{ \mZ}{*},\\
    &\sum_{i=1}^N [\nabla g(\mZ + \vb\vone^\top)]_i + \lambdab\vb\; =\; \vzero,
\end{split}
\label{eq:KKT-convex}\ee
where $[\nabla g(\mZ + \vb\vone^\top)]_i$ represents the $i$-th column in $\nabla g(\mZ + \vb\vone^\top)$, and $\partial\norm{\mZ}{*}$ denotes the subdifferential of the convex nuclear norm $\norm{\mZ}{*}$ evaluated at $\mZ$. By its definition, we have
\begin{align*}
    \partial \norm{\mb Z}{*} \;:=\; \Brac{ \mb D \in \bb R^{K \times N} \;\mid\; \norm{\mb G}{*} \geq \norm{\mb Z}{*} + \innerprod{ \mb G - \mb Z }{ \mb D },\; \mb G \in \bb R^{K \times N}  },
\end{align*}
where for nuclear norm, the previous work \cite{watson1992characterization,recht2010guaranteed} showed that based on the projection onto the column space and row space via the SVD of $\mb Z = \mb U \mb \Sigma \mb V^\top$, this is equivalent to  
\begin{align*}
   \partial \norm{\mb Z}{*} \;=\; \Brac{ \mb U \mb V^\top + \mb W, \mb W \in \bb R^{K \times N} \;\mid\; \mb U^\top \mb W = \mb 0,\; \mb W \mb V = \mb 0,\; \norm{\mb W}{}\leq 1 },
\end{align*}
where $\mb U$ and $\mb V$ are the left and right singular value matrices of $\mb Z$. Using the result above, we can now rewrite the optimality condition in \eqref{eq:KKT-convex} as suggested in Lemma \ref{lem:conv-global-cond}.
\end{proof}

\begin{lemma}[Optimality Condition for the Nonconvex Program \eqref{eq:obj-app}] \label{lem:global-optimality-nonconvex}
If a critical point $(\mW,\mH,\vb)$ of \eqref{eq:obj-app} satisfies
\begin{align}\label{eqn:global-cond-WH}
    \norm{ \nabla g(\mb W \mb H + \mb b \mb 1^\top) }{} \;\leq \; \sqrt{ \lambda_{\mb W} \lambda_{\mb H} },
\end{align}
then it is a global minimum of \eqref{eq:obj-app}.	

\end{lemma}

\begin{proof}[Proof of Lemma \ref{lem:global-optimality-nonconvex}] 
Suppose $(\mW^\star,\mH^\star,\vb^\star)$ is a critical point of \eqref{eq:obj-app} satisfying \eqref{eqn:global-cond-WH}, we will show that $(\mb Z^\star,\vb^\star)$ with $\mb Z^\star=\mW^\star\mH^\star$ is a global minimizer of \eqref{eq:convex-prob} by showing that $(\mb W^\star\mb H^\star,\vb^\star)$ satisfies the optimality condition for the convex program in \eqref{eq:KKT-convex-equivalence} (Lemma \ref{lem:conv-global-cond}). First of all, it is easy to check that
\begin{align*}
    \nabla_{\vb}f(\mW^\star,\mH^\star,\vb^\star) \;&=\;  \sum_{i=1}^N [\nabla g(\mW^\star\mH^\star + \vb^\star\vone^\top)]_i + \lambdab\vb^\star \;=\; \mb 0 \\
      \;&\Longrightarrow \; \sum_{i=1}^N [\nabla g(\mb Z^\star + \vb^\star\vone^\top)]_i + \lambdab\vb^\star\;=\; \vzero.
\end{align*}
Second, let $\mb Z^\star = \mW^\star\mH^\star = \mU\mSigma\mV^\top$ be the compact SVD of $\mb Z^\star= \mW^\star\mH^\star$. By Lemma \ref{lem:critical-balance}, we have
\begin{align*}
\mW^{\star\top}\mW^\star \;=\; \frac{\lambda_{\mH}}{\lambda_{\mW}}\mH^\star\mH^{\star\top}\;  \Longrightarrow\;  \mH^{\star\top} \mH^\star \mH^{\star\top} \mH^\star \;=\; \frac{\lambdaW}{\lambdaH} \mH^{\star\top}\mW^{\star\top}\mW^\star\mH^\star \;=\; \frac{\lambdaW}{\lambdaH} \mV\mSigma^2\mV^\top.
\end{align*}	
Now by utilizing Lemma \ref{lem:matrix-analysis-horn}, from the above equation we obtain the following
\begin{align*}
    \mb H^{\star\top} \mb H^\star \;=\; \sqrt{\frac{\lambdaW}{\lambdaH}} \mV\mSigma\mV^\top.
\end{align*}
This together with the first equation in \eqref{eqn:W-crtical} gives 
\begin{align*}
    \nabla g(\mW^\star\mH^\star + \vb^\star\vone^\top)\mH^{\star\top} \;=\; - \lambdaW \mW^\star\;\; &\Longrightarrow\;\; \nabla g(\mW^\star\mH^\star + \vb^\star\vone^\top)\mH^{\star\top}\mH^\star = - \lambdaW \mW^\star\mH^\star\\
    &\Longrightarrow \;\;\nabla g(\mW^\star\mH^\star + \vb\vone^\top)\sqrt{\frac{\lambdaW}{\lambdaH}} \mV\mSigma\mV^\top = - \lambdaW \mU\mSigma\mV^\top\\
    &\Longrightarrow \;\;  \nabla g(\mZ^\star + \vb^\star\vone^\top)\mV = - \sqrt{\lambdaW\lambdaH} \mU.
\end{align*}
Similarly, we can also get 
\begin{align*}
    \nabla g(\mZ^\star + \vb^\star\vone^\top)^\top\mU \;=\; - \sqrt{\lambdaW\lambdaH} \mV.
\end{align*}
 Thus, together with \eqref{eqn:global-cond-WH}, $(\mb Z^\star,\vb^\star)$ with $\mb Z^\star=\mb W^\star\mb H^\star$ satisfies the optimality condition \eqref{eq:KKT-convex-equivalence}, and hence is a global minimizer of $\wt{f}(\mb Z^\star,\mb b^\star)$ in \eqref{eq:convex-prob}. 
 
Finally, we complete the proof by invoking Lemma \ref{lem:equivalence}. By Lemma \ref{lem:equivalence} with $\mb Z^\star= \mb W^\star\mb H^\star$, we know that $f(\mb W^\star,\mb H^\star,\mb b^\star) = \wt{f}(\mb Z^\star,\mb b^\star) \leq f(\mb W,\mb H,\mb b)$ for all $\mW\in\R^{K\times d},\mH\in\R^{d\times N}, \vb\in\R^K$. Therefore, we must have $(\mb W^\star,\mb H^\star,\mb b^\star)$ to be the global solution of $f(\mb W,\mb H,\mb b)$ in \eqref{eq:obj-app}.
\end{proof}

%\eqref{eq:KKT-convex} and 

%By Lemma \ref{lem:equivalence}, we showed that $(\mW,\mH,\vb)$ is a global minimizer of \eqref{eq:obj-app} if $(\mb Z,\vb)$ with $\mb Z = \mb W \mb H$ is a global minimizer of the convex program \eqref{eq:convex-prob}.

%First note that any critical point $(\mW,\mH,\vb)$ of \eqref{eq:obj-app} satisfies \eqref{eq:critical-balance} (from Lemma \ref{lem:critical-balance}) and
%By assumption \eqref{eqn:global-cond-WH}, . To prove this,
